# Supplementary material for: Detailed Annotations of Chest X-Rays via CT Projection for Report Understanding
Source: arXiv:2210.03416 source file (2022-10-07)
Supplement: Supplementary file 1 [file supplementary.tex]

\section{Dataset: Additional Information}

\subsection{Visual Comparison between PAXRay and OpenI}
We show a more exploratory comparison between our projected (right columns) X-rays and samples of OpenI dataset (left columns) for frontal (top row) and lateral (bottom rows) views in Fig.~\ref{fig:syn_real}. Here, the position within frontal/lateral corresponds to the same position for the other view of the same patient. The differences in the frontal view stem from the overall difference in shoulder girdle positioning. While in the real images the arms are typically placed alongside the body, the arms are raised in the projected images due to the nature of the CT. In the lateral view, the real images display a larger variety in orientation and pose. Due to the projected images resulting from CTs usually taken while lying the pose between the different images is similar. This further results in visual differences between images of female patients between the two domains, e.g. 3rd column and second row of real, and first column and second row of projected for both frontal and lateral.

\setlength{\tabcolsep}{2pt}
\setlength{\abovecaptionskip}{6pt}
\setlength{\belowcaptionskip}{10pt}

\begin{figure}[h!]
    \centering
    \begin{tabular}{c ccc || ccc}
    \toprule
    & \multicolumn{3}{c}{OpenI (X-Ray)} & \multicolumn{3}{c}{PAXRay (Projected)} \\
    \midrule
    \multirow{3}{*}{\rotatebox{90}{Frontal}} & \includegraphics[width=0.15\linewidth,height=0.15\linewidth]{images/supplementary/real/CXR27_IM-1168-2002.png}& \includegraphics[width=0.15\linewidth,height=0.15\linewidth]{images/supplementary/real/CXR28_IM-1231-1001.png}& \includegraphics[width=0.15\linewidth,height=0.15\linewidth]{images/supplementary/real/CXR29_IM-1302-1001.png}& 
    \includegraphics[width=0.15\linewidth,height=0.15\linewidth]{images/supplementary/synthethic/RibFrac21frontal.png}& \includegraphics[width=0.15\linewidth,height=0.15\linewidth]{images/supplementary/synthethic/RibFrac22frontal.png}& \includegraphics[width=0.15\linewidth,height=0.15\linewidth]{images/supplementary/synthethic/RibFrac23frontal.png} \\
    & \includegraphics[width=0.15\linewidth,height=0.15\linewidth]{images/supplementary/real/CXR30_IM-1385-1001.png}& \includegraphics[width=0.15\linewidth,height=0.15\linewidth]{images/supplementary/real/CXR31_IM-1450-1001.png}& \includegraphics[width=0.15\linewidth,height=0.15\linewidth]{images/supplementary/real/CXR32_IM-1511-1001.png}& 
    \includegraphics[width=0.15\linewidth,height=0.15\linewidth]{images/supplementary/synthethic/RibFrac24frontal.png}& \includegraphics[width=0.15\linewidth,height=0.15\linewidth]{images/supplementary/synthethic/RibFrac25frontal.png}& \includegraphics[width=0.15\linewidth,height=0.15\linewidth]{images/supplementary/synthethic/RibFrac26frontal.png}\\
    & \includegraphics[width=0.15\linewidth,height=0.15\linewidth]{images/supplementary/real/CXR33_IM-1576-13013.png}& \includegraphics[width=0.15\linewidth,height=0.15\linewidth]{images/supplementary/real/CXR34_IM-1644-1001.png}& \includegraphics[width=0.15\linewidth,height=0.15\linewidth]{images/supplementary/real/CXR2_IM-0652-1001.png}& 
    \includegraphics[width=0.15\linewidth,height=0.15\linewidth]{images/supplementary/synthethic/RibFrac27frontal.png}& \includegraphics[width=0.15\linewidth,height=0.15\linewidth]{images/supplementary/synthethic/RibFrac28frontal.png}& \includegraphics[width=0.15\linewidth,height=0.15\linewidth]{images/supplementary/synthethic/RibFrac29frontal.png}\\\midrule\midrule
    \multirow{3}{*}{\rotatebox{90}{Lateral}}& \includegraphics[width=0.15\linewidth,height=0.15\linewidth]{images/supplementary/real/CXR27_IM-1168-3003.png}& \includegraphics[width=0.15\linewidth,height=0.15\linewidth]{images/supplementary/real/CXR29_IM-1302-2001.png}& \includegraphics[width=0.15\linewidth,height=0.15\linewidth]{images/supplementary/real/CXR28_IM-1231-2001.png}& 
    \includegraphics[width=0.15\linewidth,height=0.15\linewidth]{images/supplementary/synthethic/RibFrac21lateral.png}& \includegraphics[width=0.15\linewidth,height=0.15\linewidth]{images/supplementary/synthethic/RibFrac22lateral.png}& \includegraphics[width=0.15\linewidth,height=0.15\linewidth]{images/supplementary/synthethic/RibFrac23lateral.png} \\
    & \includegraphics[width=0.15\linewidth,height=0.15\linewidth]{images/supplementary/real/CXR30_IM-1385-2001.png}& \includegraphics[width=0.15\linewidth,height=0.15\linewidth]{images/supplementary/real/CXR31_IM-1450-3003.png}& \includegraphics[width=0.15\linewidth,height=0.15\linewidth]{images/supplementary/real/CXR32_IM-1511-4001.png}& 
    \includegraphics[width=0.15\linewidth,height=0.15\linewidth]{images/supplementary/synthethic/RibFrac24lateral.png}& \includegraphics[width=0.15\linewidth,height=0.15\linewidth]{images/supplementary/synthethic/RibFrac25lateral.png}& \includegraphics[width=0.15\linewidth,height=0.15\linewidth]{images/supplementary/synthethic/RibFrac26lateral.png}\\
    & \includegraphics[width=0.15\linewidth,height=0.15\linewidth]{images/supplementary/real/CXR33_IM-1576-12012.png}& \includegraphics[width=0.15\linewidth,height=0.15\linewidth]{images/supplementary/real/CXR34_IM-1644-2001.png}& \includegraphics[width=0.15\linewidth,height=0.15\linewidth]{images/supplementary/real/CXR2_IM-0652-2001.png}& 
    \includegraphics[width=0.15\linewidth,height=0.15\linewidth]{images/supplementary/synthethic/RibFrac27lateral.png}& \includegraphics[width=0.15\linewidth,height=0.15\linewidth]{images/supplementary/synthethic/RibFrac28lateral.png}& \includegraphics[width=0.15\linewidth,height=0.15\linewidth]{images/supplementary/synthethic/RibFrac29lateral.png}\\
    \bottomrule
    \end{tabular}
    \caption{Comparison of different real and projected samples for the frontal and lateral view}
    \label{fig:syn_real}
\end{figure}

\subsection{Further Visual Examples of Generated Labels}
We show additional examples for the annotations of our dataset in Fig.~\ref{fig:supplementary_dataset_examples}. We can see that lung halves can overlap in the second frontal row. While this might seem contradictory at first, when we consider the lung as a 3D-volume the classes can overlap along one dimension i.e. the lung halves in front and behind the heart as can be seen in Fig.~\ref{fig:3dslice_supp}. As we intend to capture the entire anatomy present in the upper body we consider this labeling assumption as a more holistic approach. 

\setlength{\tabcolsep}{2pt}

\begin{figure}[h]
    \centering
        \begin{tabular}{cccccc}
        \toprule
         & Input & Lungs & Mediastinum & Bones & Sub-Diaphragm  \\
         \midrule
         \multirow{3}{*}{\rotatebox{90}{Frontal}} & 
         \includegraphics[width=0.18\linewidth,height=0.18\linewidth]{images/supplementary_dataset_examples/9_frontal.jpg}&
         \includegraphics[width=0.18\linewidth,height=0.18\linewidth]{images/supplementary_dataset_examples/9_lung_frontal.jpg}&
         \includegraphics[width=0.18\linewidth,height=0.18\linewidth]{images/supplementary_dataset_examples/9_mediastinum_frontal.jpg}&
         \includegraphics[width=0.18\linewidth,height=0.18\linewidth]{images/supplementary_dataset_examples/9_bones_frontal.jpg}&
         \includegraphics[width=0.18\linewidth,height=0.18\linewidth]{images/supplementary_dataset_examples/9_diaphragm_frontal.jpg}\\
         & 
         \includegraphics[width=0.18\linewidth,height=0.18\linewidth]{images/supplementary_dataset_examples/12_frontal.jpg}&
         \includegraphics[width=0.18\linewidth,height=0.18\linewidth]{images/supplementary_dataset_examples/12_lung_frontal.jpg}&
         \includegraphics[width=0.18\linewidth,height=0.18\linewidth]{images/supplementary_dataset_examples/12_mediastinum_frontal.jpg}&
         \includegraphics[width=0.18\linewidth,height=0.18\linewidth]{images/supplementary_dataset_examples/12_bones_frontal.jpg}&
         \includegraphics[width=0.18\linewidth,height=0.18\linewidth]{images/supplementary_dataset_examples/12_diaphragm_frontal.jpg}\\
         \midrule
         \multirow{3}{*}{\rotatebox{90}{Lateral}} & 
         \includegraphics[width=0.18\linewidth,height=0.18\linewidth]{images/supplementary_dataset_examples/9_lateral.jpg}&
         \includegraphics[width=0.18\linewidth,height=0.18\linewidth]{images/supplementary_dataset_examples/9_lung_lateral.jpg}&
         \includegraphics[width=0.18\linewidth,height=0.18\linewidth]{images/supplementary_dataset_examples/9_mediastinum_lateral.jpg}&
         \includegraphics[width=0.18\linewidth,height=0.18\linewidth]{images/supplementary_dataset_examples/9_bones_lateral.jpg}&
         \includegraphics[width=0.18\linewidth,height=0.18\linewidth]{images/supplementary_dataset_examples/9_diaphragm_lateral.jpg}\\
         & 
         \includegraphics[width=0.18\linewidth,height=0.18\linewidth]{images/supplementary_dataset_examples/12_lateral.jpg}&
         \includegraphics[width=0.18\linewidth,height=0.18\linewidth]{images/supplementary_dataset_examples/12_lung_lateral.jpg}&
         \includegraphics[width=0.18\linewidth,height=0.18\linewidth]{images/supplementary_dataset_examples/12_mediastinum_lateral.jpg}&
         \includegraphics[width=0.18\linewidth,height=0.18\linewidth]{images/supplementary_dataset_examples/12_bones_lateral.jpg}&
         \includegraphics[width=0.18\linewidth,height=0.18\linewidth]{images/supplementary_dataset_examples/12_diaphragm_lateral.jpg}\\
         \bottomrule
    \end{tabular}
    \caption{Different ground truth annotations of our PAX-ray dataset for frontal and lateral view}
    \label{fig:supplementary_dataset_examples}
\end{figure}
\begin{figure}[h!]
    \centering
    \includegraphics[width=\linewidth, trim={0 3.5cm 0cm 7cm},clip]{images/supplementary_dataset_examples/ribfrac11.png}
    \caption{Example of a axial slice of a 3D Volume of the RibFrac dataset, where the two lung halves overlap along the sagittal plane}
    \label{fig:3dslice_supp}
\end{figure}

\newpage
\subsection{Complete Label Set}

\begin{minipage}{0.5\textwidth}

\begin{enumerate}

    \item  Lung
    \begin{enumerate}
        \item Right Lung
        \begin{enumerate}
            \item Right Lobe Upper
            \item Right Lobe Middle
            \item Right Lobe Lower
            \item Right Lung Vessel
        \end{enumerate}
        \item Left Lung
        \begin{enumerate}
            \item Left Lobe Upper
            \item Left Lobe Lower
            \item Left Lung Vessel
        \end{enumerate}
    \end{enumerate}
    % \item Diaphragm
    % \begin{enumerate}
    %     \item Left  Hemidiaphragm
    %     \item Right Hemidiaphragm
    % \end{enumerate}
\end{enumerate}
\end{minipage}
\begin{minipage}{0.5\textwidth}
\centering
    \includegraphics[width=0.7\textwidth]{images/supplementary/labels/3_lobes_frontal.jpg}
    \captionof{figure}{Lung Lobes}
\label{fig:figure}
\end{minipage}    

\begin{minipage}{0.5\textwidth}
\begin{enumerate}
\setcounter{enumi}{1}
    \item Mediastinum
    \begin{enumerate}
      
        \item Inferior Mediastinum
        \begin{enumerate}
            \item Anterior Mediastinum
            \item Middle Mediastinum
            \item Posterior Mediastinum
        \end{enumerate}
        \item Superior Mediastinum
        \item Heart
        \item Airways
        \item Esophagus
        \item Aorta
        \begin{enumerate}
            \item Ascending Aorta
            \item Aortic Arch
            \item Descending Aorta
        \end{enumerate}
    \end{enumerate}
\end{enumerate}
\end{minipage}
\begin{minipage}{0.5\textwidth}
\centering
    \begin{tabular}{c}
        
    \includegraphics[width=0.7\textwidth]{images/supplementary/labels/3_heart_frontal.jpg}\\
     \includegraphics[width=0.7\textwidth]{images/supplementary/labels/3_heart_lateral.jpg}
    \end{tabular}
    \captionof{figure}{Heart and Aorta}
\label{fig:figure}
\end{minipage} 

\begin{minipage}{0.5\textwidth}
\centering
    \begin{tabular}{c}
        
    \includegraphics[width=0.7\textwidth]{images/supplementary/labels/3_mediastinum_lateral.jpg}
    \end{tabular}
    \captionof{figure}{Mediastinum}
\label{fig:figure}
\end{minipage} 
\begin{minipage}{0.5\textwidth}
\centering
    \begin{tabular}{c}
        
    \includegraphics[width=0.7\textwidth]{images/supplementary/labels/3_vessels_frontal.jpg}
    \end{tabular}
    \captionof{figure}{Airways and Vessels}
\label{fig:figure}
\end{minipage} 

\begin{minipage}{0.5\textwidth}
\begin{enumerate}
    \setcounter{enumi}{2}
    \item Bones
    \begin{enumerate}
        \item Spine
        \begin{enumerate}
        \item Cervical Spine
        \begin{enumerate}
            \item C1
            \item C2
            \item C3
            \item C4
            \item C5
            \item C6
            \item C7
        \end{enumerate}
        \end{enumerate}
    \end{enumerate}
\end{enumerate}
\end{minipage}
\begin{minipage}{0.5\textwidth}
\centering
    \begin{tabular}{c}
        
    \includegraphics[width=0.7\textwidth]{images/supplementary/labels/3_cervical_frontal.jpg}\\
    \includegraphics[width=0.7\textwidth]{images/supplementary/labels/3_cervical_lateral.jpg}
    \end{tabular}
    \captionof{figure}{Cervical Spine}
\label{fig:figure}
\end{minipage} 

\begin{minipage}{0.5\textwidth}
\begin{enumerate}
    \begin{enumerate}
        \begin{enumerate}
            \item Thoracic Spine
        \begin{enumerate}
            \item T1
            \item T2
            \item T3
            \item T4
            \item T5
            \item T6
            \item T7
            \item T8
            \item T9
            \item T10
            \item T11
            \item T12
            \item T13
        \end{enumerate}
        \end{enumerate}
    \end{enumerate}
\end{enumerate}
\end{minipage}
\begin{minipage}{0.5\textwidth}
\centering
    \begin{tabular}{c}
        
    \includegraphics[width=0.7\textwidth]{images/supplementary/labels/3_thoracic_frontal.jpg}\\
    \includegraphics[width=0.7\textwidth]{images/supplementary/labels/3_thoracic_lateral.jpg}
    \end{tabular}
    \captionof{figure}{Thoracic Spine}
\label{fig:figure}
\end{minipage} 

\begin{minipage}{0.5\textwidth}
\begin{enumerate}
    \begin{enumerate}
        \begin{enumerate}
            \item Lumbar Spine
            \begin{enumerate}
                \item L1
                \item L2
                \item L3
                \item L4
                \item L5
            \end{enumerate}
            \item Sacrum
            \item Cocygis
        \end{enumerate}
    \end{enumerate}
\end{enumerate}
\end{minipage}
\begin{minipage}{0.5\textwidth}
\centering
    \begin{tabular}{c}
        
    \includegraphics[width=0.7\textwidth]{images/supplementary/labels/3_lumbar_frontal.jpg}\\
    \includegraphics[width=0.7\textwidth]{images/supplementary/labels/3_lumbar_lateral.jpg}
    \end{tabular}
    \captionof{figure}{Lumbar Spine}
\label{fig:figure}
\end{minipage} 

\begin{minipage}{0.5\textwidth}
\begin{enumerate}
\begin{enumerate}
    \item Ribs
        \begin{enumerate}
            \item 1st Rib
            \begin{enumerate}
                \item 1st Rib Posterior
                \item 1st Rib Anterior
                \item Left 1st Rib
                \begin{enumerate}
                    \item Left 1st Rib Posterior
                    \item Left 1st Rib Anterior
                \end{enumerate}
                \item Right 1st Rib
                \begin{enumerate}
                    \item Right 1st Rib Posterior
                    \item Right 1st Rib Anterior
                \end{enumerate}
            \end{enumerate}
            \item 2nd Rib
            
            \begin{enumerate}
            \item 2nd Rib Posterior
            \item 2nd Rib Anterior
                \item Left 2nd Rib
                \begin{enumerate}
                    \item Left 2nd Rib Posterior
                    \item Left 2nd Rib Anterior
                \end{enumerate}
                \item Right 2nd Rib
                \begin{enumerate}
                    \item Right 2nd Rib Posterior
                    \item Right 2nd Rib Anterior
                \end{enumerate}
            \end{enumerate}
            
        \end{enumerate}
\end{enumerate}
\end{enumerate}
\end{minipage}
\begin{minipage}{0.5\textwidth}
\centering
    \begin{tabular}{c}
        
    \includegraphics[width=0.7\textwidth]{images/supplementary/labels/3_ribs_frontal.jpg}\\
    \includegraphics[width=0.7\textwidth]{images/supplementary/labels/3_rib_lateral.jpg}
    \end{tabular}
    \captionof{figure}{6th Rib}
\label{fig:figure}
\end{minipage} 

\hspace{-30pt}
\begin{minipage}{0.5\textwidth}
 \begin{enumerate}
     \begin{enumerate}
         \begin{enumerate}
            \item 3rd Rib
            \begin{enumerate}
                \item 3rd Rib Posterior
                \item 3rd Rib Anterior
                \item Left 3rd Rib
                \begin{enumerate}
                    \item Left 3rd Rib Posterior
                    \item Left 3rd Rib Anterior
                \end{enumerate}
                \item Right 3rd Rib
                \begin{enumerate}
                    \item Right 3rd Rib Posterior
                    \item Right 3rd Rib Anterior
                \end{enumerate}
            \end{enumerate}
             \item 4th Rib
            
            \begin{enumerate}
            \item 4th Rib Posterior
            \item 4th Rib Anterior
                \item Left 4th Rib
                \begin{enumerate}
                    \item Left 4th Rib Posterior
                    \item Left 4th Rib Anterior
                \end{enumerate}
                \item Right 4th Rib
                \begin{enumerate}
                    \item Right 4th Rib Posterior
                    \item Right 4th Rib Anterior
                \end{enumerate}
            \end{enumerate}
            \item 5th Rib
            
            \begin{enumerate}
            \item 5th Rib Posterior
            \item 5th Rib Anterior
                \item Left 5th Rib
                \begin{enumerate}
                    \item Left 5th Rib Posterior
                    \item Left 5th Rib Anterior
                \end{enumerate}
                \item Right 5th Rib
                \begin{enumerate}
                    \item Right 5th Rib Posterior
                    \item Right 5th Rib Anterior
                \end{enumerate}
            \end{enumerate}
            \item 6th Rib
            
            \begin{enumerate}
            \item 6th Rib Posterior
            \item 6th Rib Anterior
                \item Left 6th Rib
                \begin{enumerate}
                    \item Left 6th Rib Posterior
                    \item Left 6th Rib Anterior
                \end{enumerate}
                \item Right 6th Rib
                \begin{enumerate}
                    \item Right 6th Rib Posterior
                    \item Right 6th Rib Anterior
                \end{enumerate}
            \end{enumerate}
            \item 7th Rib
           
            \begin{enumerate}
             \item 7th Rib Posterior
            \item 7th Rib Anterior
                \item Left 7th Rib
                \begin{enumerate}
                    \item Left 7th Rib Posterior
                    \item Left 7th Rib Anterior
                \end{enumerate}
                \item Right 7th Rib
                \begin{enumerate}
                    \item Right 7th Rib Posterior
                    \item Right 7th Rib Anterior
                \end{enumerate}
            \end{enumerate}
         \end{enumerate}
     \end{enumerate}
 \end{enumerate}
\end{minipage}
\begin{minipage}{0.5\textwidth}
\begin{enumerate}
 \begin{enumerate}
     \begin{enumerate}
            \item 8th Rib
            
            \begin{enumerate}
            \item 8th Rib Posterior
            \item 8th Rib Anterior
                \item Left 8th Rib
                \begin{enumerate}
                    \item Left 8th Rib Posterior
                    \item Left 8th Rib Anterior
                \end{enumerate}
                \item Right 8th Rib
                \begin{enumerate}
                    \item Right 8th Rib Posterior
                    \item Right 8th Rib Anterior
                \end{enumerate}
            \end{enumerate}
            \item 9th Rib
            
            \begin{enumerate}
            \item 9th Rib Posterior
            \item 9th Rib Anterior
                \item Left 9th Rib
                \begin{enumerate}
                    \item Left 9th Rib Posterior
                    \item Left 9th Rib Anterior
                \end{enumerate}
                \item Right 9th Rib
                \begin{enumerate}
                    \item Right 9th Rib Posterior
                    \item Right 9th Rib Anterior
                \end{enumerate}
            \end{enumerate}
            \item 10th Rib
            
            \begin{enumerate}
            \item 10th Rib Posterior
            \item 10th Rib Anterior
                \item Left 10th Rib
                \begin{enumerate}
                    \item Left 10th Rib Posterior
                    \item Left 10th Rib Anterior
                \end{enumerate}
                \item Right 10th Rib
                \begin{enumerate}
                    \item Right 10th Rib Posterior
                    \item Right 10th Rib Anterior
                \end{enumerate}
            \end{enumerate}
            \item 11th Rib
           
            \begin{enumerate}
             \item 1st Rib Posterior
            \item 1st Rib Anterior
                \item Left 11th Rib
                \begin{enumerate}
                    \item Left 11th Rib Posterior
                    \item Left 11th Rib Anterior
                \end{enumerate}
                \item Right 11th Rib
                \begin{enumerate}
                    \item Right 11th Rib Posterior
                    \item Right 11th Rib Anterior
                \end{enumerate}
            \end{enumerate}
            \item 12th Rib
            
            \begin{enumerate}
            \item 12th Rib Posterior
            \item 12th Rib Anterior
                \item Left 12th Rib
                \begin{enumerate}
                    \item Left 12th Rib Posterior
                    \item Left 12rd Rib Anterior
                \end{enumerate}
                \item Right 12th Rib
                \begin{enumerate}
                    \item Right 12th Rib Posterior
                    \item Right 12th Rib Anterior
                \end{enumerate}
            \end{enumerate}
     \end{enumerate}
 \end{enumerate}
\end{enumerate}
\end{minipage}

\begin{enumerate}
\setcounter{enumi}{3}
    \item Diaphragm
    \begin{enumerate}
        \item Hemidiaphragm Left
        \item Hemidiaphragm Right
    \end{enumerate}
\end{enumerate}

\section{Additional Segmentation Results}

\setlength{\tabcolsep}{2pt}

\begin{figure*}[t]
    \centering
        \begin{tabular}{cccccc}
        \toprule
         & Input & Lungs & Mediastinum & Bones & Sub-Diaphragm  \\
         \midrule
         \multirow{3}{*}{\rotatebox{90}{Frontal}} & 
         \includegraphics[width=0.17\linewidth,height=0.17\linewidth]{images/supplementary_label_examples/15_frontal.png}&
         \includegraphics[width=0.17\linewidth,height=0.17\linewidth]{images/supplementary_label_examples/15_frontal_lung.png}&
         \includegraphics[width=0.17\linewidth,height=0.17\linewidth]{images/supplementary_label_examples/15_frontal_mediastinum.png}&
         \includegraphics[width=0.17\linewidth,height=0.17\linewidth]{images/supplementary_label_examples/15_frontal_bones.png}&
         \includegraphics[width=0.17\linewidth,height=0.17\linewidth]{images/supplementary_label_examples/15_frontal_diaphragm.png}\\
         & 
         \includegraphics[width=0.17\linewidth,height=0.17\linewidth]{images/supplementary_label_examples/14_frontal.png}&
         \includegraphics[width=0.17\linewidth,height=0.17\linewidth]{images/supplementary_label_examples/14_frontal_lung.png}&
         \includegraphics[width=0.17\linewidth,height=0.17\linewidth]{images/supplementary_label_examples/14_frontal_mediastinum.png}&
         \includegraphics[width=0.17\linewidth,height=0.17\linewidth]{images/supplementary_label_examples/14_frontal_bones.png}&
         \includegraphics[width=0.17\linewidth,height=0.17\linewidth]{images/supplementary_label_examples/14_frontal_diaphragm.png}\\
         \midrule
         \multirow{3}{*}{\rotatebox{90}{Lateral}} & 
         \includegraphics[width=0.17\linewidth,height=0.17\linewidth]{images/supplementary_label_examples/15_lateral.png}&
         \includegraphics[width=0.17\linewidth,height=0.17\linewidth]{images/supplementary_label_examples/15_lateral_lung.png}&
         \includegraphics[width=0.17\linewidth,height=0.17\linewidth]{images/supplementary_label_examples/15_lateral_mediastinum.png}&
         \includegraphics[width=0.17\linewidth,height=0.17\linewidth]{images/supplementary_label_examples/15_lateral_bones.png}&
         \includegraphics[width=0.17\linewidth,height=0.17\linewidth]{images/supplementary_label_examples/15_lateral_diaphragm.png}\\

         & 
         \includegraphics[width=0.17\linewidth,height=0.17\linewidth]{images/supplementary_label_examples/14_lateral.png}&
         \includegraphics[width=0.17\linewidth,height=0.17\linewidth]{images/supplementary_label_examples/14_lateral_lung.png}&
         \includegraphics[width=0.17\linewidth,height=0.17\linewidth]{images/supplementary_label_examples/14_lateral_mediastinum.png}&
         \includegraphics[width=0.17\linewidth,height=0.17\linewidth]{images/supplementary_label_examples/14_lateral_bones.png}&
         \includegraphics[width=0.17\linewidth,height=0.17\linewidth]{images/supplementary_label_examples/14_lateral_diaphragm.png}\\
         \bottomrule
    \end{tabular}
    \caption{Qualitative results of a UNet with ResNet50 backbone trained on our PAX-ray dataset for multiple patients in OpenI.}
    \label{fig:supplementary_label_examples}
\end{figure*}
\subsection{3D Segmentation Results}
In this section, we show the training performance of nnUNet~\cite{isensee2021nnu} across the considered datasets. The training and validation losses as well as the validation  performance for all splits of all datasets are  displayed in Fig.~\ref{fig:training}.
For SegThor, the final validation performance ranges between 0.91 and 0.93 across all splits. For Verse, the final validation performance ranges between 0.82 and 0.84 across all splits. 
Hofmanninger's~\etal~\cite{hofmanninger2020automatic} report a dice score for their lung segmentation model of 0.99, 0.94, and 0.98 on the LTRC~\cite{ltrc}, LCTSC~\cite{yang2017data}, and  VESS12~\cite{rudyanto2014comparing} datasets respectively. Koitka~\etal~\cite{koitka2021fully} show a performance for their BCA of 0.96 dice on their internal dataset.

\setlength{\tabcolsep}{-7pt}

\begin{figure*}
    \centering
    \begin{tabular}{ccc}
    \toprule
    & SegThor & Verse\\\midrule
    
    \rotatebox{90}{$\;\;\;\;\;\;\;\;\;\;$ Split 0}
    
    & \includegraphics[ width=0.45\linewidth,height=0.27\linewidth,trim={1cm 0.5cm 0.25cm 1cm},clip,]{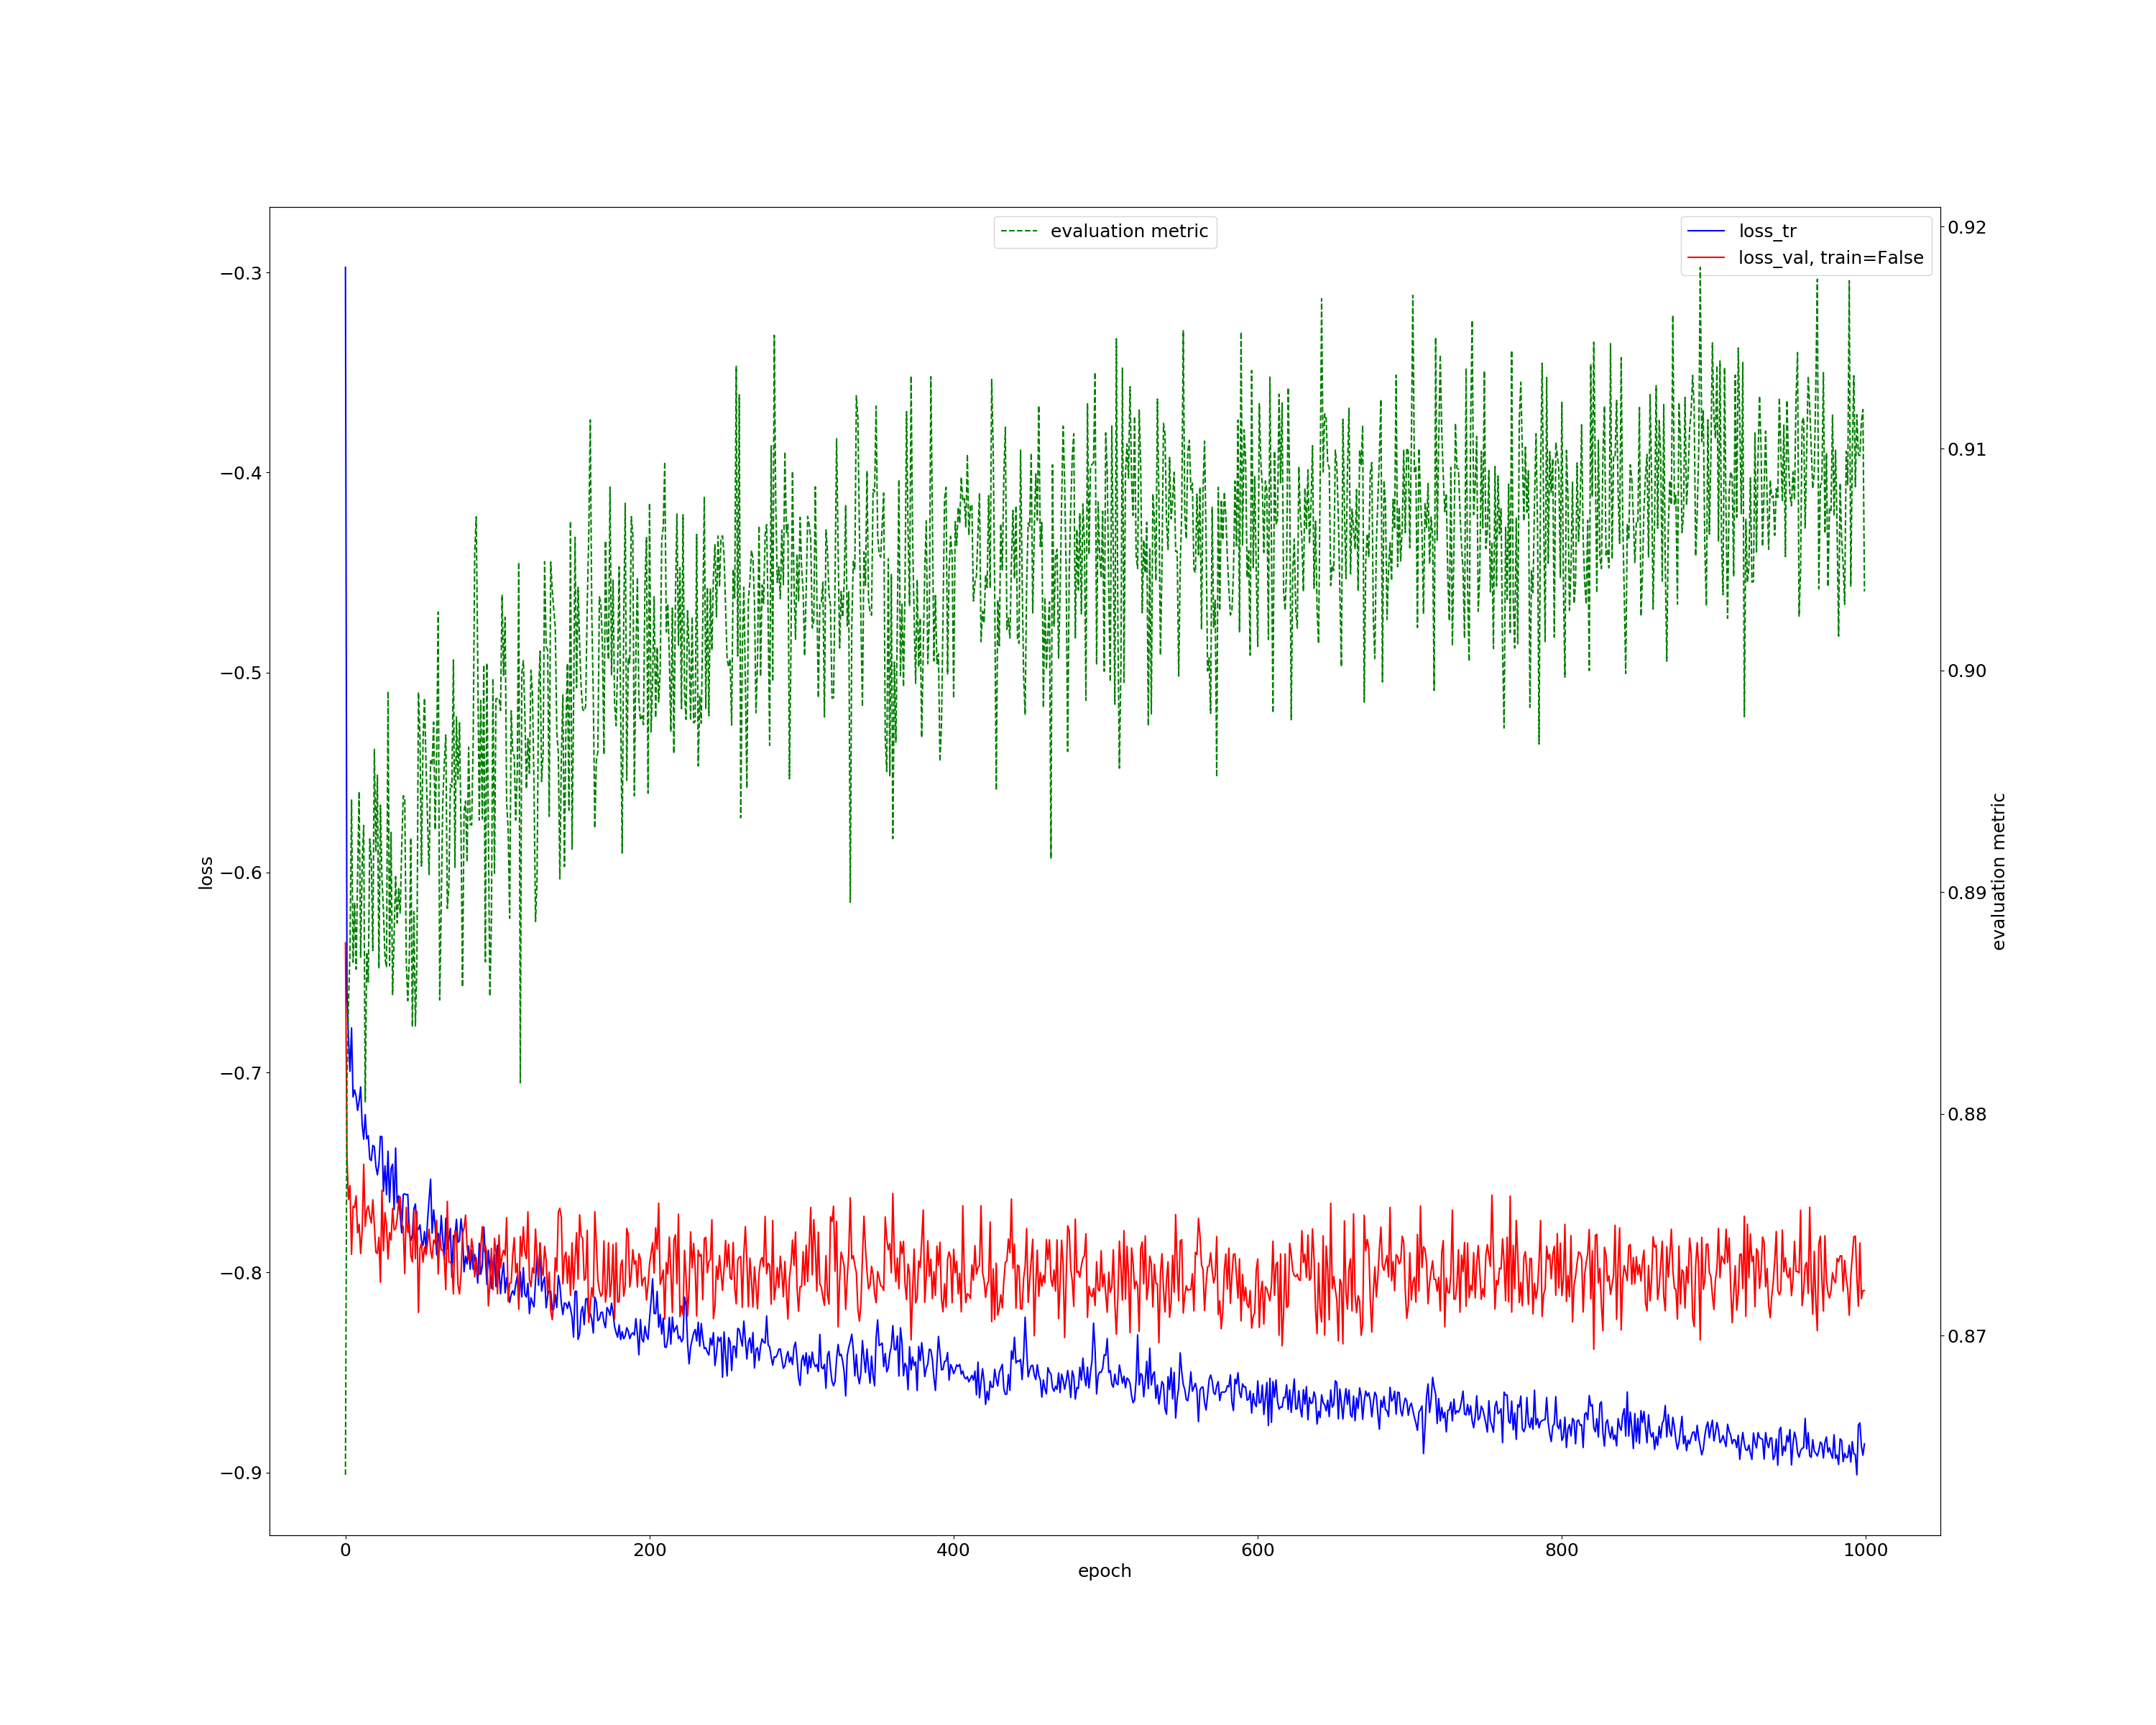}
    & \includegraphics[ width=0.45\linewidth,height=0.27\linewidth,trim={1cm 0.5cm 0.25cm 1cm},clip,]{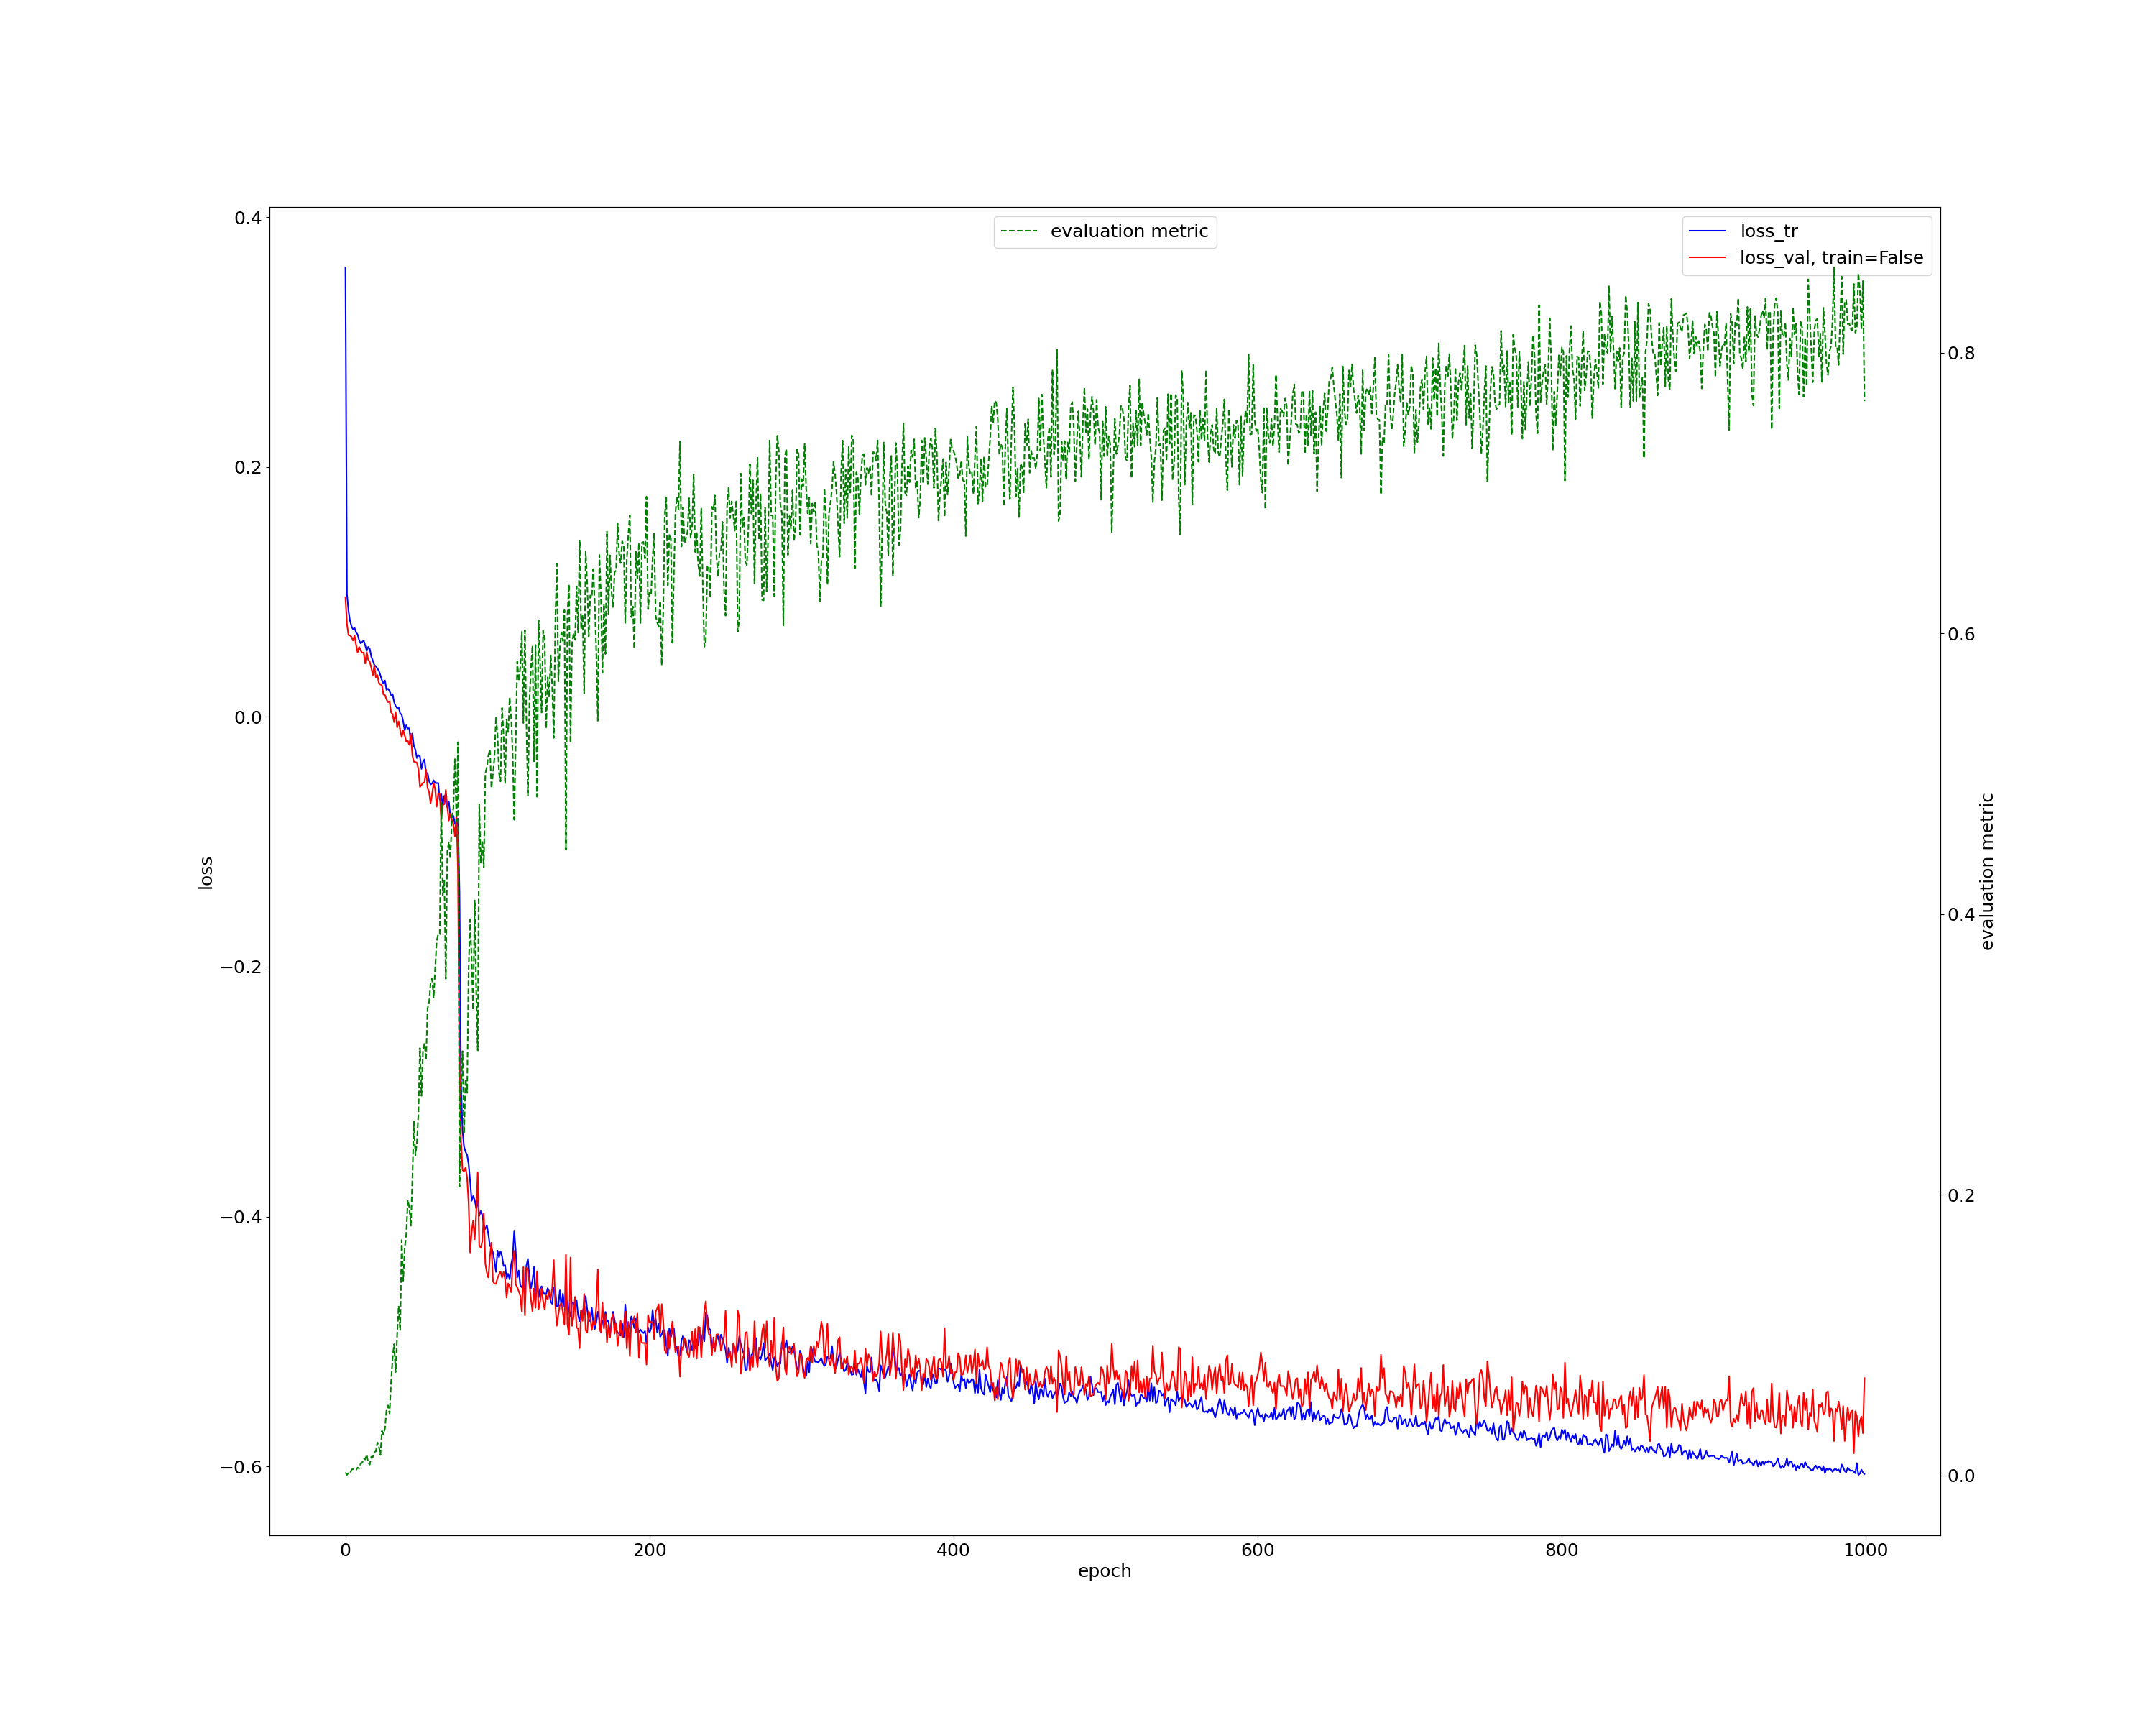}
    
    \\
    
    \rotatebox{90}{$\;\;\;\;\;\;\;\;\;\;$ Split 1}
    & \includegraphics[ width=0.45\linewidth,height=0.27\linewidth,trim={1cm 0.5cm 0.25cm 1cm},clip,]{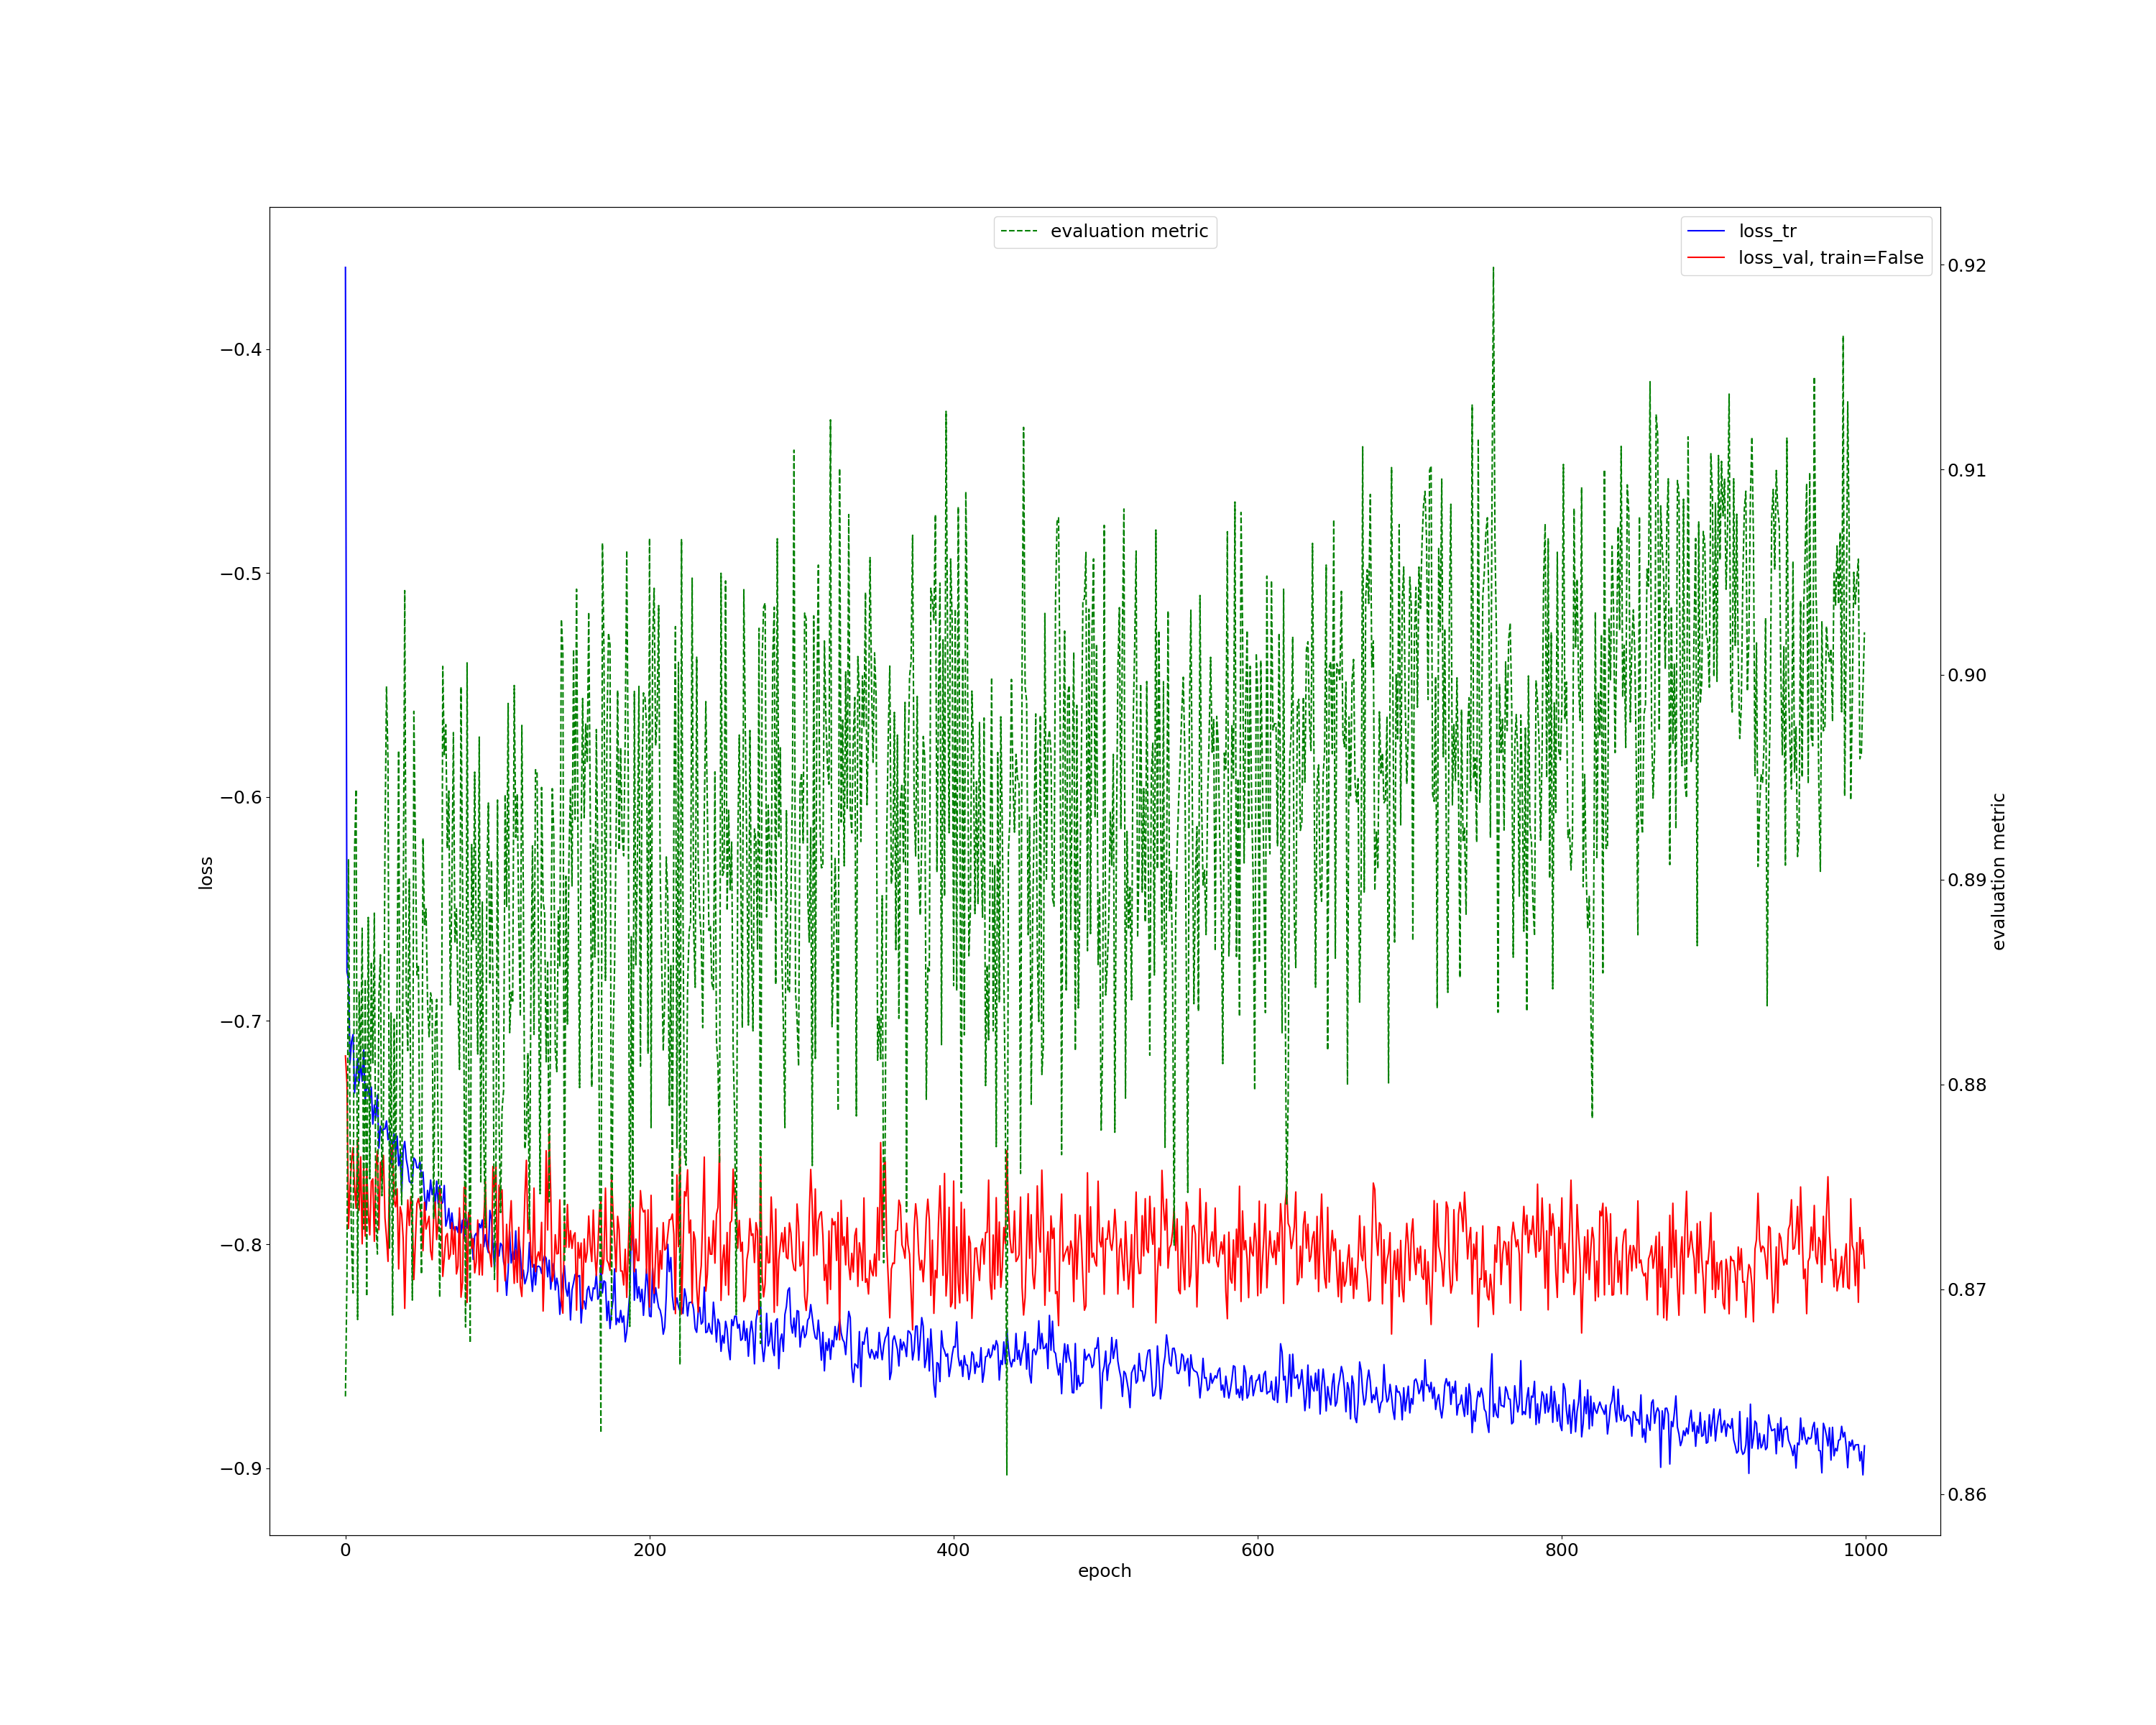}
& \includegraphics[ width=0.45\linewidth,height=0.27\linewidth,trim={1cm 0.5cm 0.25cm 1cm},clip,]{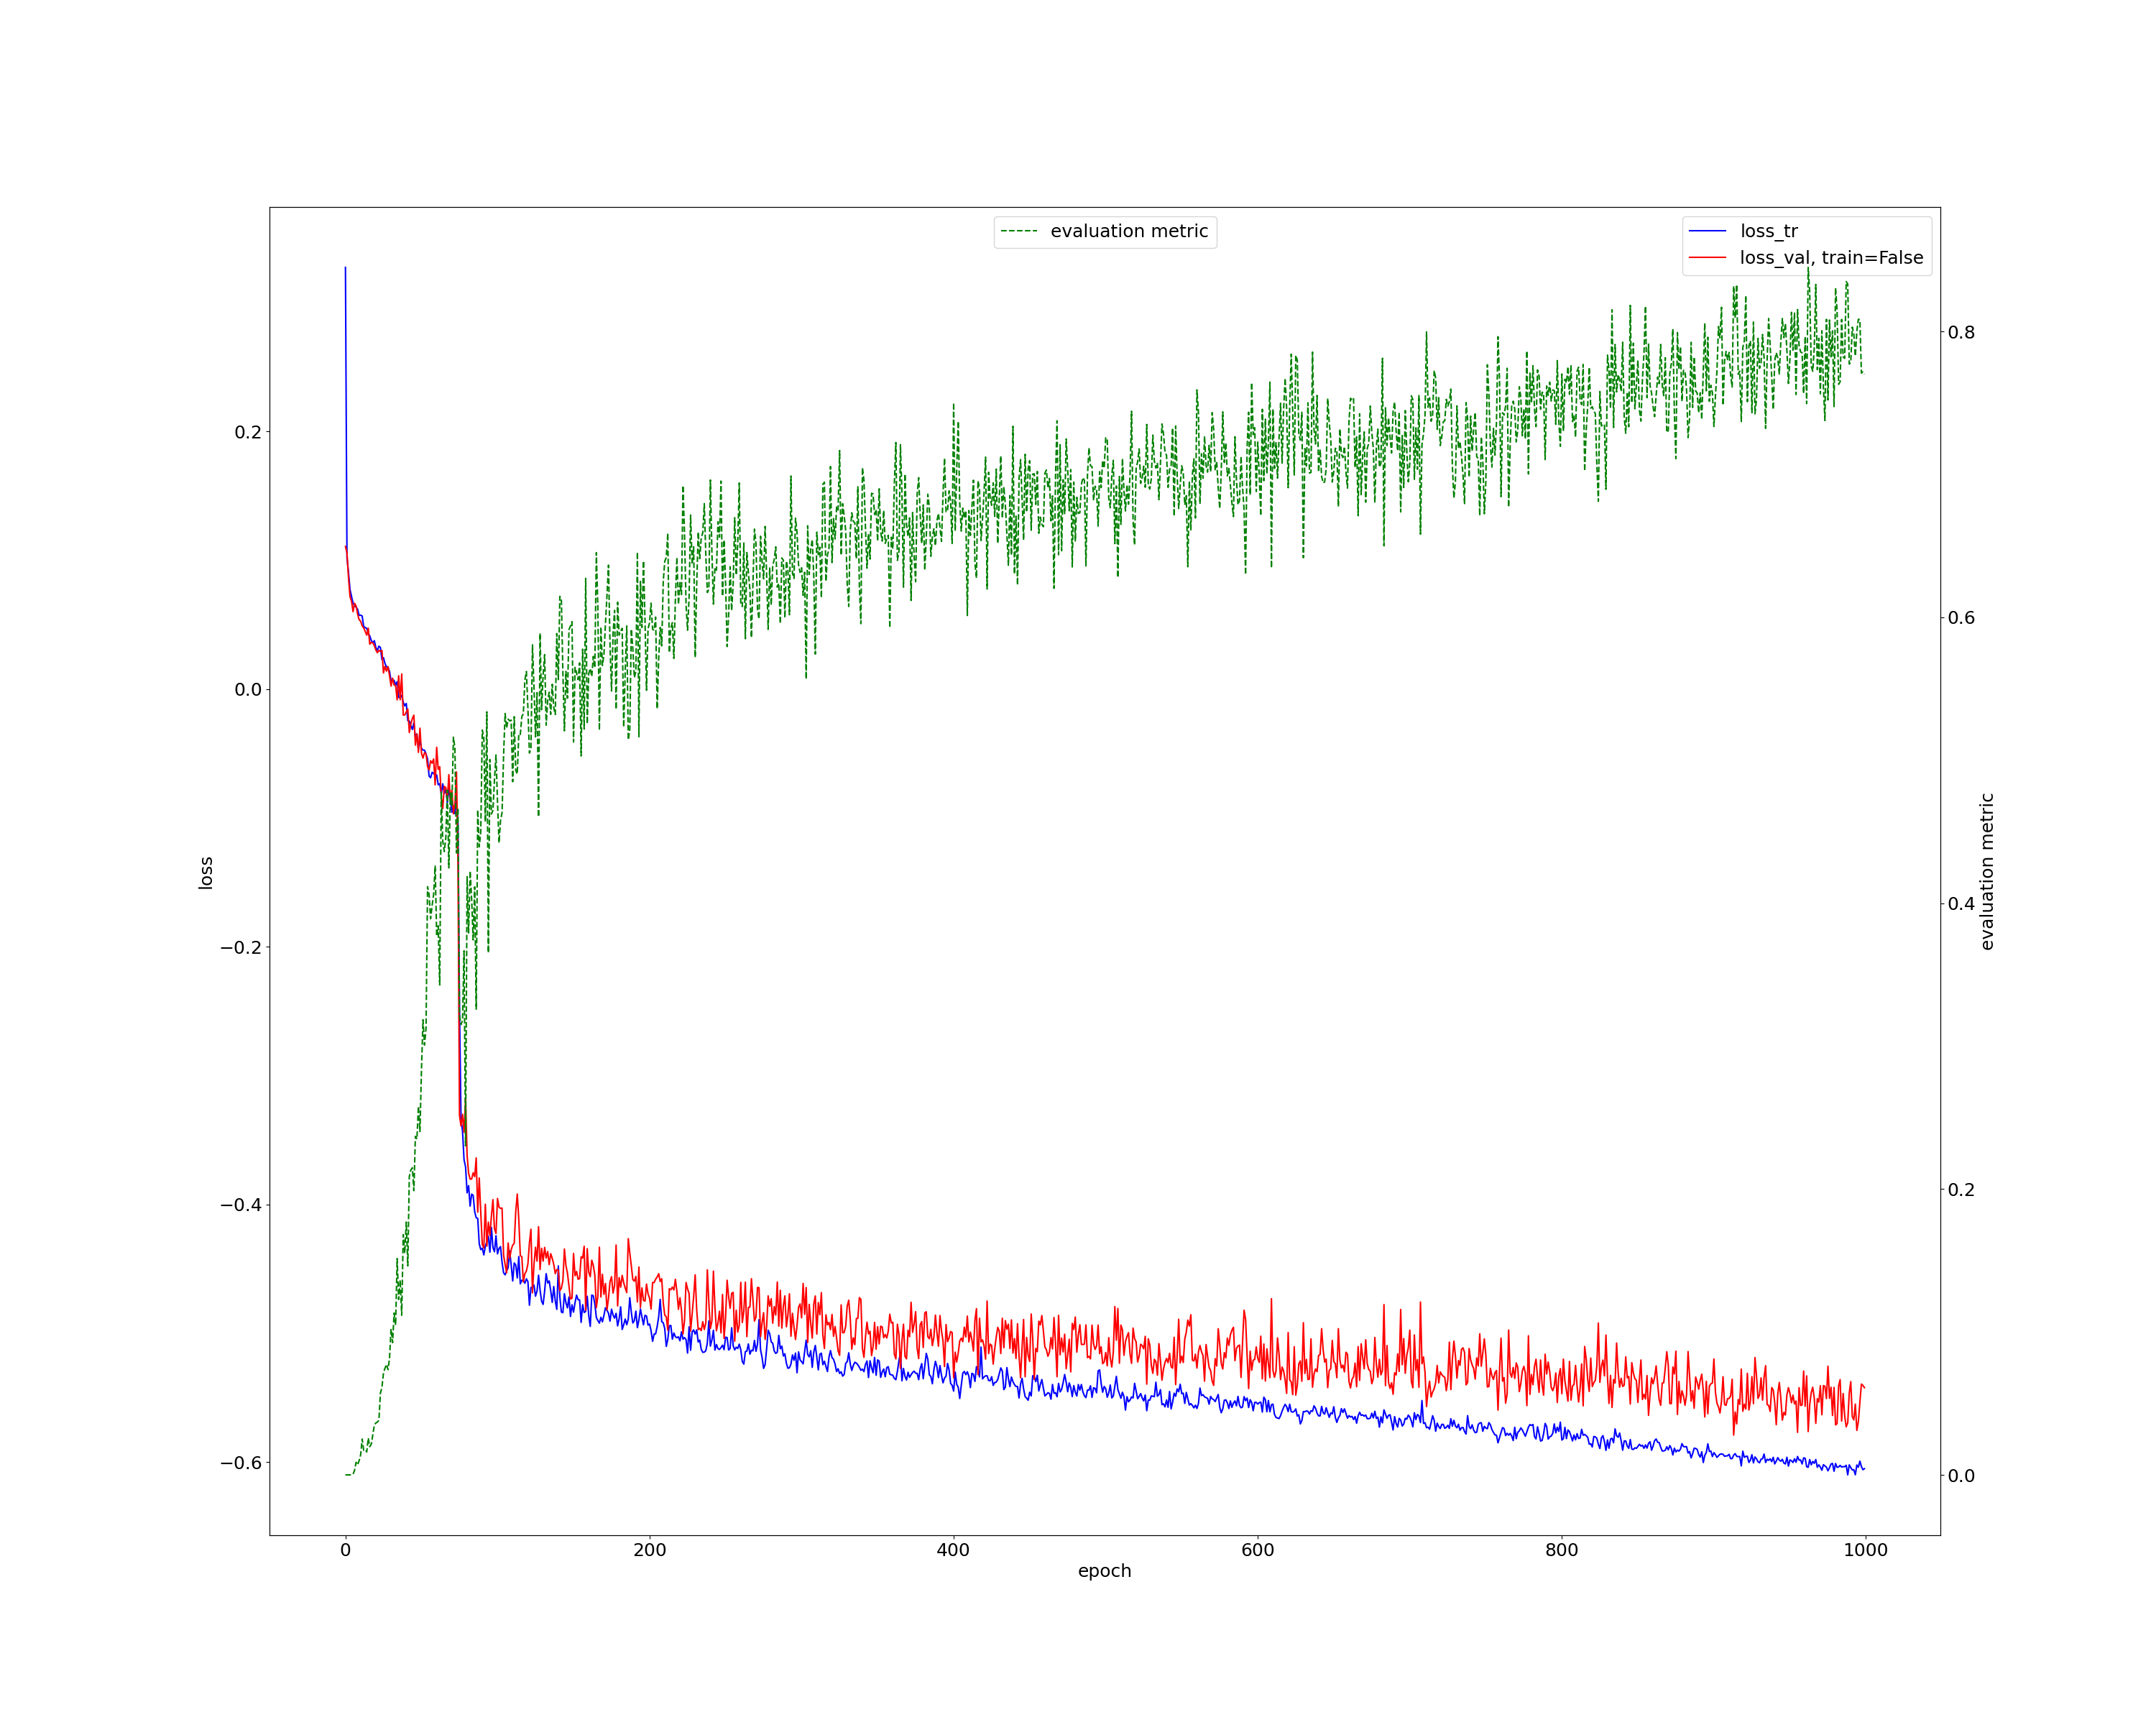}
 \\

    \rotatebox{90}{$\;\;\;\;\;\;\;\;\;\;$ Split 2}
    & \includegraphics[ width=0.45\linewidth,height=0.27\linewidth,trim={1cm 0.5cm 0.25cm 1cm},clip,]{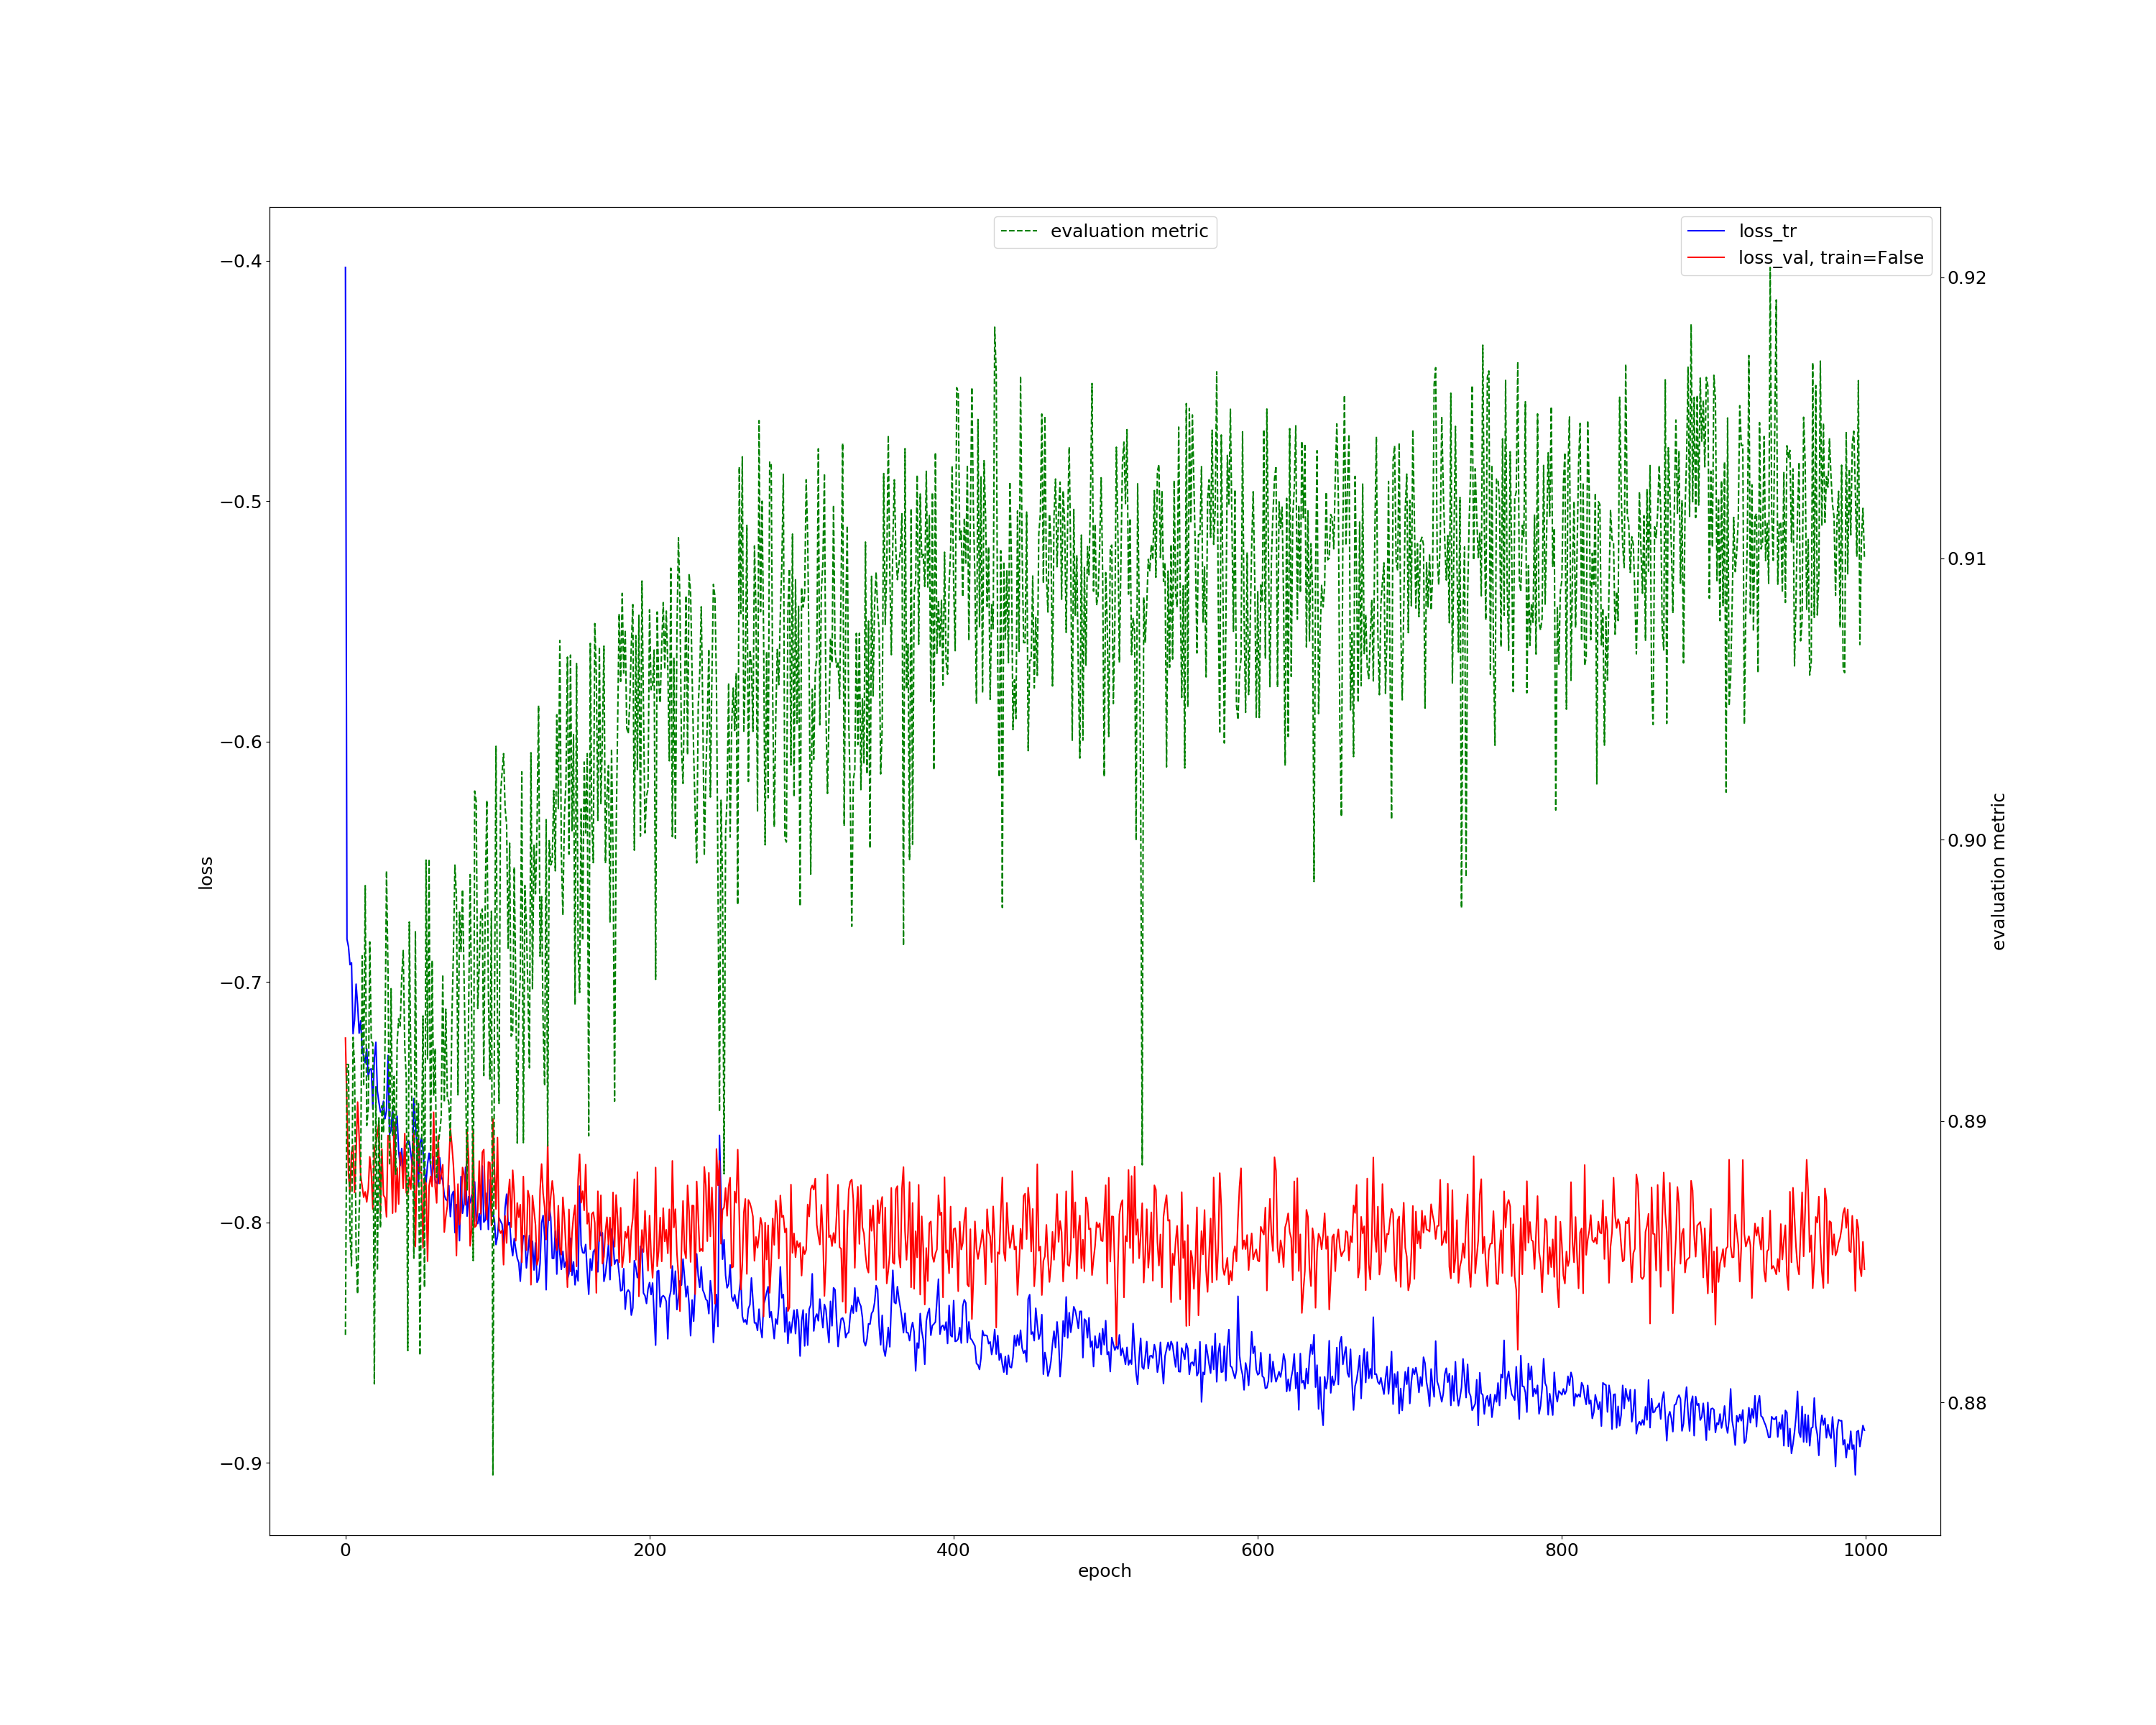}
& \includegraphics[ width=0.45\linewidth,height=0.27\linewidth,trim={1cm 0.5cm 0.25cm 1cm},clip,]{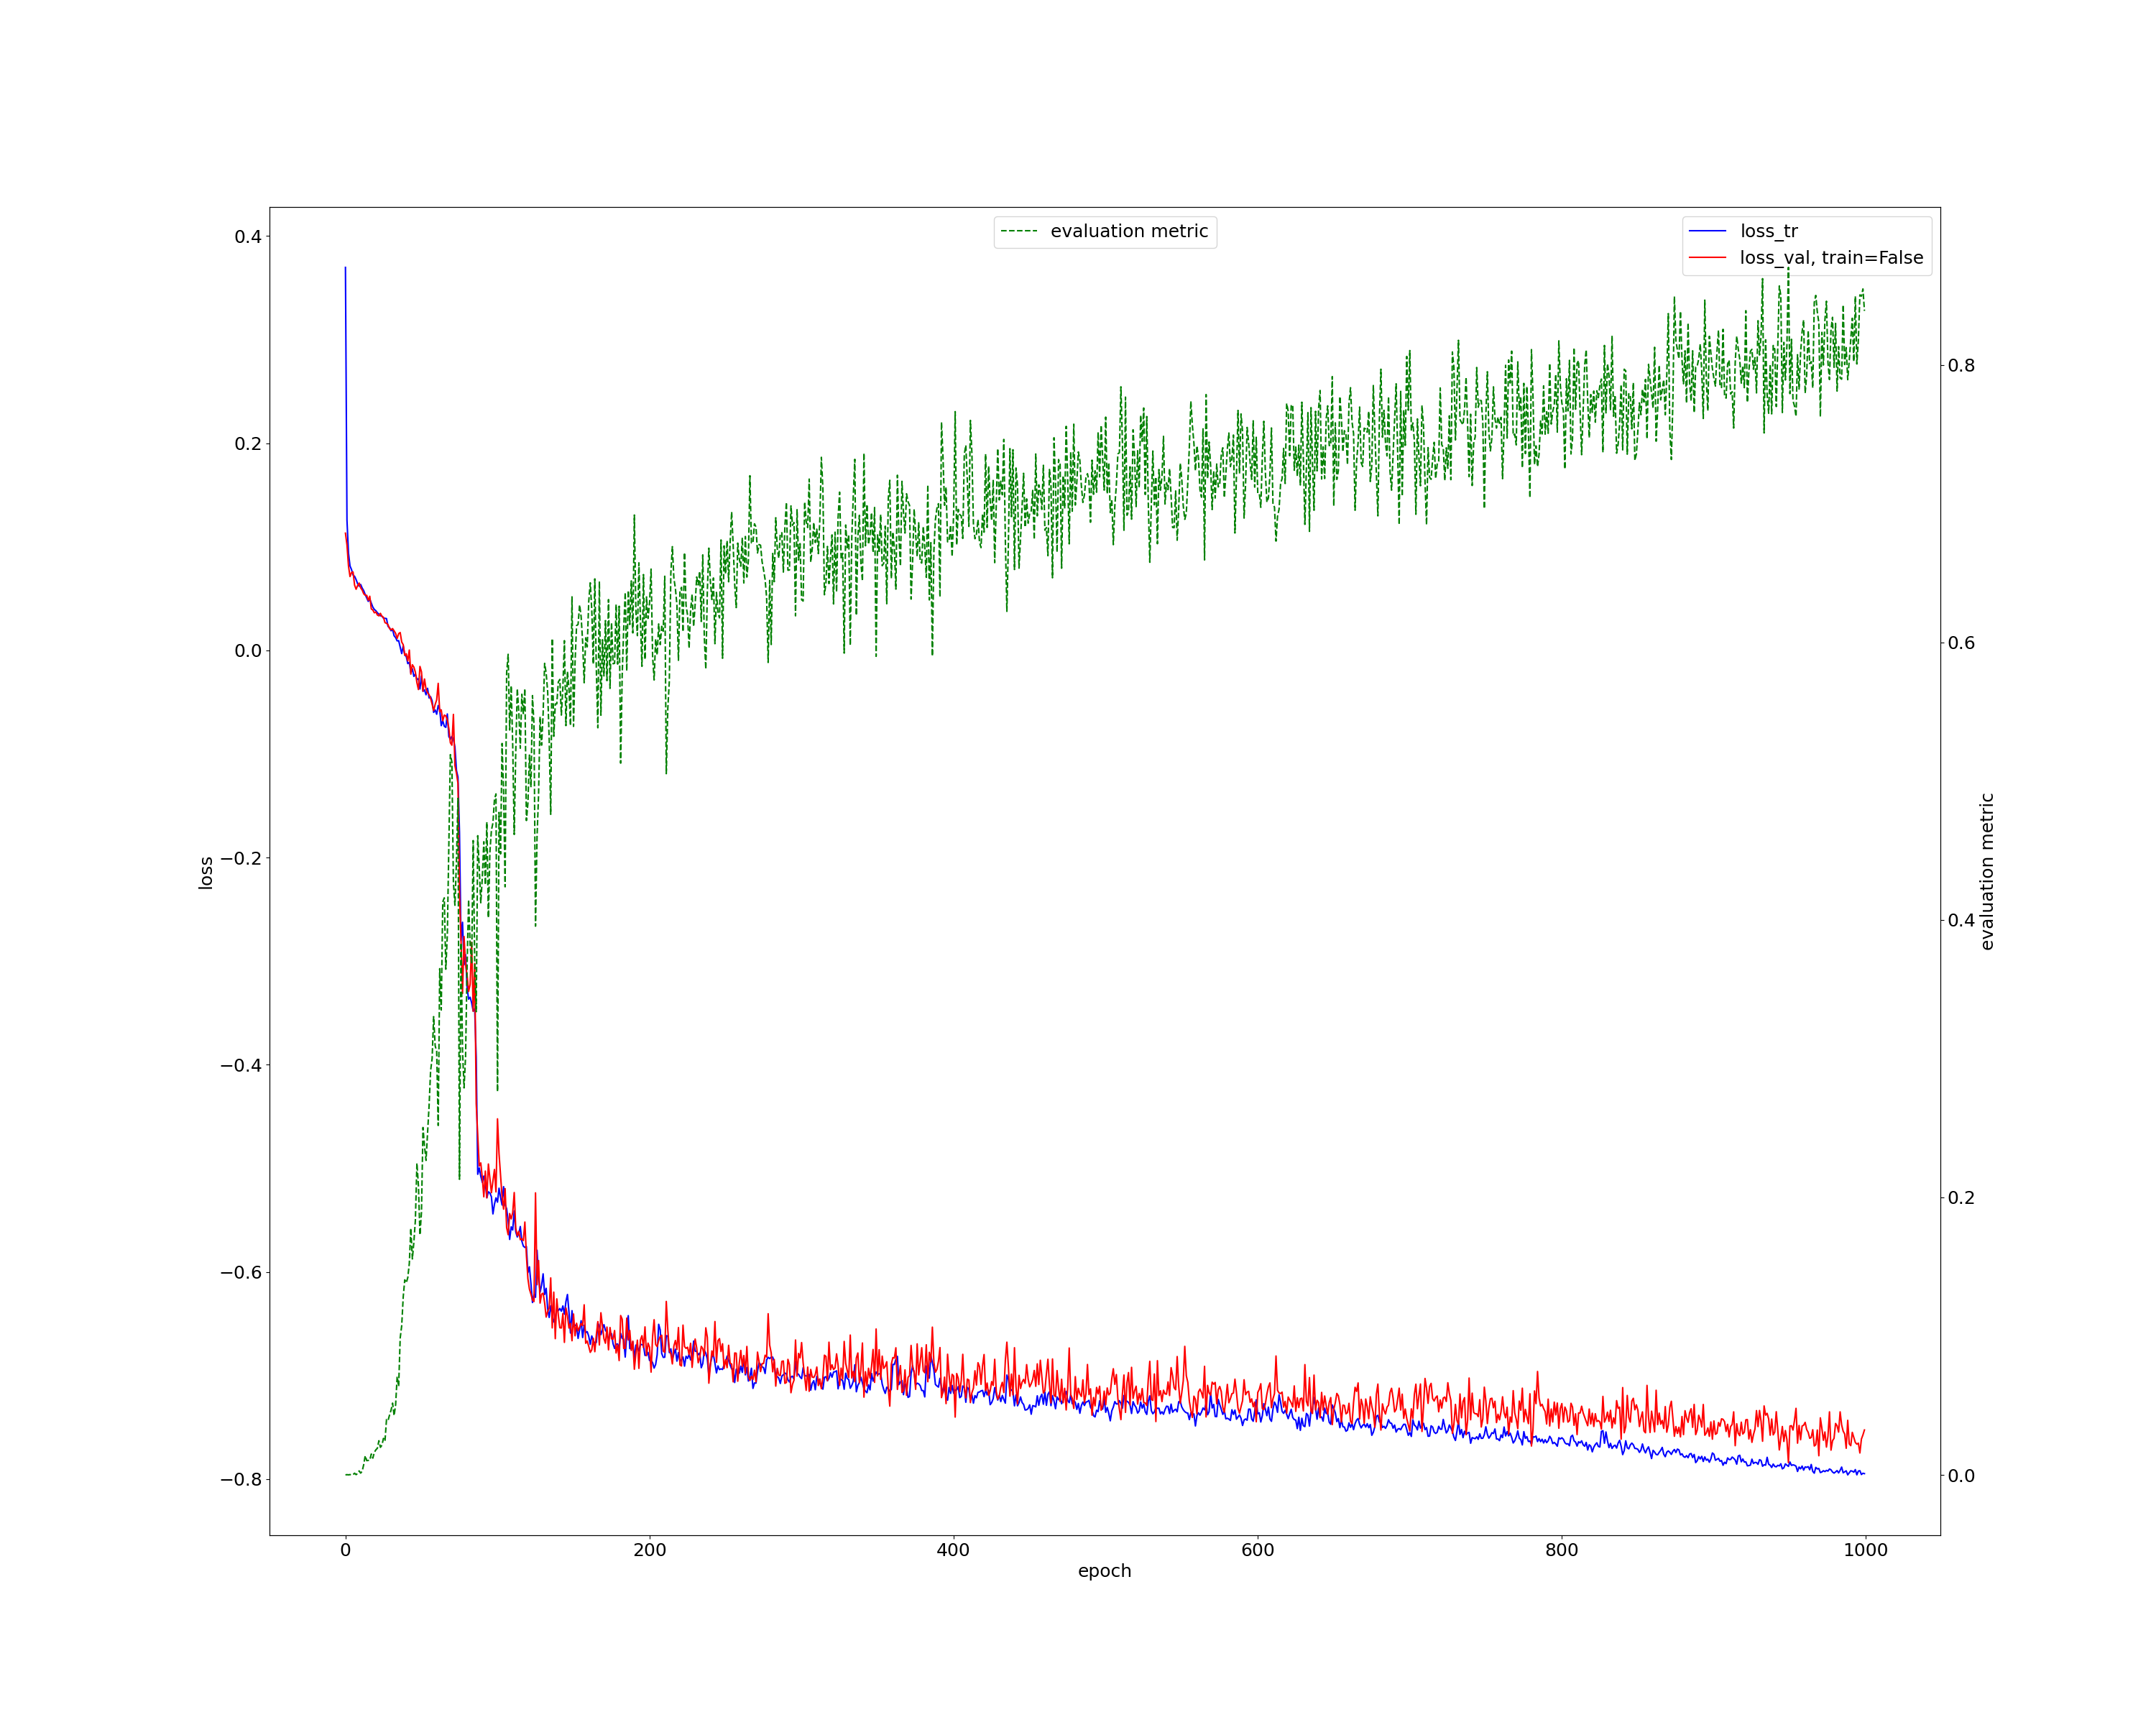}

 \\

    \rotatebox{90}{$\;\;\;\;\;\;\;\;\;\;$ Split 3}
    & \includegraphics[ width=0.45\linewidth,height=0.27\linewidth,trim={1cm 0.5cm 0.25cm 1cm},clip,]{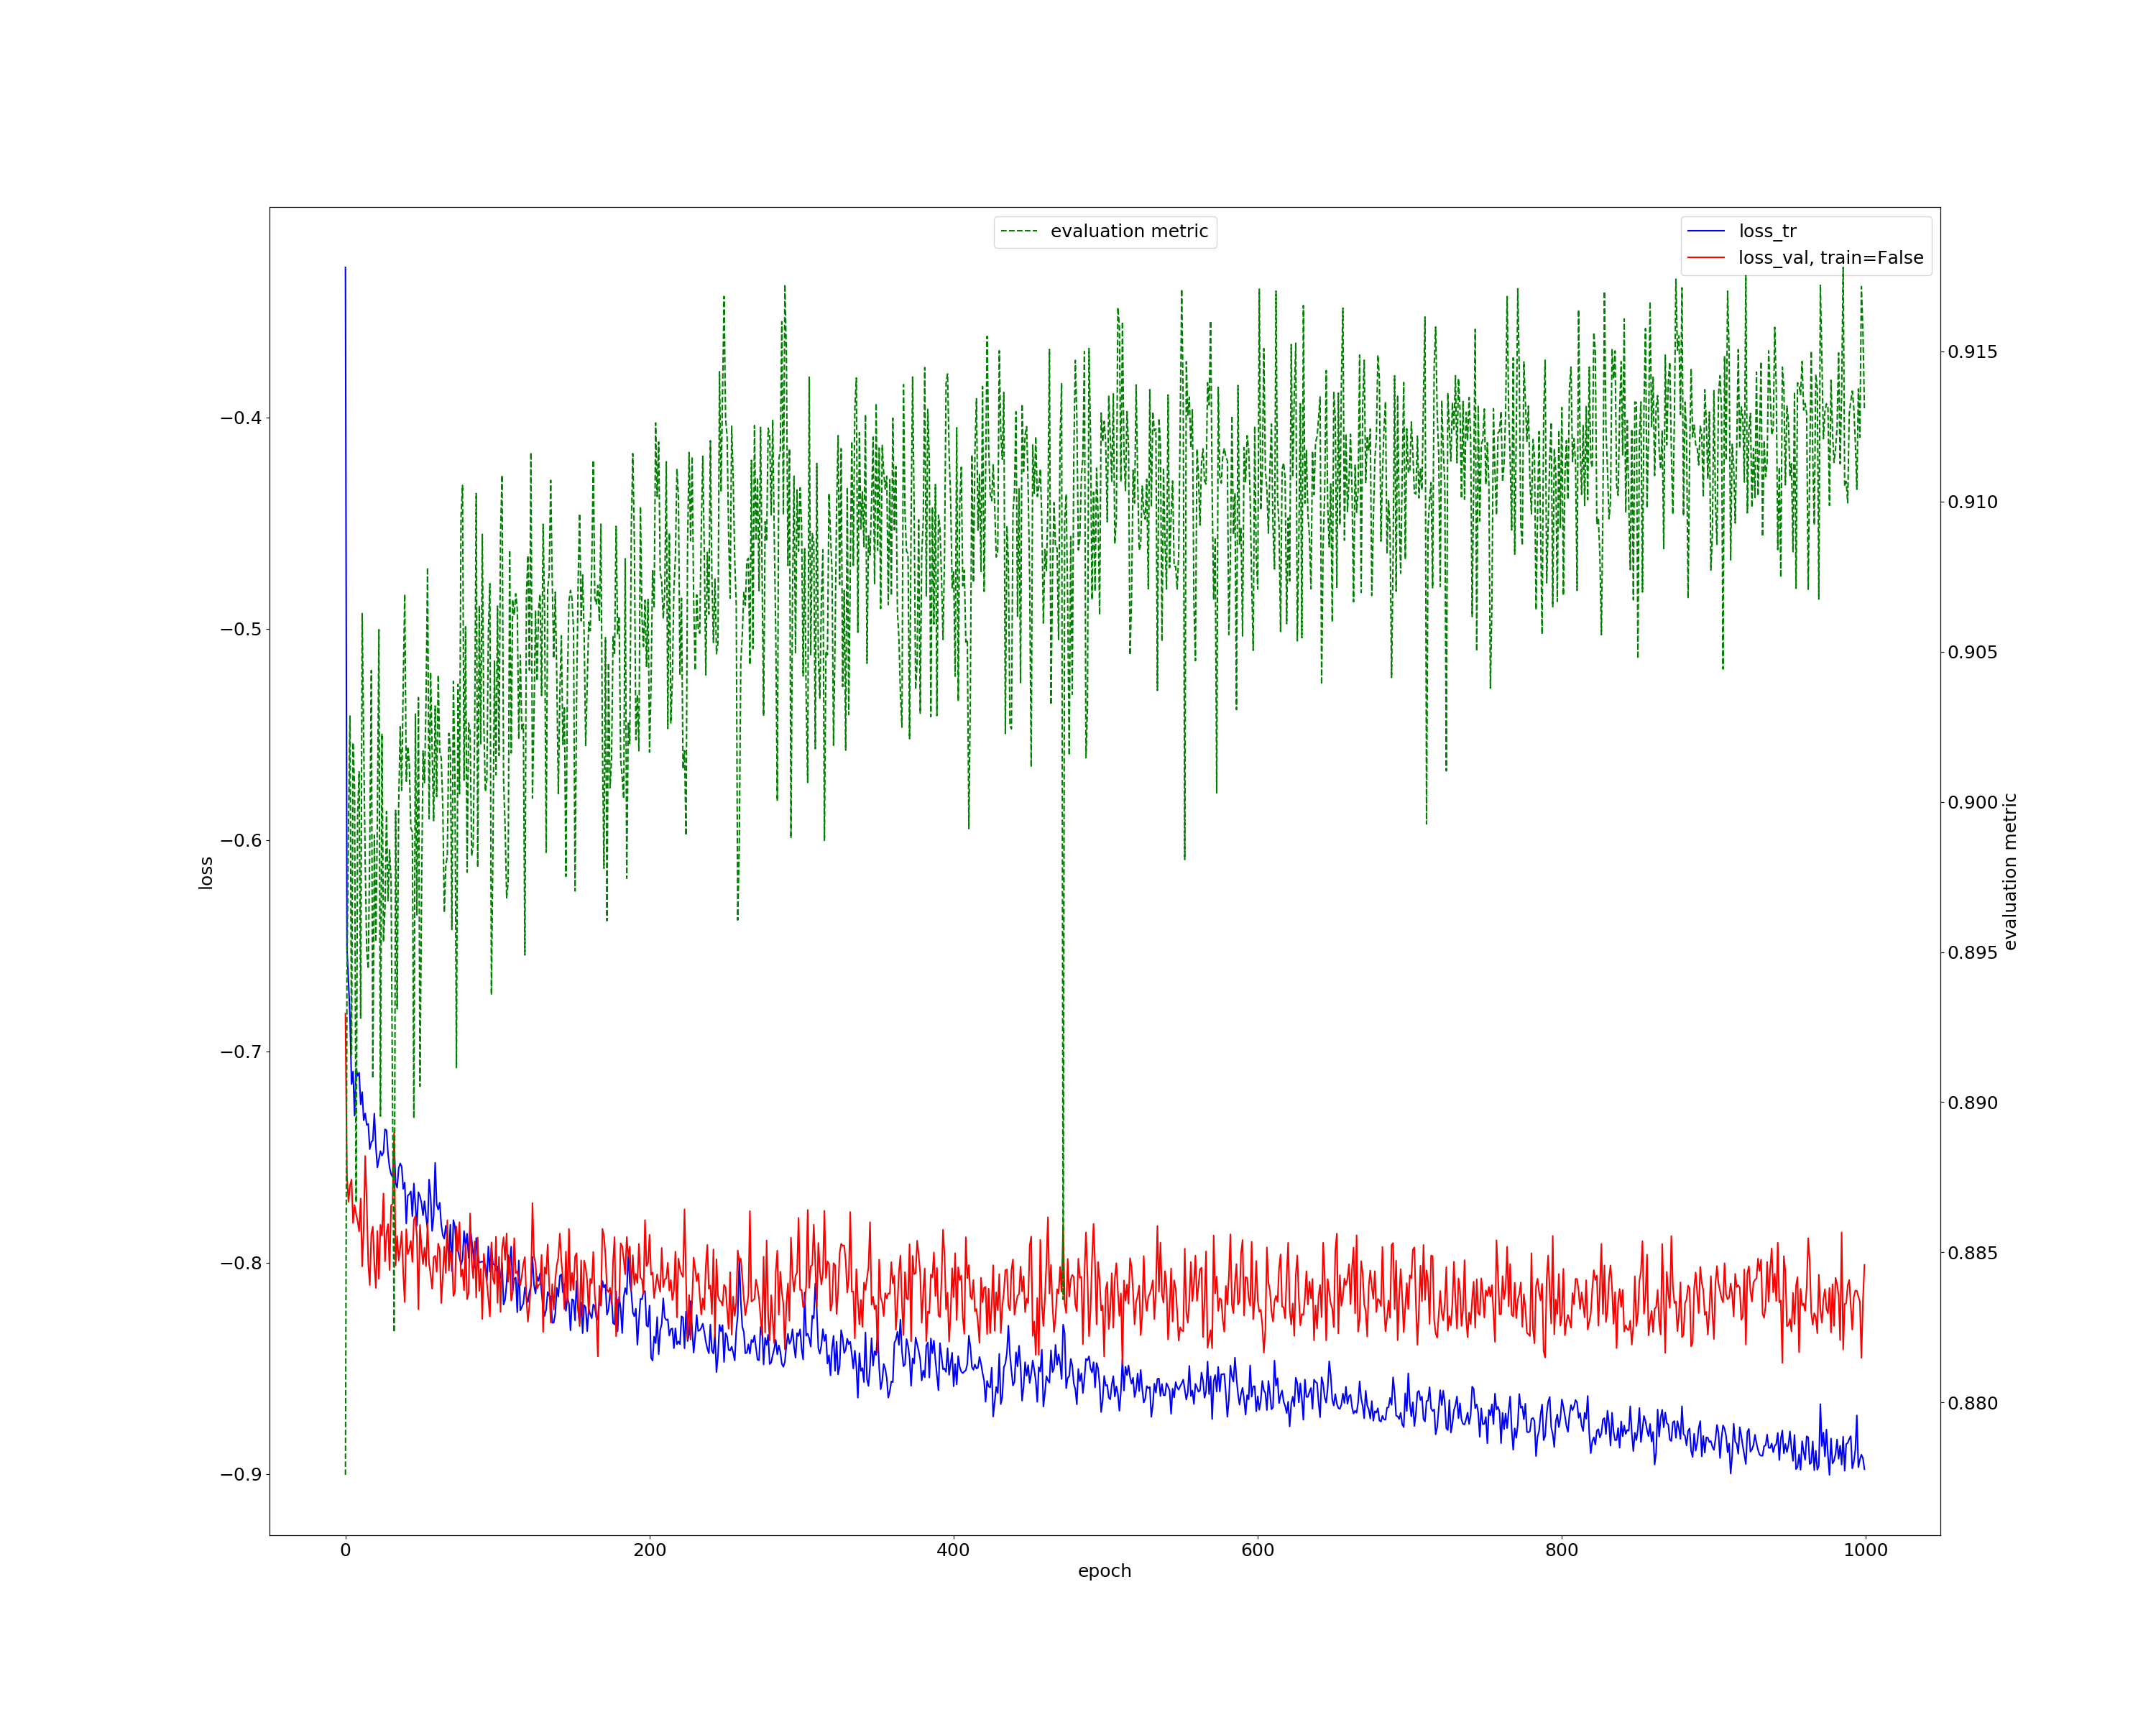}
& \includegraphics[ width=0.45\linewidth,height=0.27\linewidth,trim={1cm 0.5cm 0.25cm 1cm},clip,]{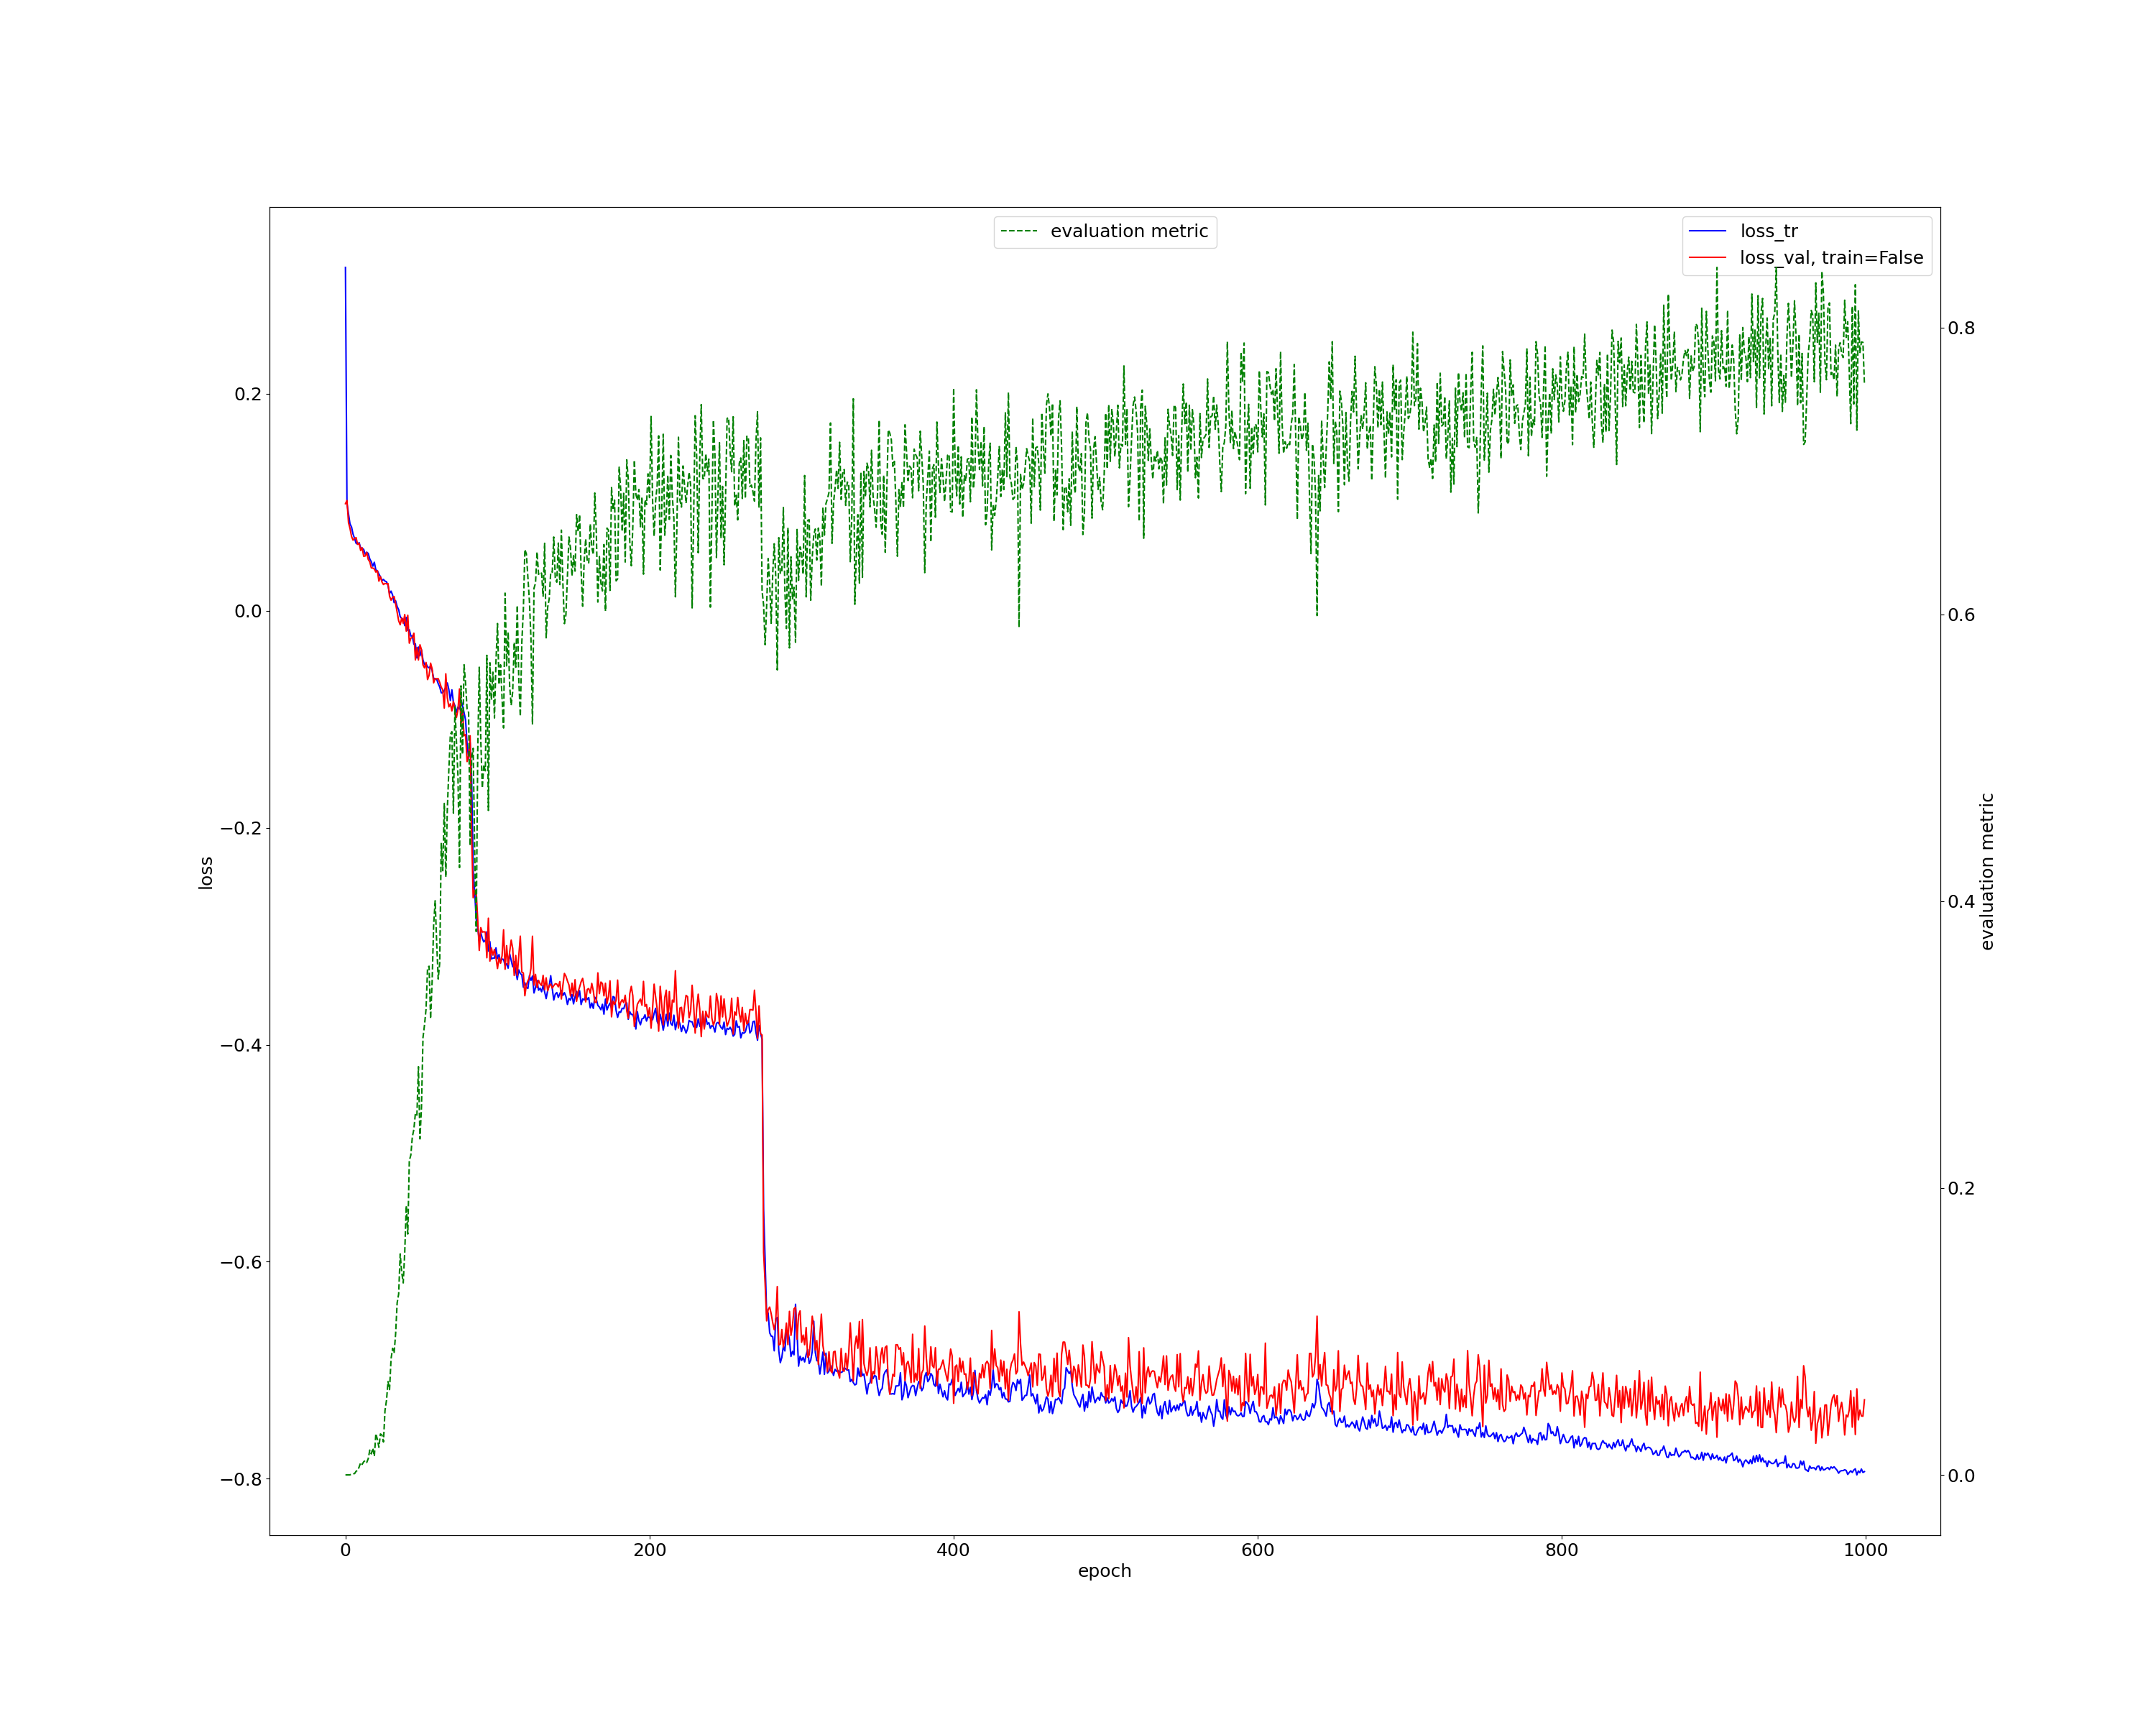}

\\

    \rotatebox{90}{$\;\;\;\;\;\;\;\;\;\;$ Split 4}
    & \includegraphics[ width=0.45\linewidth,height=0.27\linewidth,trim={1cm 0.5cm 0.25cm 1cm},clip,]{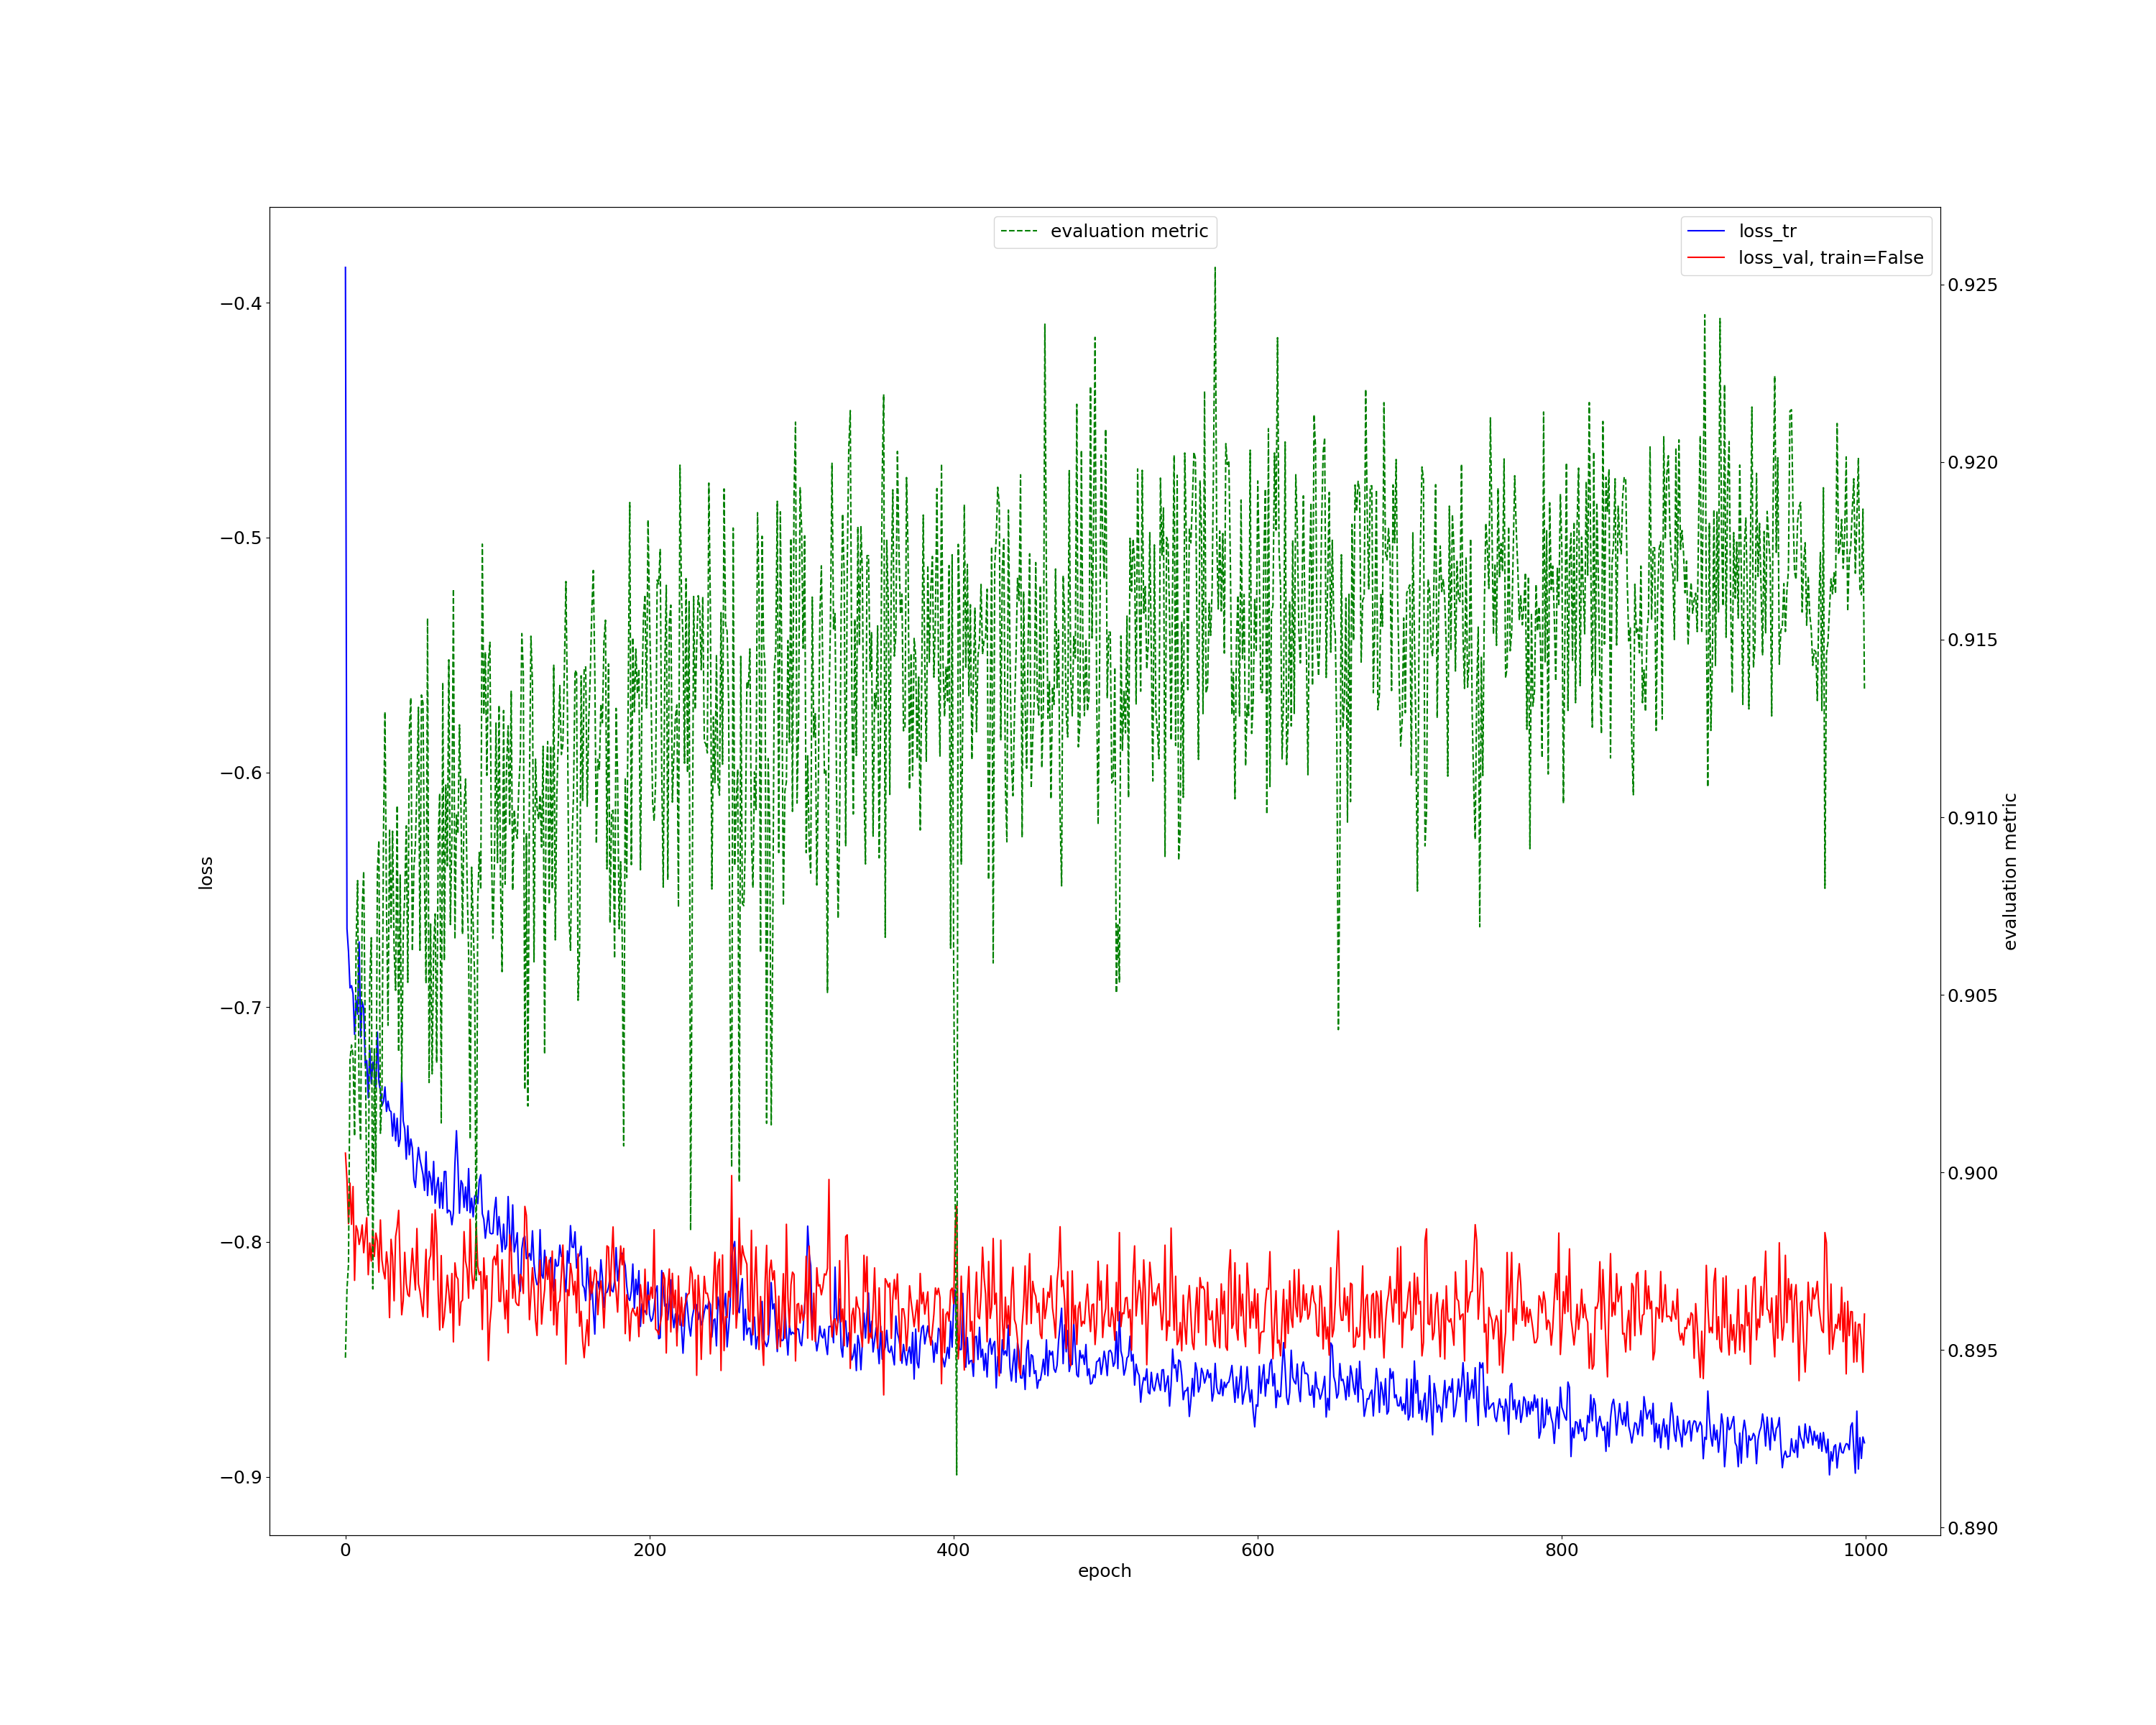}
& \includegraphics[width=0.45\linewidth,height=0.27\linewidth,trim={1cm 0.5cm 0.25cm 1cm},clip,]{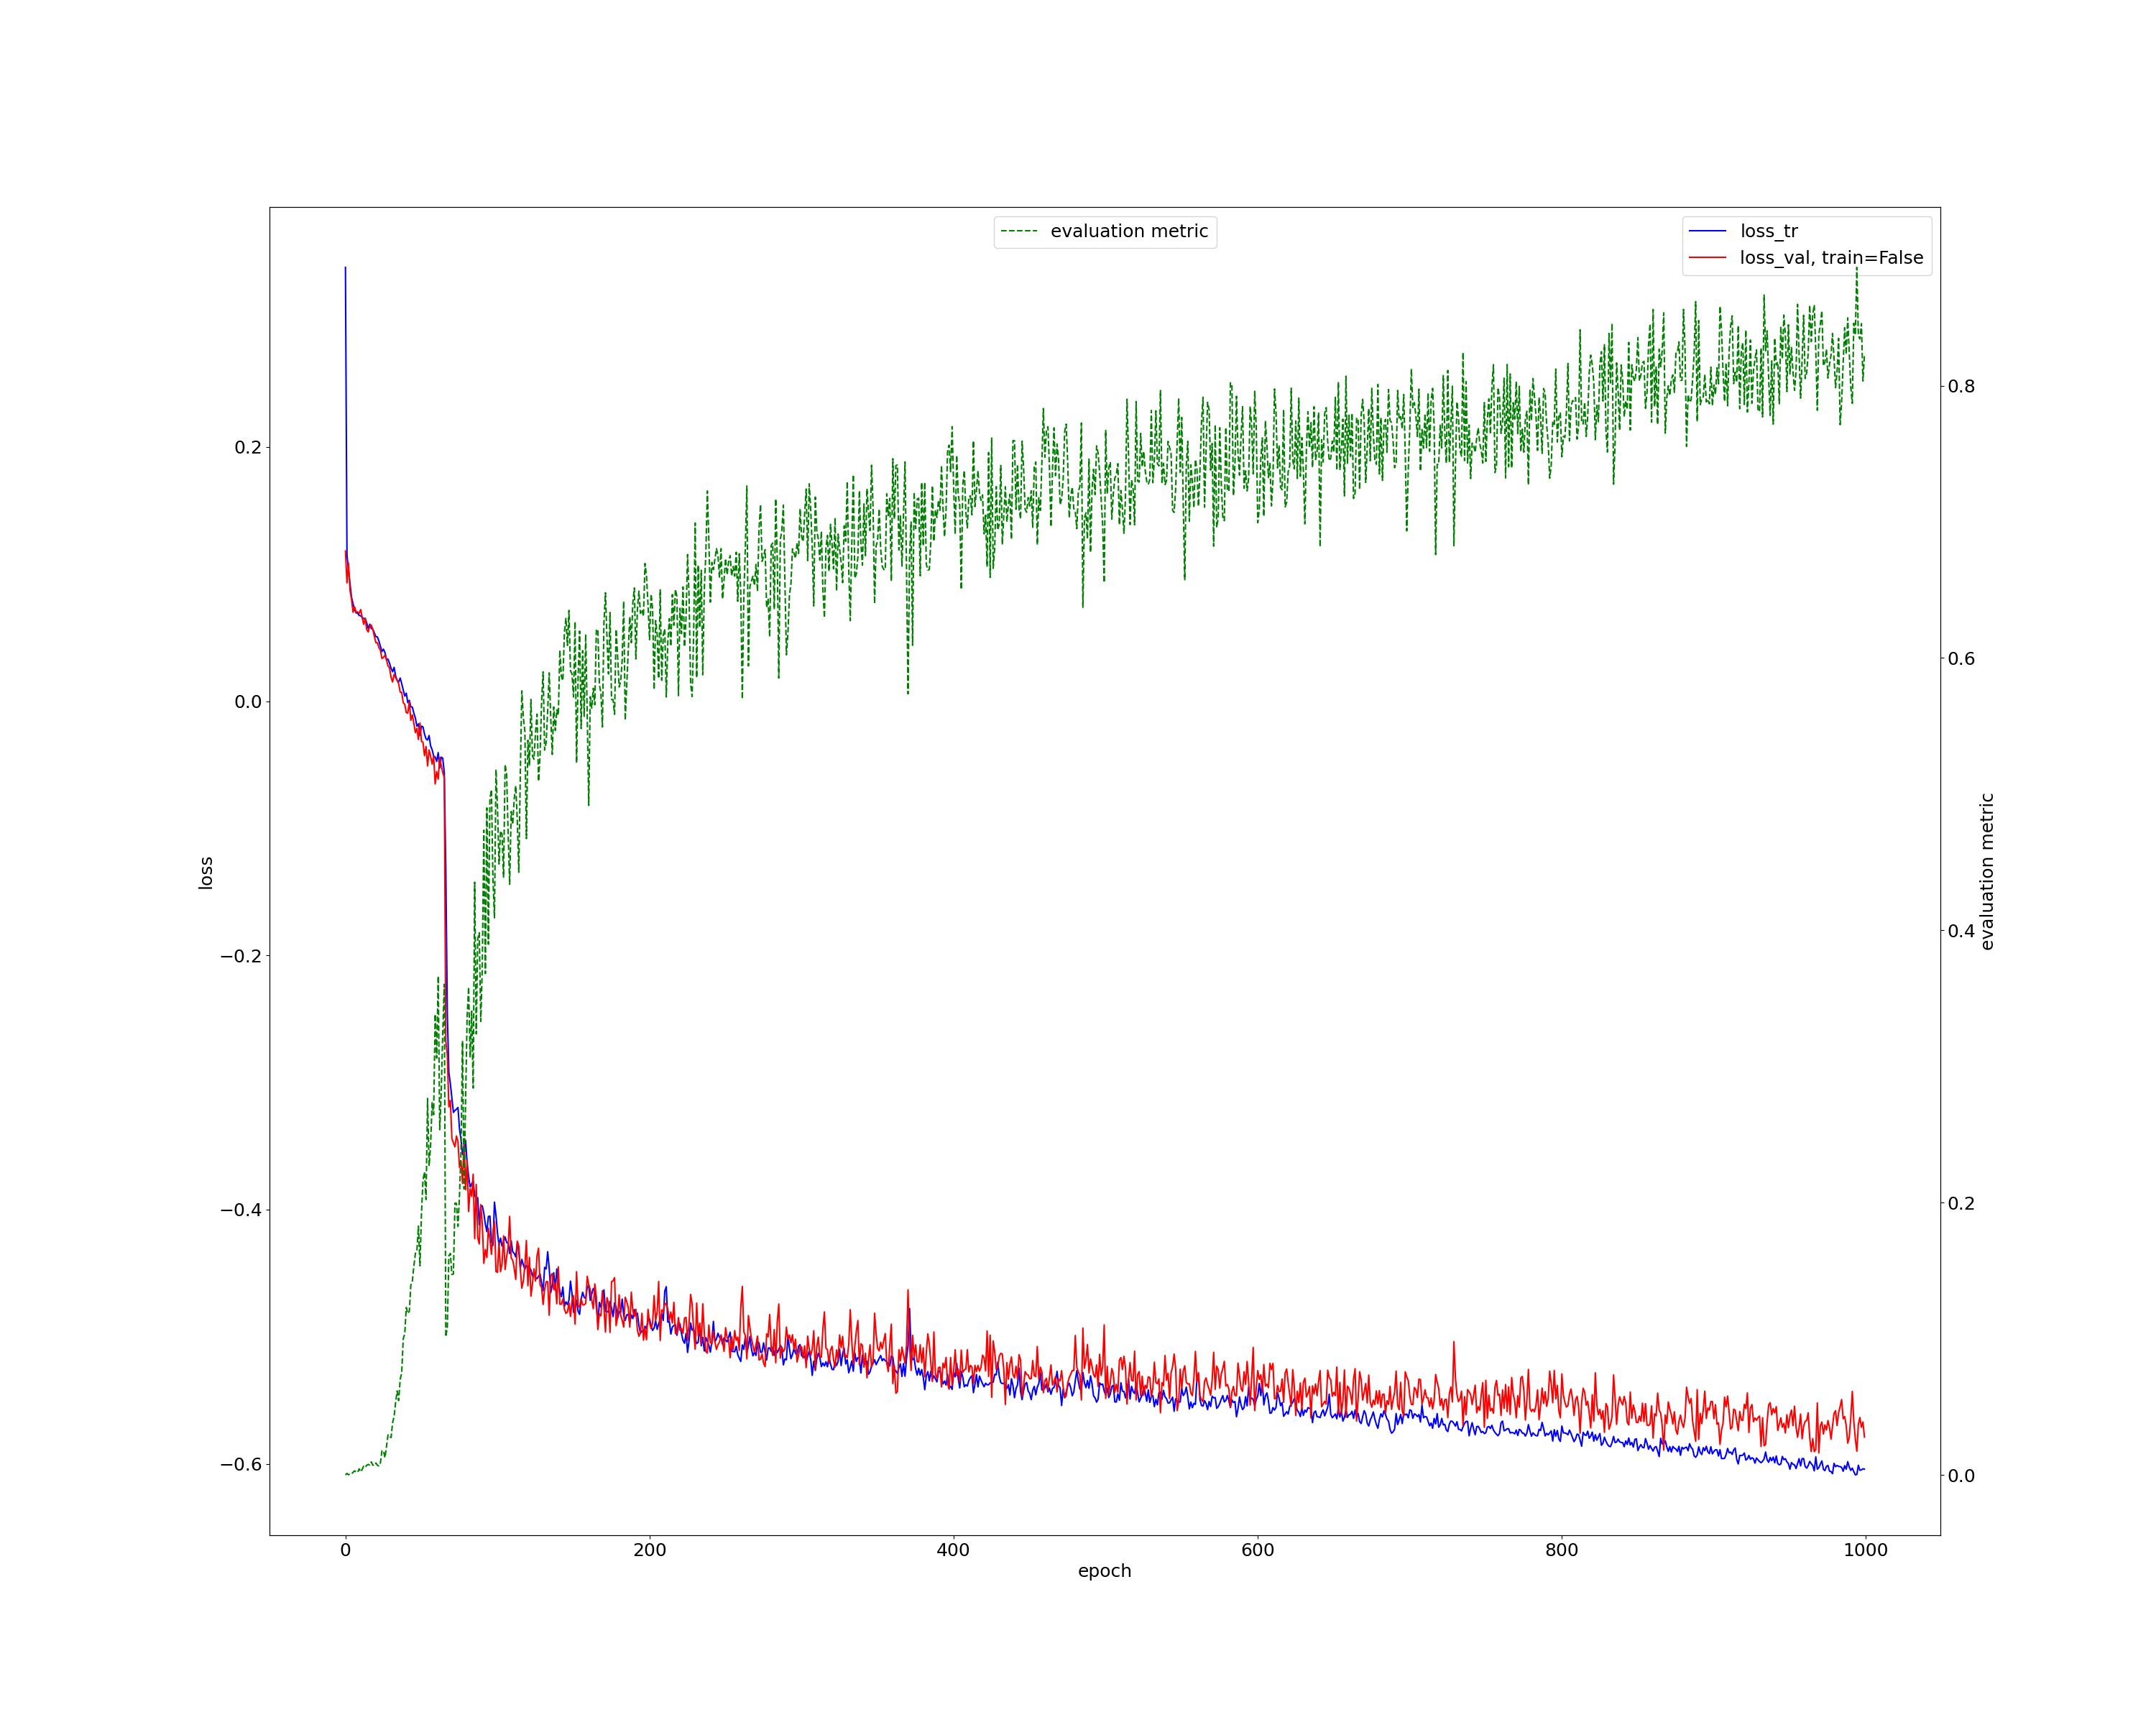}

\\

 \bottomrule
 
    \end{tabular}
    \caption{Visualization of training (Blue) and validation (Red) losses as well as validation performance (Green). For SegThor, the final validation performance ranges between 0.91 and 0.93 across all splits. For Verse, the final validation performance ranges between 0.82 and 0.84 across all splits. }
    \label{fig:training}
\end{figure*}
\subsection{2D Segmentation Results}
We show the segmentation performance on the PAXRay dataset for all classes in Table 2-7.
\subsection{Further Visual Examples of Predictions on Real X-Rays}
We show additional examples for network predictions on the OpenI dataset for both frontal and lateral views in Fig.~\ref{fig:supplementary_label_examples}. The segmentation results for the mediastinal classes, the sub-diaphragm, lung regions as well as most of the spine and ribs appear quite fitting for both views. One can notice that the prediction of individual ribs at times can be lacking despite the overall bone structure being segmented fine. Such errors can be seen in the overlapping areas of heart and ribs, possible attributable to the overall brighter region. Lungs vessel predictions in comparison to the annotations are quite coarse which is due to vessels being hardly visible in a chest X-ray.
\section{Grounding Dataset}
For our evaluation of medical phrase grounding, we use the OpenI dataset~\cite{openi} which consists of medical reports paired with frontal and lateral chest X-rays. When creating the validation dataset for CXR phrase grounding we tried to incorporate a large variety of phrases and anomalies.  We tasked two radiologist to highlight phrases within 100 medical reports for both the lateral and frontal (Anterior-Posterior/Posterior-Anterior) view in the OpenI dataset resulting in 178 frontal and 146 lateral bounding box annotations. We use the joined annotations as ground truth for the task.
 Following the NER-results of Stanza, these 100 reports resulted in annotated phrases with 90 different observations, 70 different observation modifiers, 88 different anatomies and 42 different anatomy modifiers. 
 
\setlength{\tabcolsep}{3pt}
\begin{table}[]
    \centering
    \caption{PAXRay Segmentation Performance for UNet and SegFPN with a ResNet50 backbone in IoU in \% (1/6)}
    \begin{tabular}{lrrr}
        \toprule
        {}     &  Lungs &  Right Lung &  Left Lung \\\midrule
        UNet &                                95.44 &                              90.63 &                             82.73 \\
         SegFPN  &                                94.91 &                               90.2 &                             82.09 \\ \midrule
        &  Left Upper Lobe &  Left Lower Lobe &  Right Upper Lobe \\\midrule 
        &                                       89.08 &                                       85.23 &                                        88.11 \\
        &                                       88.05 &                                       85.17 &                                        87.33 \\ \midrule
        &  Right Middle Lobe &  Right Lower Lobe &  Right Lung Vessel \\\midrule 
        &                                         81.68 &                                        87.46 &                                     54.65 \\
        &                                          79.6 &                                        86.88 &                                     55.65 \\ \midrule
        
        &  Left Lung Vessel &  Mediastinum &  Inferior Mediastinum \\\midrule 
        &                                    47.28 &                                       91.98 &                                     89.56 \\
        &                                    48.37 &                                       90.76 &                                     87.77 \\ \midrule
        
        &  Superior Mediastinum &  Anterior Mediastinum &  Middle Mediastinum \\\midrule 
        &                                      85.4 &                                        54.47 &                                      89.17 \\
        &                                     81.89 &                                        50.22 &                                      87.49 \\ \midrule
        
        &  Posterior Mediastinum &  Heart &  Airways \\\midrule 
        &                                         81.34 &                         89.73 &                           74.12 \\
        &                                         79.22 &                         88.76 &                           70.09 \\ \midrule 
        &  Esophagus &  Aorta &  Ascending Aorta \\\midrule 
        &                              68.2 &                          81.2 &                                   62.49 \\
        &                             65.19 &                         78.24 &                                   59.94 \\ \midrule 
        &  Aortic Arch &  Descending Aorta &  Bones \\\midrule 
&                               77.1 &                                    49.29 &                         90.87 \\
&                              71.53 &                                    45.99 &                         87.77 \\ \midrule 
&  Spine &  c1 &  c2 \\\midrule 
&                          92.6 &                         0.0 &                         0.0 \\
&                         90.38 &                         0.0 &                         0.0 \\ \midrule 
&  c3 &  c4 &  c5 \\\midrule 
&                         0.0 &                      1.71 &                      11.05 \\
&                         0.0 &                      00.62 &                      8.18 \\ \midrule 

\bottomrule
        \end{tabular}
    
    \label{tab:my_label}
\end{table}
\begin{table}[]
    \centering
        \caption{PAXRay Segmentation Performance (2/6)}

    \begin{tabular}{lrrr}
    \toprule
    &  c6 &  c7 &  t1 \\\midrule 
&                      37.83 &                      67.71 &                      78.87 \\
&                      30.45 &                      55.54 &                      67.88 \\ \midrule 
    &  t2 &  t3 &  t4 \\\midrule 
&                       79.2 &                      77.95 &                      78.01 \\
&                      69.61 &                      68.22 &                      67.35 \\ \midrule 
&  t5 &  t6 &  t7 \\\midrule 
&                      77.96 &                      78.05 &                      77.92 \\
&                      65.37 &                      64.86 &                      64.73 \\ \midrule 
&  t8 &  t9 &  t10 \\\midrule 
&                      77.48 &                      77.89 &                       78.66 \\
&                      65.58 &                      65.21 &                       65.37 \\ \midrule 
&  t11 &  t12 &  l1 \\\midrule 
&                       79.05 &                       80.16 &                      82.34 \\
&                       66.18 &                       66.58 &                      66.32 \\ \midrule 
     &  l2 &  l3 &  l4 \\\midrule 
&                      81.35 &                      76.28 &                      47.52 \\
&                      64.36 &                      60.97 &                      33.68 \\ \midrule 
&  l5 &  l6 &  sacrum \\\midrule 
&                      10.94 &                         0.0 &                             0.0 \\
&                       8.4 &                         0.0 &                             0.0 \\ \midrule 
&  cocygis &  t13 &  ribs \\\midrule 
&                              0.0 &                          0.0 &                        84.98 \\
&                              0.0 &                          0.0 &                        78.72 \\ \midrule 
&  Rib - 1 &  Rib - 2 &  Rib - 3 \\\midrule 
&                         76.43 &                         73.17 &                         70.99 \\
&                         70.31 &                         61.44 &                          57.1 \\ \midrule 
&  Rib - 4 &  Rib - 5 &  Rib - 6 \\\midrule 
&                          72.6 &                         70.12 &                         70.61 \\
&                         56.97 &                         54.81 &                         55.04 \\ \midrule 
 \bottomrule

\end{tabular}

    \label{tab:my_label}
\end{table}
\begin{table}[]
    \centering
        \caption{PAXRay Segmentation Performance (3/6)}

    \begin{tabular}{lrrr}
    \toprule
    &  Rib - 7 &  Rib - 8 &  Rib - 9 \\\midrule 
&                          70.7 &                          71.4 &                         72.19 \\
&                         56.19 &                         55.85 &                         56.89 \\ \midrule 
    &  Rib - 10 &  Rib - 11 &  Rib - 12\\\midrule 
&                          71.77 &                          59.75 &                          54.64 \\
&                          57.83 &                          47.93 &                          43.11 \\ \midrule 
&  Rib - Anterior -1 &  Rib - Posterior -1 &  Rib - Anterior -2 \\\midrule 
&                                  72.36 &                                   71.61 &                                   68.9 \\ 
&                                  68.09 &                                    64.2 &                                  57.34 \\ \midrule
&  Rib - Posterior -2 &  Rib - Anterior -3 &  Rib - Posterior -3 \\\midrule 
&                                   73.35 &                                  66.23 &                                   73.35 \\ 
&                                   62.73 &                                   52.7 &                                   60.97 \\ \midrule
&  Rib - Anterior -4 &  Rib - Posterior -4 &  Rib - Anterior -5 \\\midrule 
&                                  67.39 &                                   74.86 &                                  63.06 \\ 
&                                  52.28 &                                   61.38 &                                  48.69 \\ \midrule
& Rib - Posterior -5 &  Rib - Anterior -6 &  Rib - Posterior -6 \\\midrule 
&                                    73.6 &                                  63.96 &                                   71.48 \\
&                                   60.37 &                                  48.63 &                                   58.12\\ \midrule
&  Rib - Anterior -7 &  Rib - Posterior -7 &  Rib - Anterior -8 \\\midrule 
&                                  61.29 &                                    71.3 &                                  59.96  \\
&                                  47.53 &                                   57.65 &                                  46.81 \\ \midrule
&  Rib - Posterior -8 &  Rib - Anterior -9 &  Rib - Posterior -9\\\midrule 
&                                   72.83 &                                  60.56 &                                   72.67 \\
&                                   57.68 &                                  46.57 &                                   57.71\\ \midrule
&  Rib - Anterior -10 &  Rib - Posterior -10 &  Rib - Anterior -11\\\midrule 
&                                    54.3 &                                    70.42 &                                   9.54 \\
&                                   40.88 &                                    57.98 &                                    4.1\\ \midrule
&  Rib - Posterior -11 &  Rib - Anterior -12 &  Rib - Posterior -12\\\midrule
&                                    59.65 &                                   4.79 &                                    53.23\\ 
&                                    48.01 &                                   1.27 &                                    41.58\\\midrule

    \end{tabular}
    \label{tab:my_label}
\end{table}

\begin{table}[]
    \centering
        \caption{PAXRay Segmentation Performance (4/6)}

    \begin{tabular}{lrrr}
    \toprule
             &  Rib - Left - 1 &  Rib - Right - 1 &  Rib - Left - 2 \\ \midrule
&                              67.22 &                               68.72 &                              62.72 \\
&                              63.02 &                               63.59 &                              53.12 \\ \midrule
&  Rib - Right - 2 &  Rib - Left - 3 &  Rib - Right - 3 \\ \midrule
&                               65.49 &                              61.35 &                                61.3 \\ 
&                               55.17 &                              49.12 &                               49.99 \\ \midrule
&  Rib - Left - 4 &  Rib - Right - 4 &  Rib - Left - 5 \\ \midrule
&                              61.12 &                               62.71 &                              57.52 \\ 
&                              48.29 &                               50.89 &                              44.62 \\ \midrule
&  Rib - Right - 5 &  Rib - Left - 6 &  Rib - Right - 6 \\ \midrule
&                               61.17 &                              59.32 &                               62.55 \\ 
&                               49.57 &                              45.67 &                               50.27 \\  \midrule 
&  Rib - Left - 7 &  Rib - Right - 7 &  Rib - Left - 8 \\  \midrule 
&                               59.8 &                               63.92 &                              60.29 \\  
&                              46.84 &                               51.72 &                              46.39 \\  \midrule 
&  Rib - Right - 8 &  Rib - Left - 9 &  Rib - Right - 9 \\ \midrule 
&                               63.31 &                              61.27 &                               62.39 \\  
&                               51.95 &                              48.18 &                               51.52 \\  \midrule 
 &  Rib - Left - 10 &  Rib - Right - 10 &  Rib - Left - 11 \\  \midrule 
&                               59.04 &                                61.27 &                               46.06 \\ 
&                               46.69 &                                 52.6 &                               35.51 \\ \midrule 
&  Rib - Right - 11 &  Rib - Left - 12 &  Rib - Right - 12 \\  \midrule 
&                                52.32 &                               42.28 &                                46.77 \\ 
&                                43.08 &                               35.04 &                                 34.1 \\ \midrule 
&  Rib - Left - Anterior -1 &  Rib - Left - Posterior -1 &  Rib - Left - Anterior -2  \\ \midrule
&                                       65.15 &                                         60.8 &                                       65.12 \\
&                                       61.68 &                                        56.58 &                                       60.91 \\ \midrule
&  Rib - Left - Posterior -2 &  Rib - Left - Anterior -3 &  Rib - Left - Posterior -3  \\ \midrule
&                                        65.14 &                                       59.25 &                                        61.25\\
&                                        59.28 &                                        48.4 &                                        54.35\\ \midrule
    \end{tabular}
    \label{tab:my_label}
\end{table}

\begin{table}[]
    \centering
        \caption{PAXRay Segmentation Performance (5/6)}

    \begin{tabular}{lrrr}
    \toprule
    &  Rib - Left - Anterior -4 &  Rib - Left - Posterior -4 &  Rib - Left - Anterior -5  \\ \midrule
&                                       62.13 &                                         65.1 &                                       58.13 \\
&                                       50.95 &                                         55.9 &                                       44.78 \\ \midrule
&  Rib - Left - Posterior -5 &  Rib - Left - Anterior -6 &  Rib - Left - Posterior -6 \\ \midrule
&                                        60.12 &                                       56.42 &                                        64.76\\
&                                        50.25 &                                       45.63 &                                        54.84\\ \midrule
    &  Rib - Left - Anterior -7 &  Rib - Left - Posterior -7 &  Rib - Left - Anterior -8  \\ \midrule
&                                       57.04 &                                        62.28 &                                       58.09 \\
&                                       44.34 &                                        52.02 &                                       46.96 \\ \midrule
&  Rib - Left - Posterior -8 &  Rib - Left - Anterior -9 &  Rib - Left - Posterior -9 \\ \midrule
&                                        65.33 &                                       50.97 &                                        61.23\\
&                                        55.15 &                                       39.15 &                                        50.43\\ \midrule
&  Rib - Left - Anterior -10 &  Rib - Left - Posterior -10 &  Rib - Left - Anterior -11 \\ \midrule
&                                        55.18 &                                         63.21 &                                        53.43\\
&                                         45.3 &                                         53.55 &                                        39.72\\ \midrule
    &  Rib - Left - Posterior -11 &  Rib - Left - Anterior -12 &  Rib - Left - Posterior -12 \\ \midrule
&                                         60.69 &                                        57.17 &                                         62.79\\
&                                         47.98 &                                        45.03 &                                         52.99\\ \midrule

         &  Rib - Right - Anterior -1 &  Rib - Right - Posterior -1 &  Rib - Right - Anterior -2  \\ \midrule
&                                        51.21 &                                         60.34 &                                        54.15 \\
&                                        38.86 &                                         48.28 &                                        42.56 \\ \midrule
&  Rib - Right - Posterior -2 &  Rib - Right - Anterior -3 &  Rib - Right - Posterior -3  \\ \midrule 
&                                         65.62 &                                        48.55 &                                         62.19\\
&                                         53.87 &                                        37.94 &                                         48.39\\ \midrule
&  Rib - Right - Anterior -4 &  Rib - Right - Posterior -4 &  Rib - Right - Anterior -5 \\ \midrule
&                                        52.04 &                                         65.25 &                                        48.98 \\
&                                        40.85 &                                         53.91 &                                        35.43 \\ \midrule

\bottomrule
    
\end{tabular}
    \label{tab:my_label}
\end{table}

\begin{table}[]
    \centering
        \caption{PAXRay Segmentation Performance (6/6)}

    \begin{tabular}{lrrr}
    \toprule
    &  Rib - Right - Posterior -5 &  Rib - Right - Anterior -6 &  Rib - Right - Posterior -6 \\ \midrule
&                                         62.69 &                                        50.69 &                                          63.8\\
&                                         49.37 &                                        39.66 &                                         53.08\\ \midrule
&  Rib - Right - Anterior -7 &  Rib - Right - Posterior -7 &  Rib - Right - Anterior -8\\  \midrule
&                                        36.76 &                                         58.41 &                                        43.77 \\
&                                        26.17 &                                         46.67 &                                        34.46 \\ \midrule
&  Rib - Right - Posterior -8 &  Rib - Right - Anterior -9 &  Rib - Right - Posterior -9 \\\midrule
&                                          61.3 &                                        5.13 &                                         45.54\\
&                                         52.86 &                                        02.42 &                                         35.21\\ \midrule
    &  Rib - Right - Anterior -10 &  Rib - Right - Posterior -10 &  Rib - Right - Anterior -11\\\midrule
&                                         6.41 &                                           50.9 &                                         0.27\\
&                                         03.1 &                                          41.91 &                                            0.0\\ \midrule
 &  Rib - Right - Posterior -11 &  Rib - Right - Anterior -12 &  Rib - Right - Posterior -12 \\\midrule
&                                          37.64 &                                         0.11 &                                          43.84\\
&                                          30.32 &                                            0.0 &                                          31.95\\ \midrule
&  Diaphragm &  Hemidiaphragm - Right &  Hemidiaphragm - Left \\\midrule
&                              96.8 &                                       94.08 &                                      93.67\\ 
&                             96.15 &                                       93.87 &                                      93.25\\  \midrule
&  Mean \\\midrule
&             60.69 \\
&             51.87 \\  
\bottomrule
    
\end{tabular}
    \label{tab:my_label}
\end{table}
