# Supplementary material for: Detailed Annotations of Chest X-Rays via CT Projection for Report Understanding
Source: arXiv:2210.03416 source file (2022-10-07)
Supplement: Supplementary file 2 [file 3dsuppslice.tex]

\begin{figure}[h!]
    \centering
    \includegraphics[width=\linewidth, trim={0 3.5cm 0cm 7cm},clip]{images/supplementary_dataset_examples/ribfrac11.png}
    \caption{Example of a axial slice of a 3D Volume of the RibFrac dataset, where the two lung halves overlap along the sagittal plane}
    \label{fig:3dslice_supp}
\end{figure}
