# Supplementary material for: Detailed Annotations of Chest X-Rays via CT Projection for Report Understanding
Source: arXiv:2210.03416 source file (2022-10-07)
Supplement: Supplementary file 3 [file 3dtraining.tex]

\setlength{\tabcolsep}{-7pt}

\begin{figure*}
    \centering
    \begin{tabular}{ccc}
    \toprule
    & SegThor & Verse\\\midrule
    
    \rotatebox{90}{$\;\;\;\;\;\;\;\;\;\;$ Split 0}
    
    & \includegraphics[ width=0.45\linewidth,height=0.27\linewidth,trim={1cm 0.5cm 0.25cm 1cm},clip,]{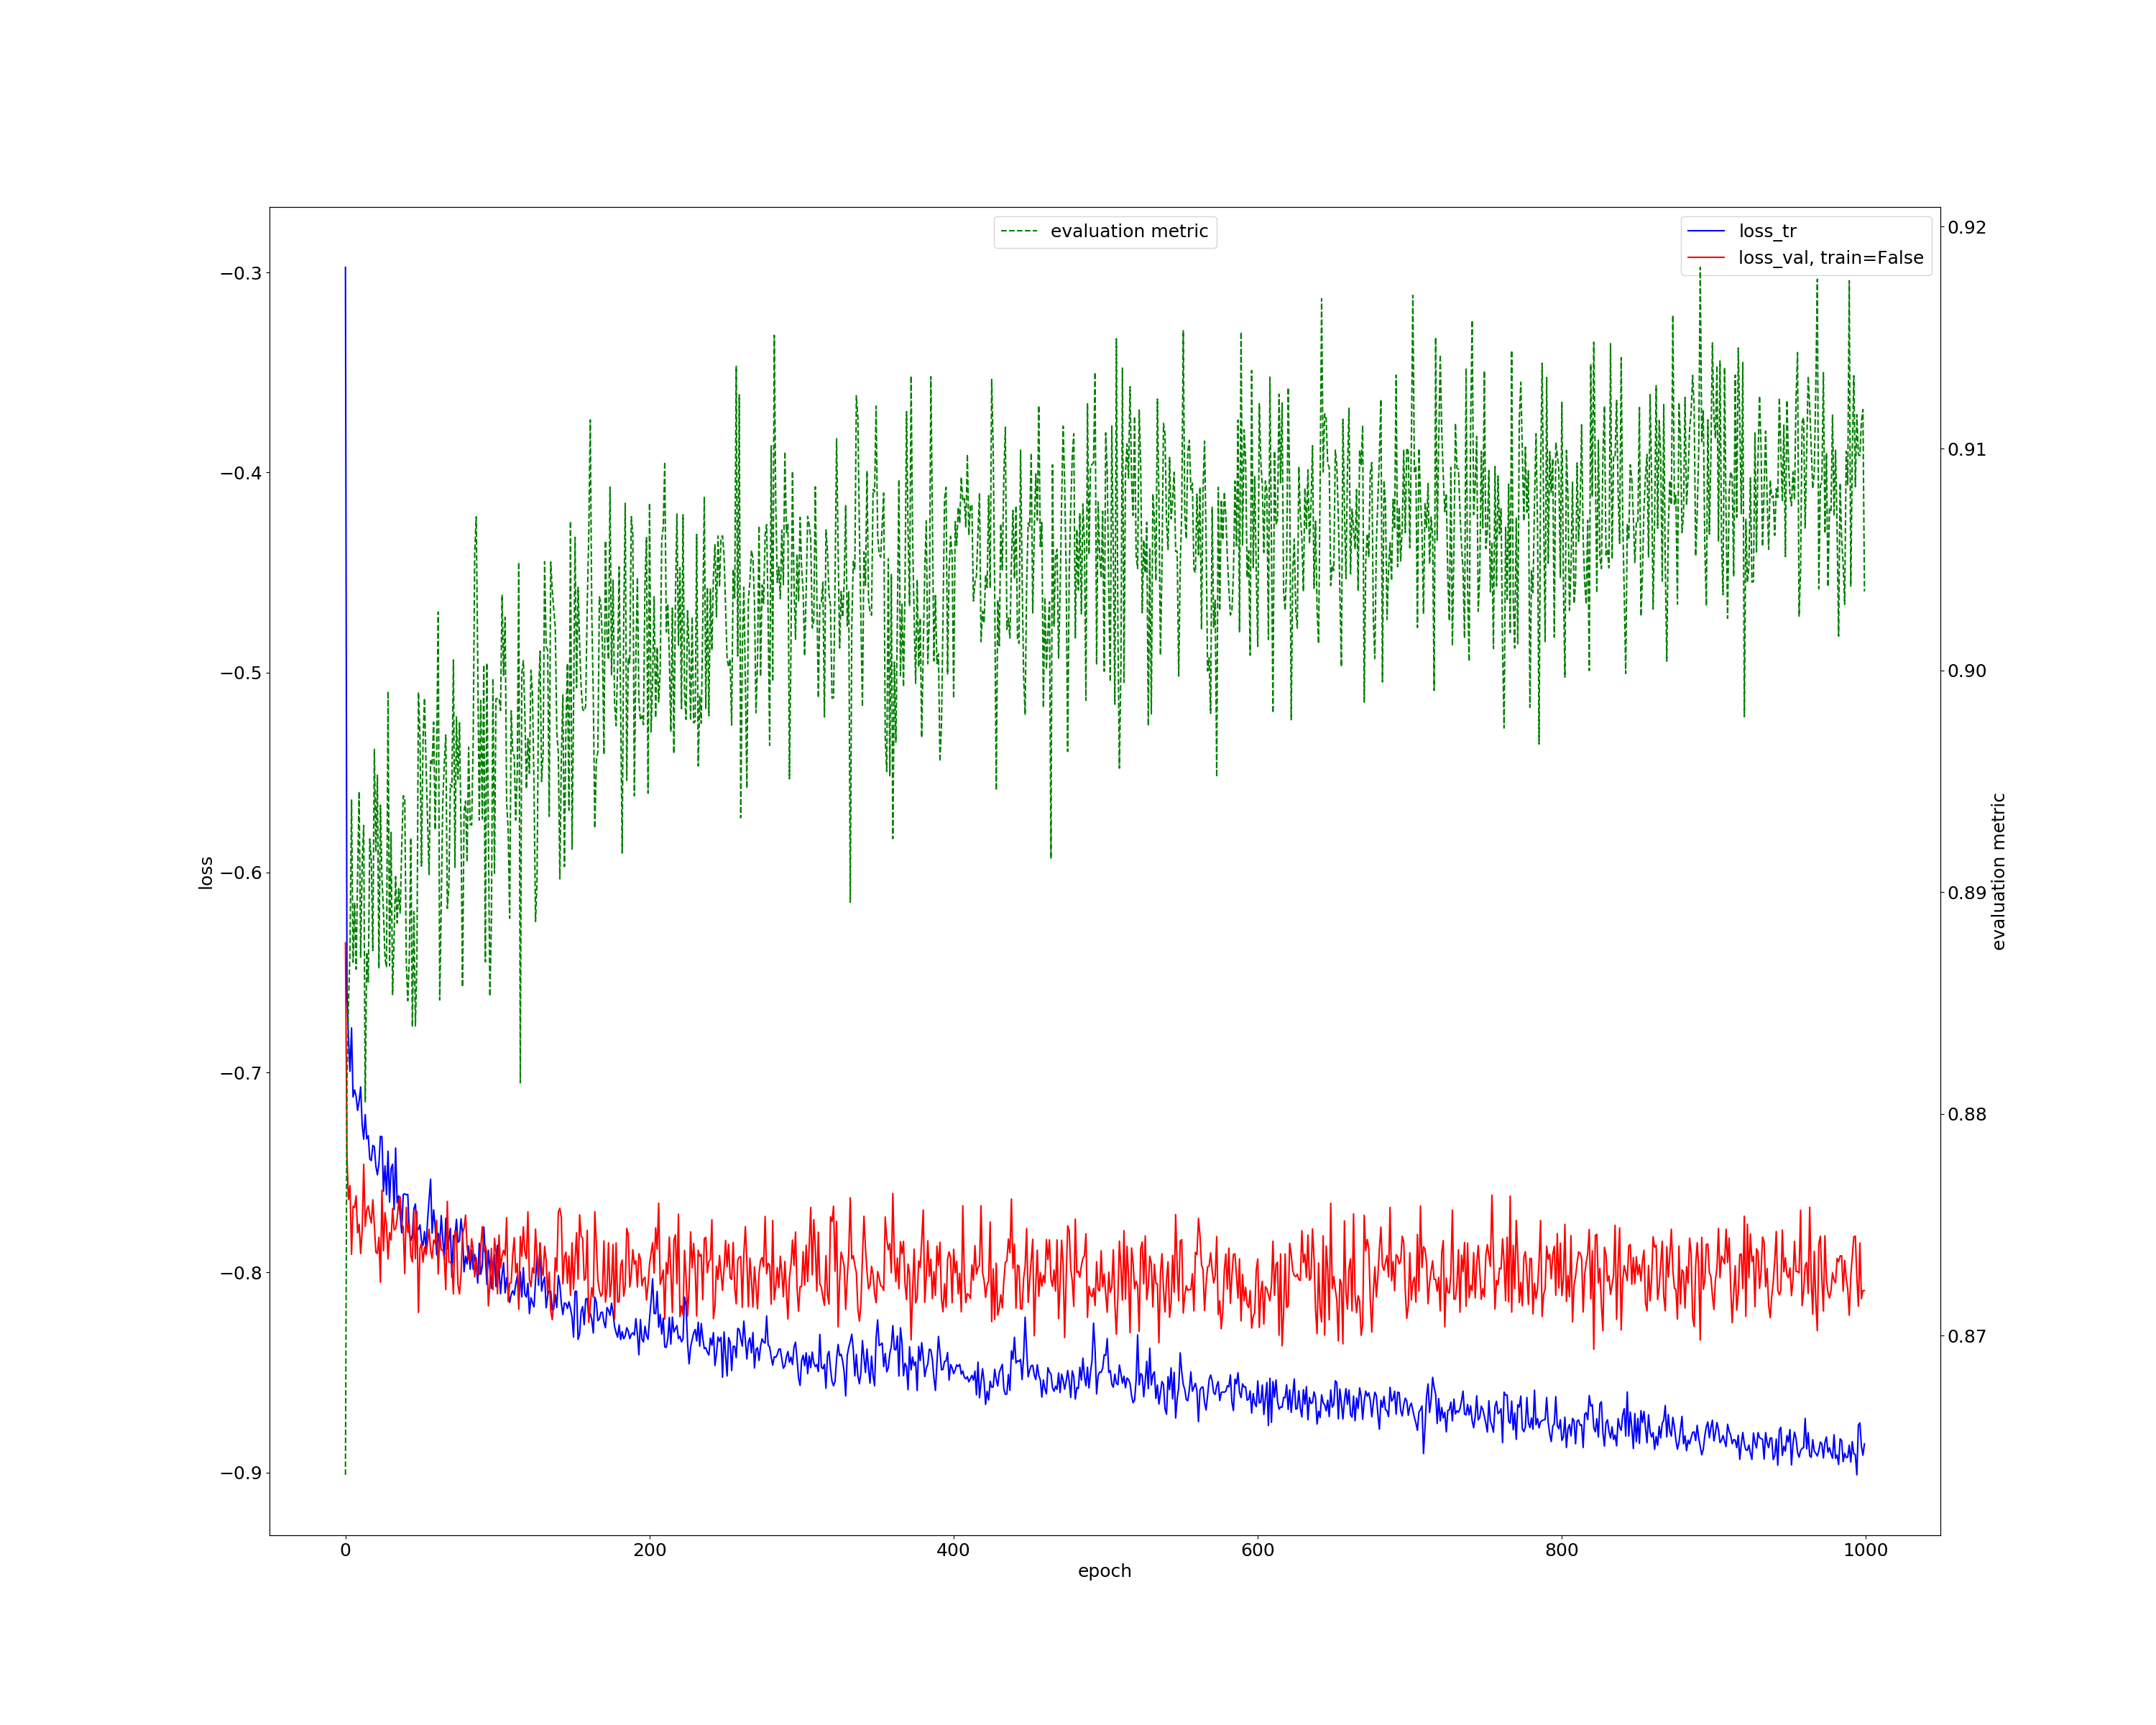}
    & \includegraphics[ width=0.45\linewidth,height=0.27\linewidth,trim={1cm 0.5cm 0.25cm 1cm},clip,]{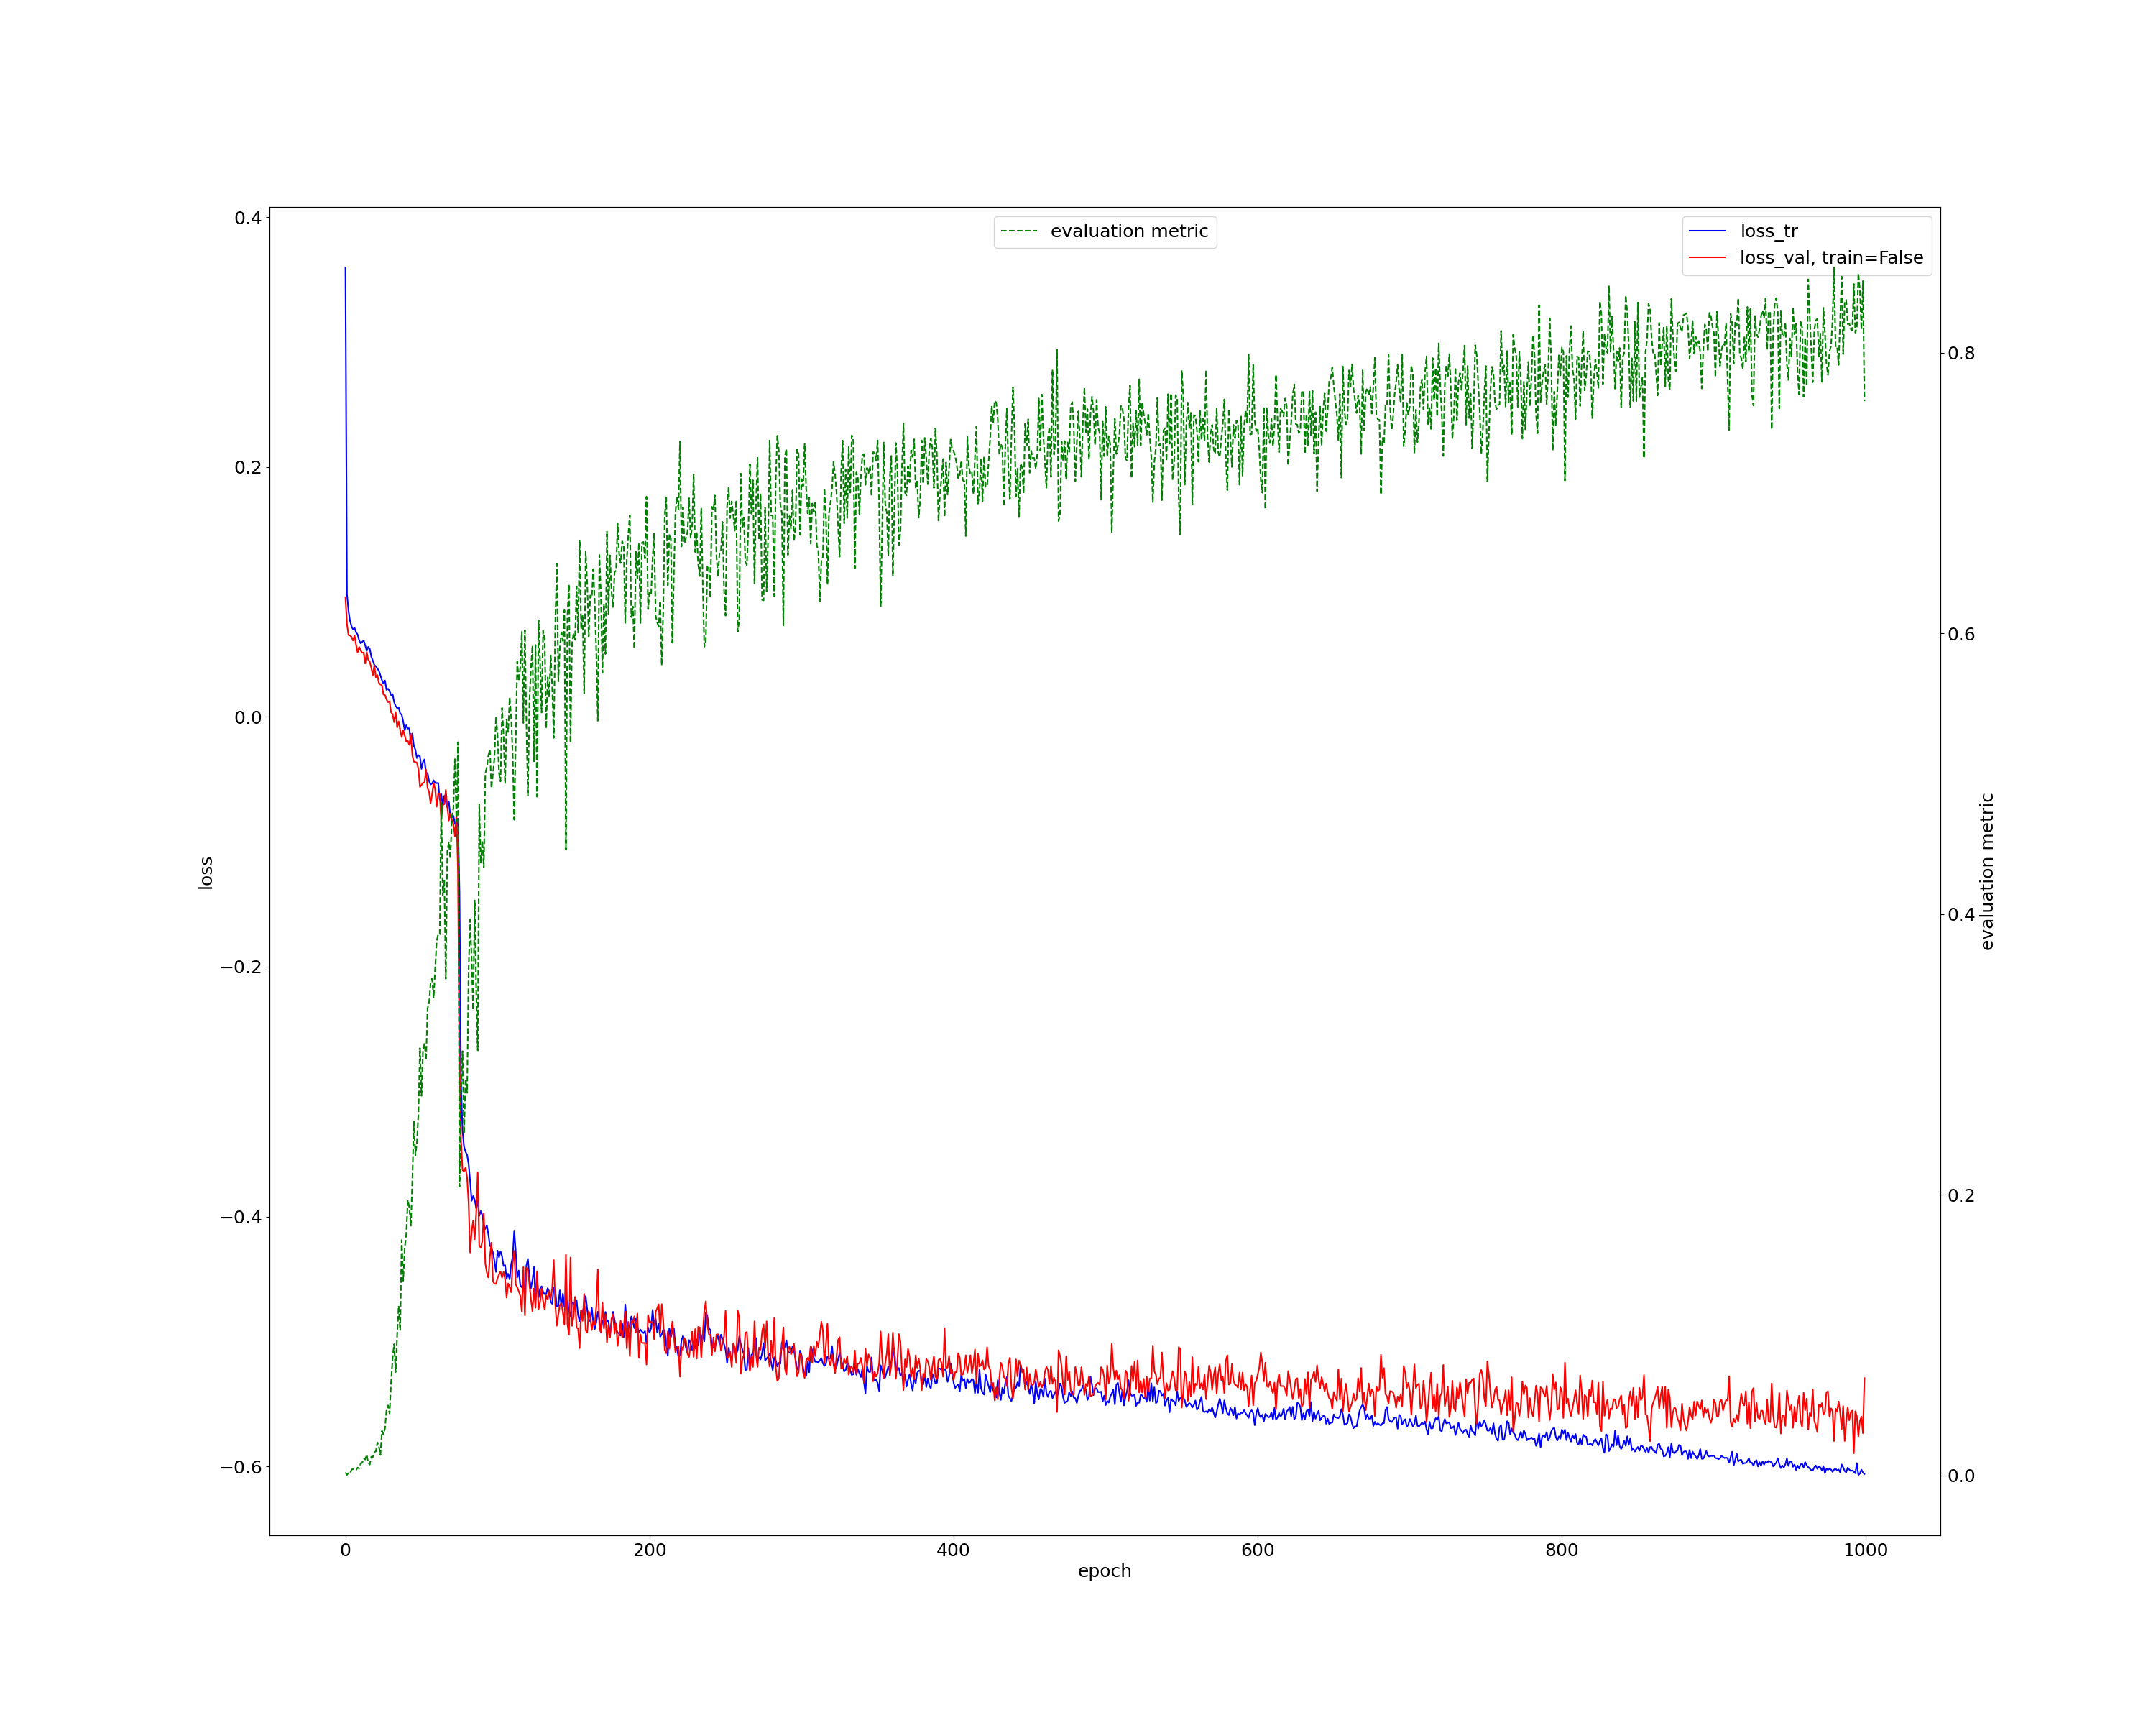}
    
    \\
    
    \rotatebox{90}{$\;\;\;\;\;\;\;\;\;\;$ Split 1}
    & \includegraphics[ width=0.45\linewidth,height=0.27\linewidth,trim={1cm 0.5cm 0.25cm 1cm},clip,]{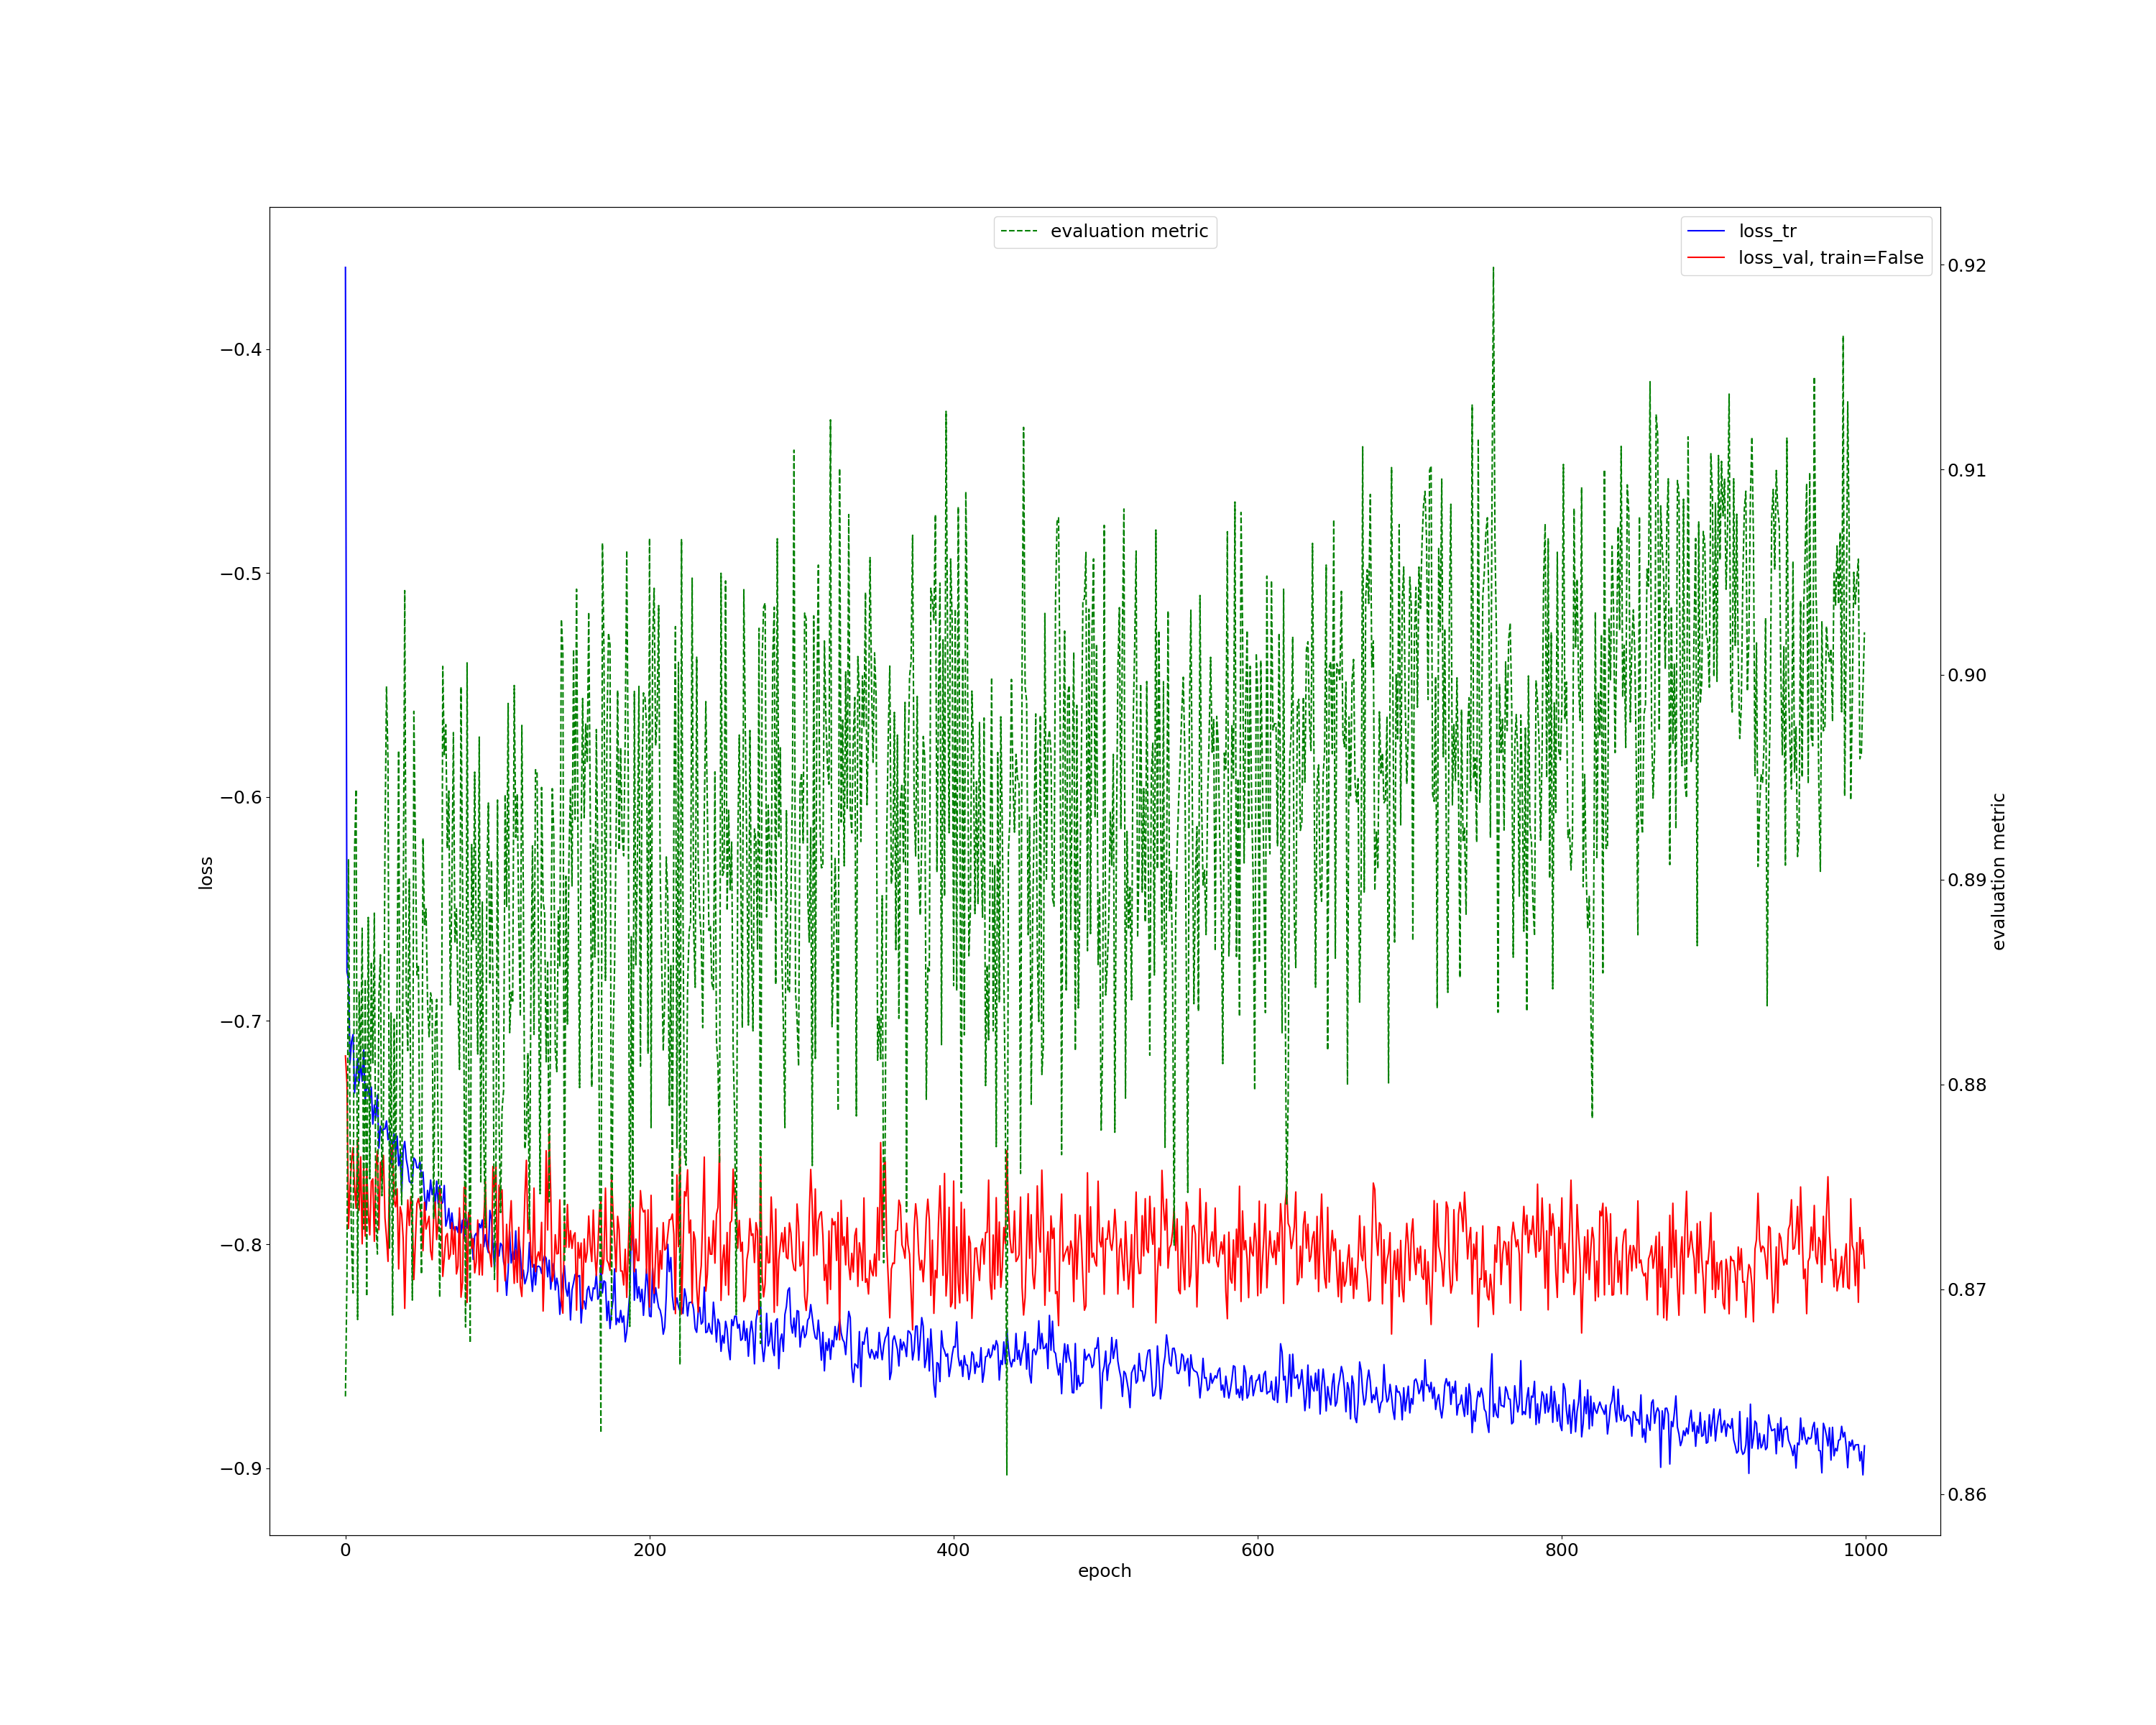}
& \includegraphics[ width=0.45\linewidth,height=0.27\linewidth,trim={1cm 0.5cm 0.25cm 1cm},clip,]{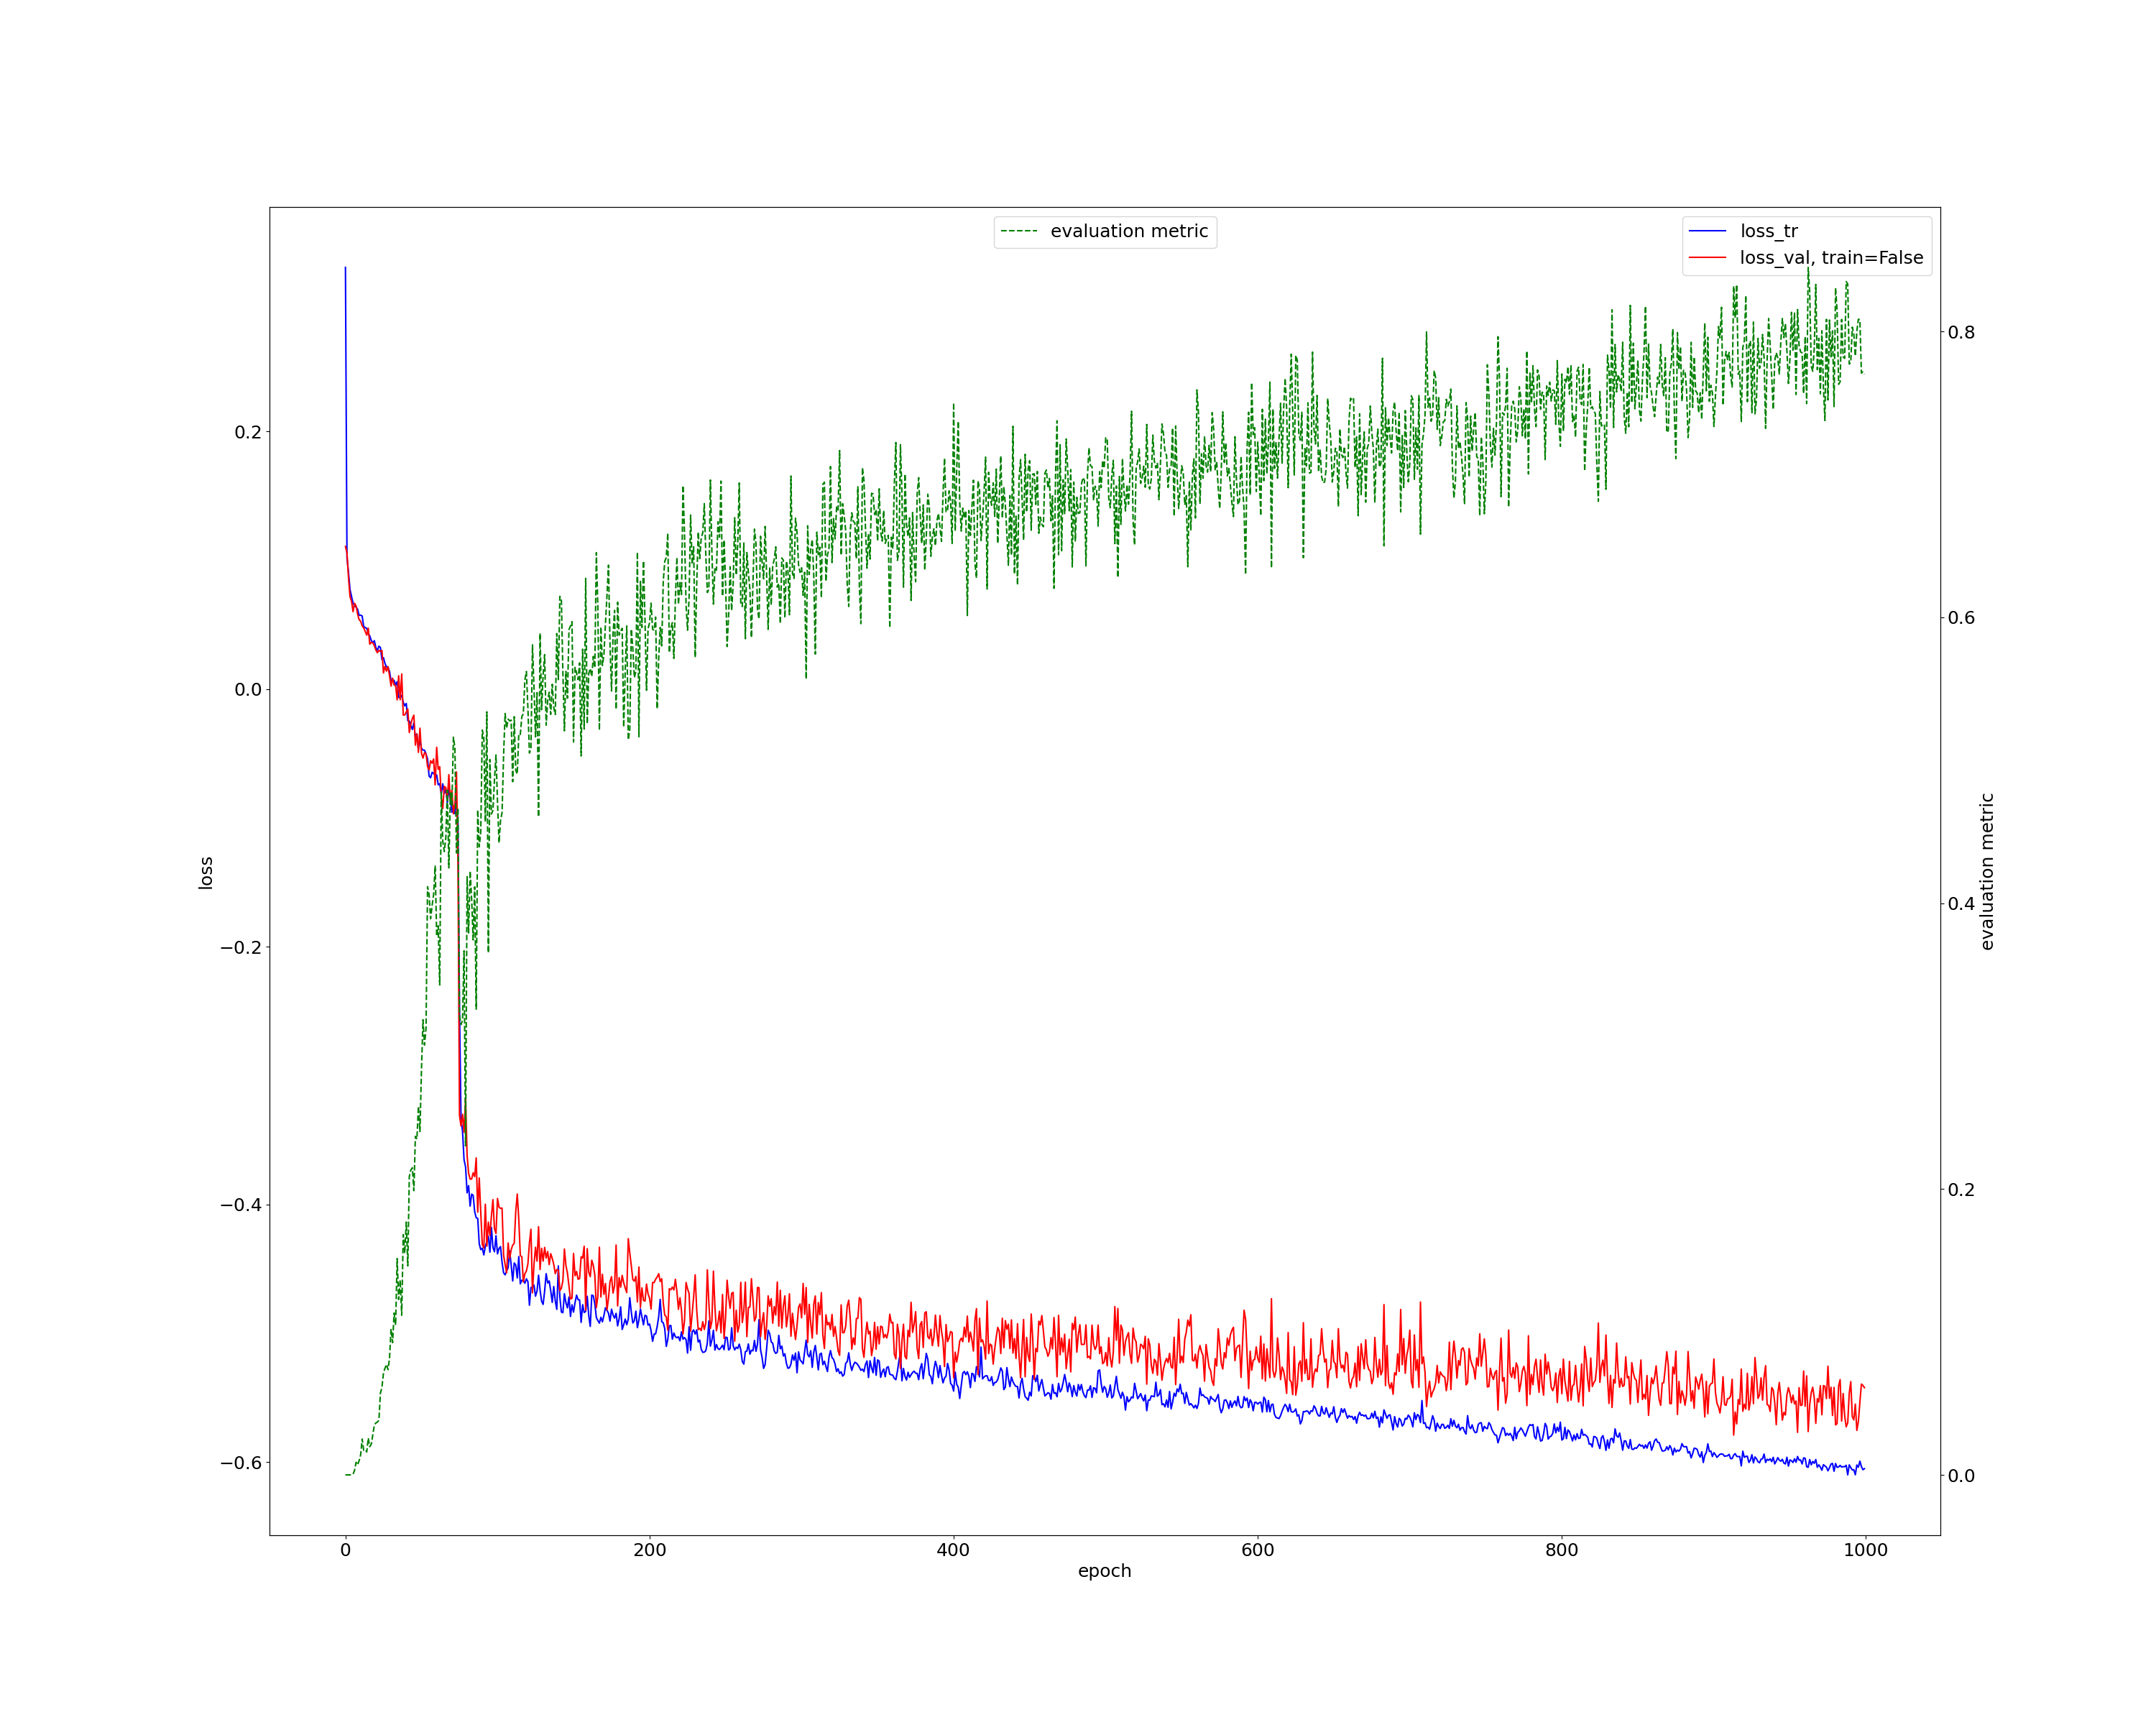}
 \\

    \rotatebox{90}{$\;\;\;\;\;\;\;\;\;\;$ Split 2}
    & \includegraphics[ width=0.45\linewidth,height=0.27\linewidth,trim={1cm 0.5cm 0.25cm 1cm},clip,]{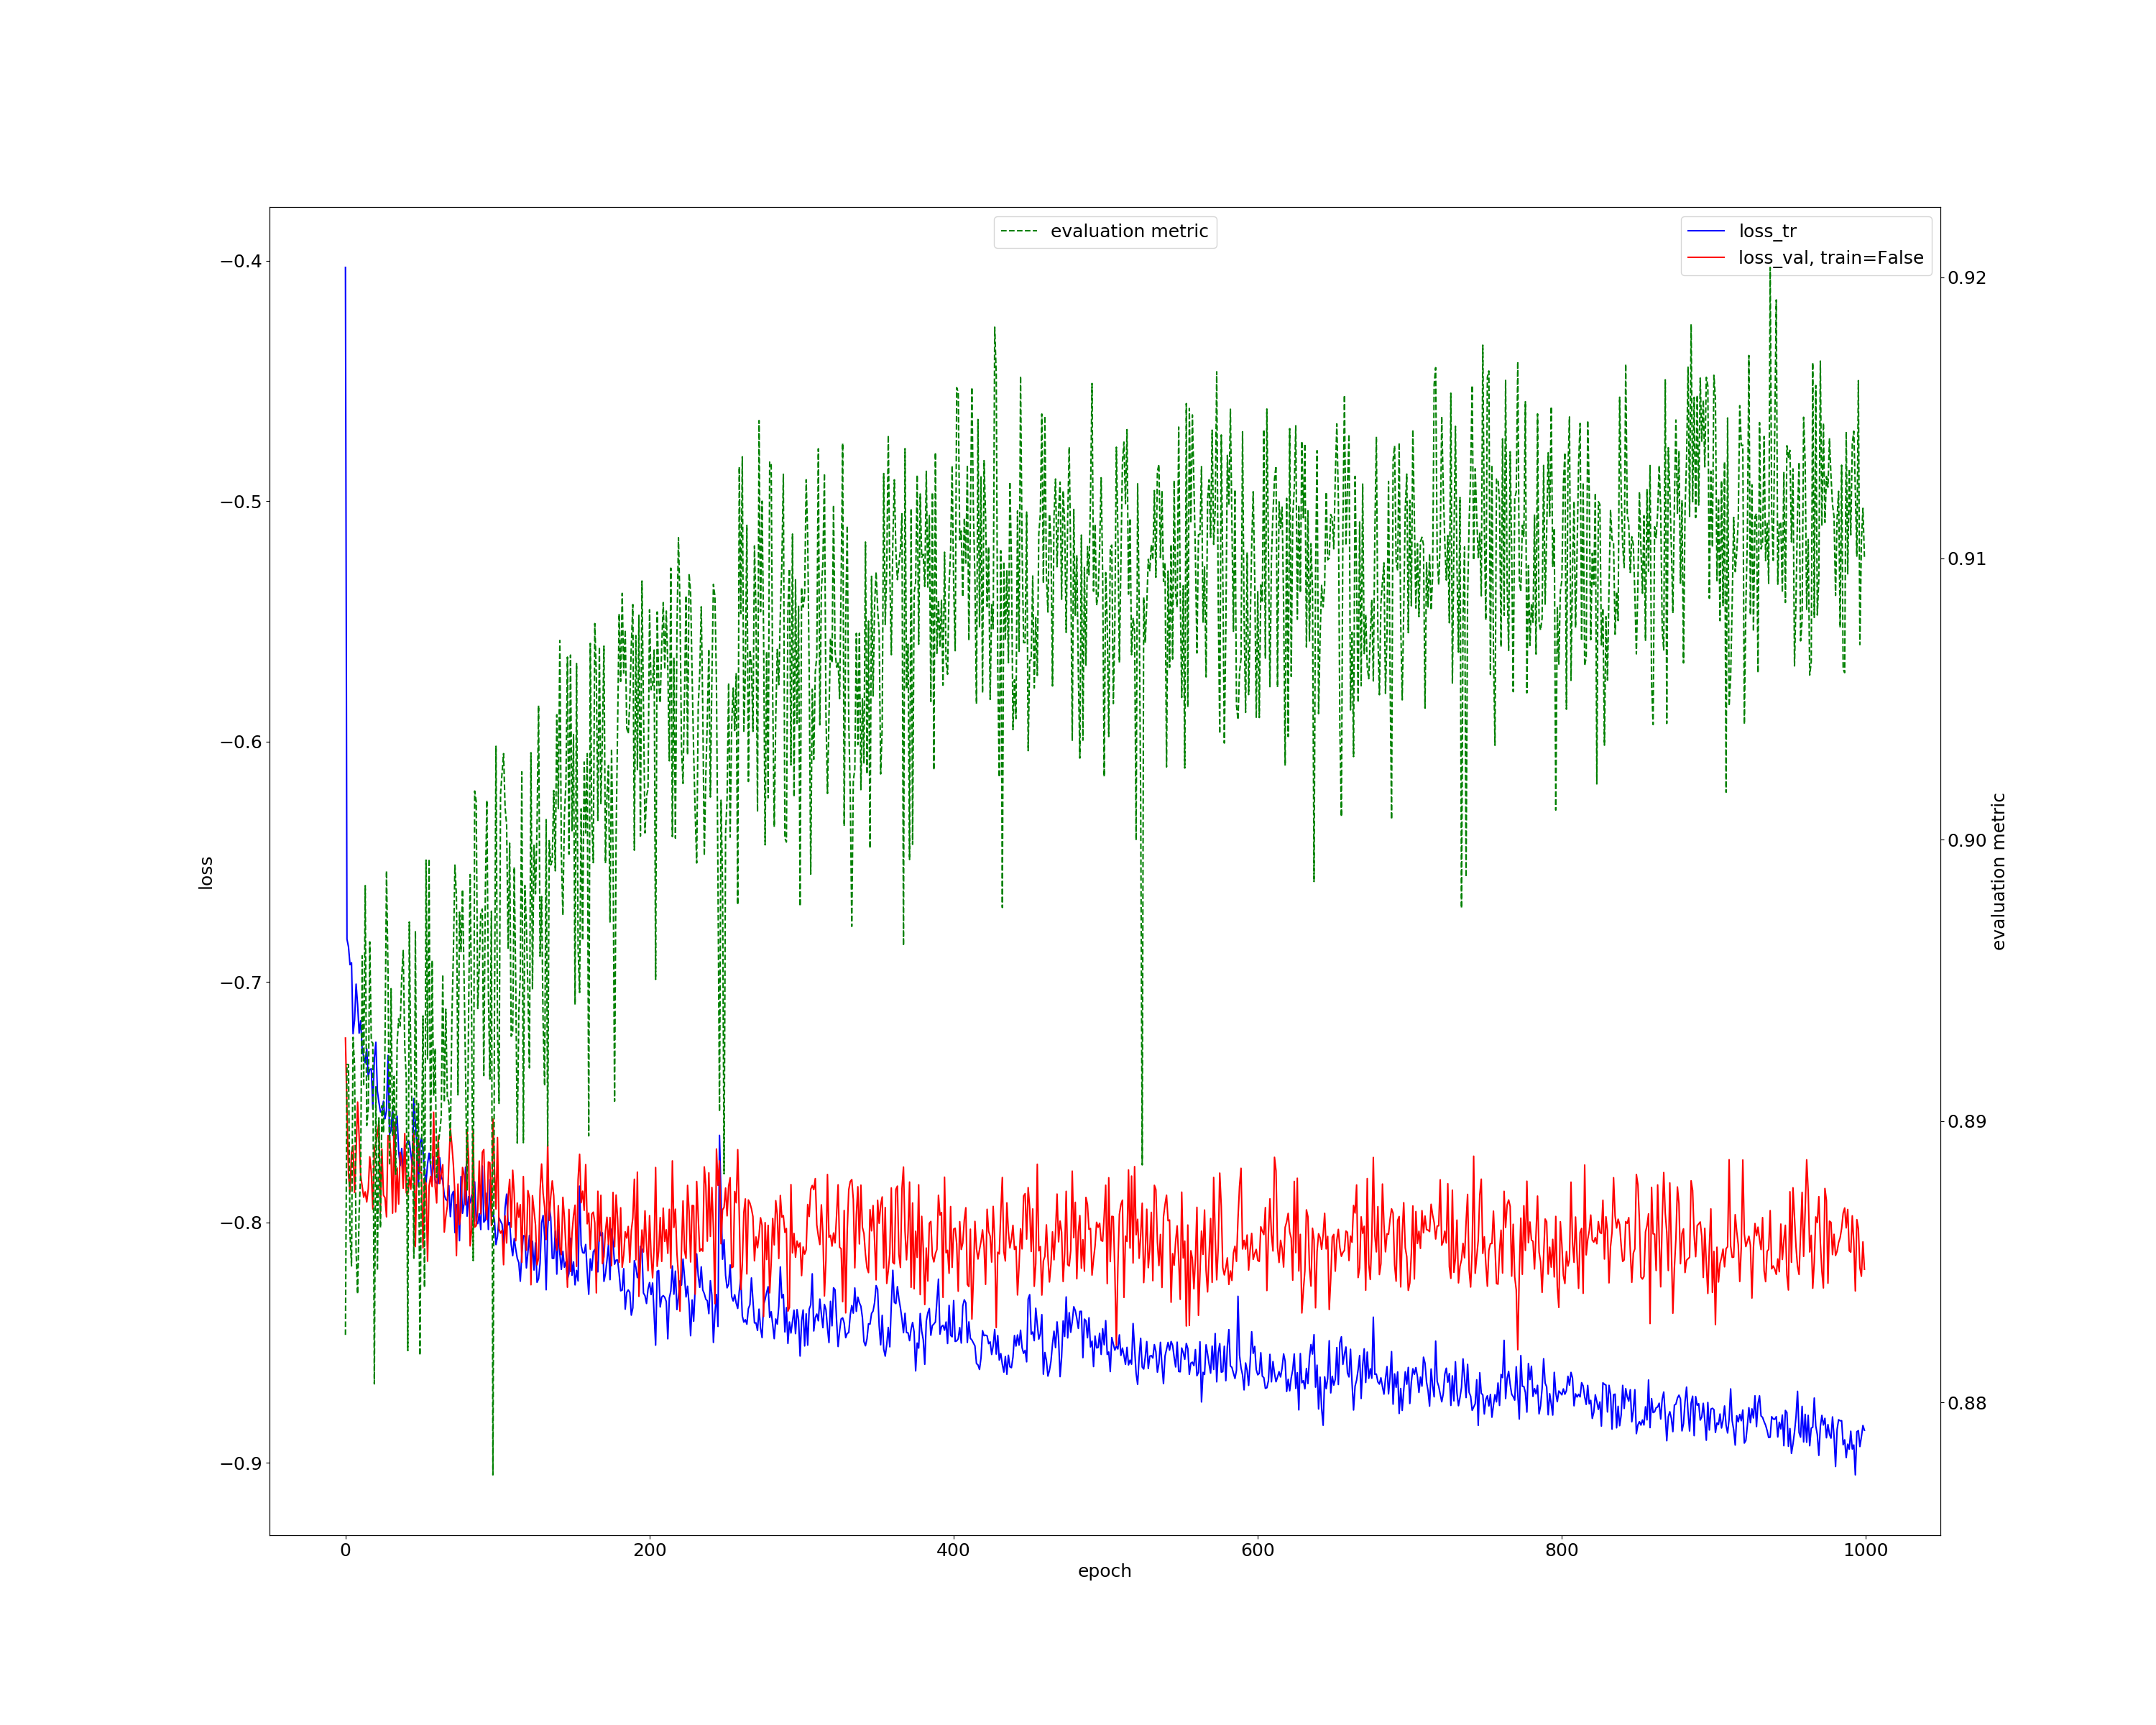}
& \includegraphics[ width=0.45\linewidth,height=0.27\linewidth,trim={1cm 0.5cm 0.25cm 1cm},clip,]{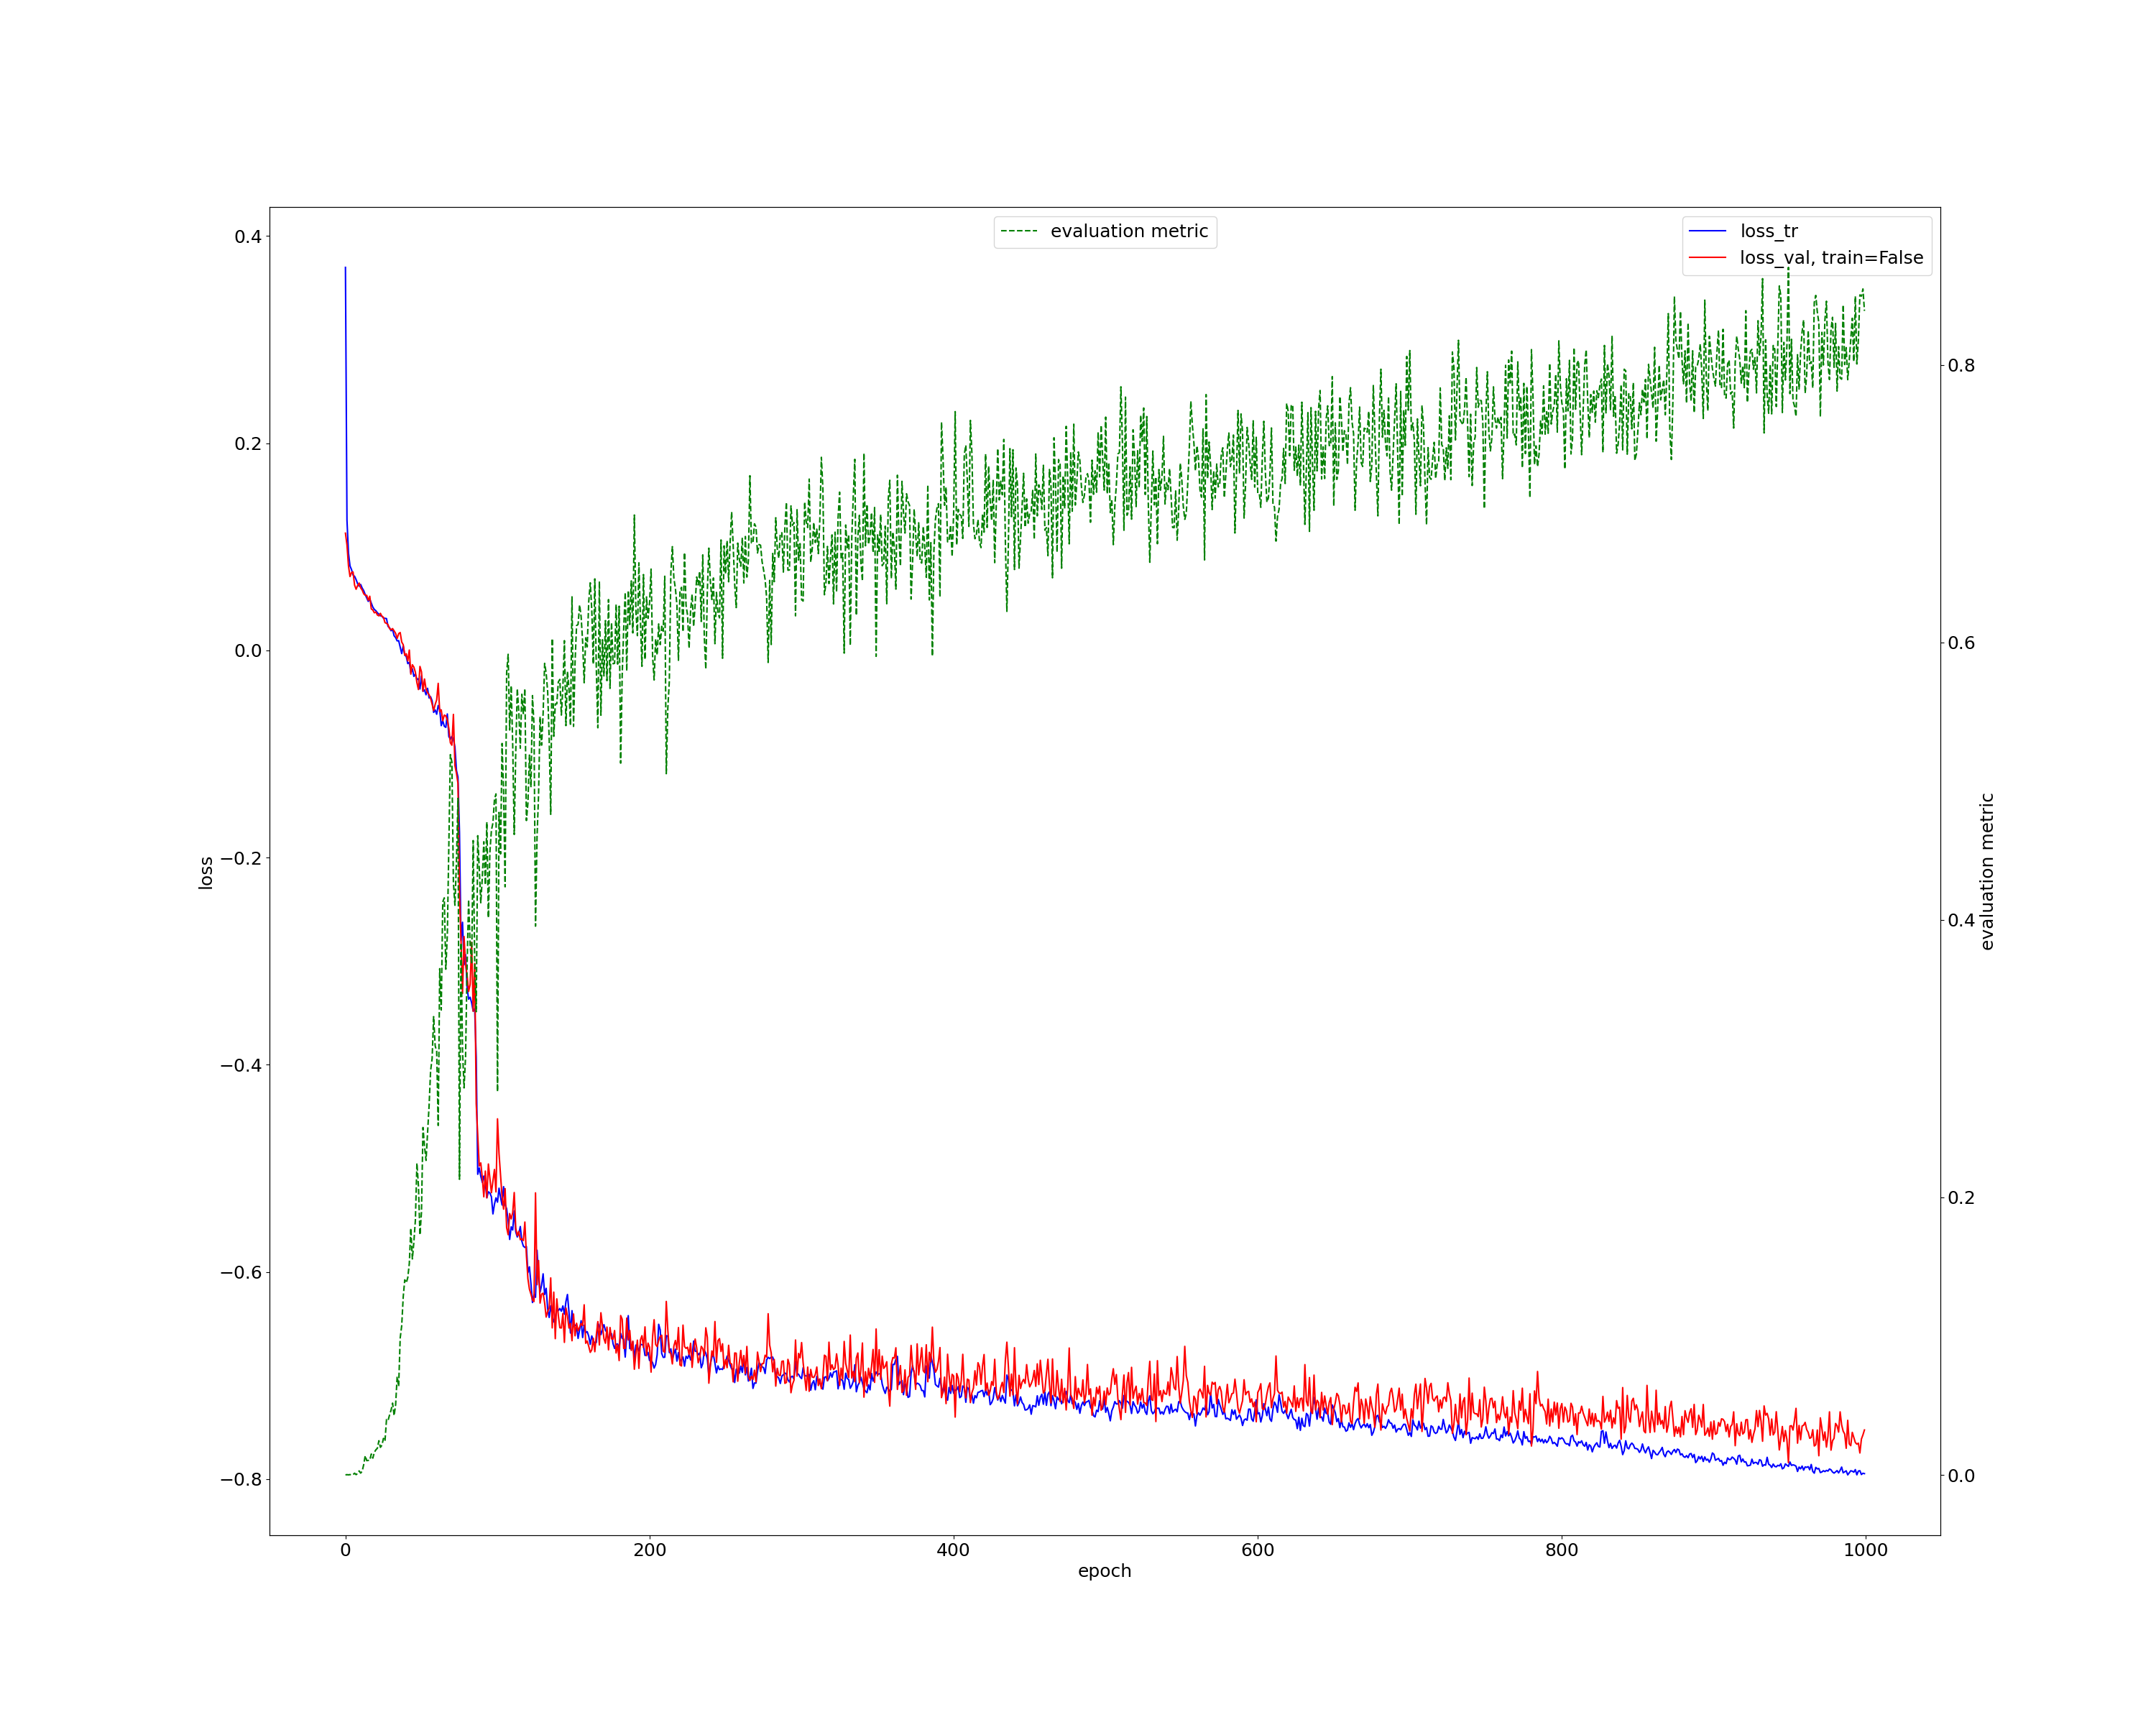}

 \\

    \rotatebox{90}{$\;\;\;\;\;\;\;\;\;\;$ Split 3}
    & \includegraphics[ width=0.45\linewidth,height=0.27\linewidth,trim={1cm 0.5cm 0.25cm 1cm},clip,]{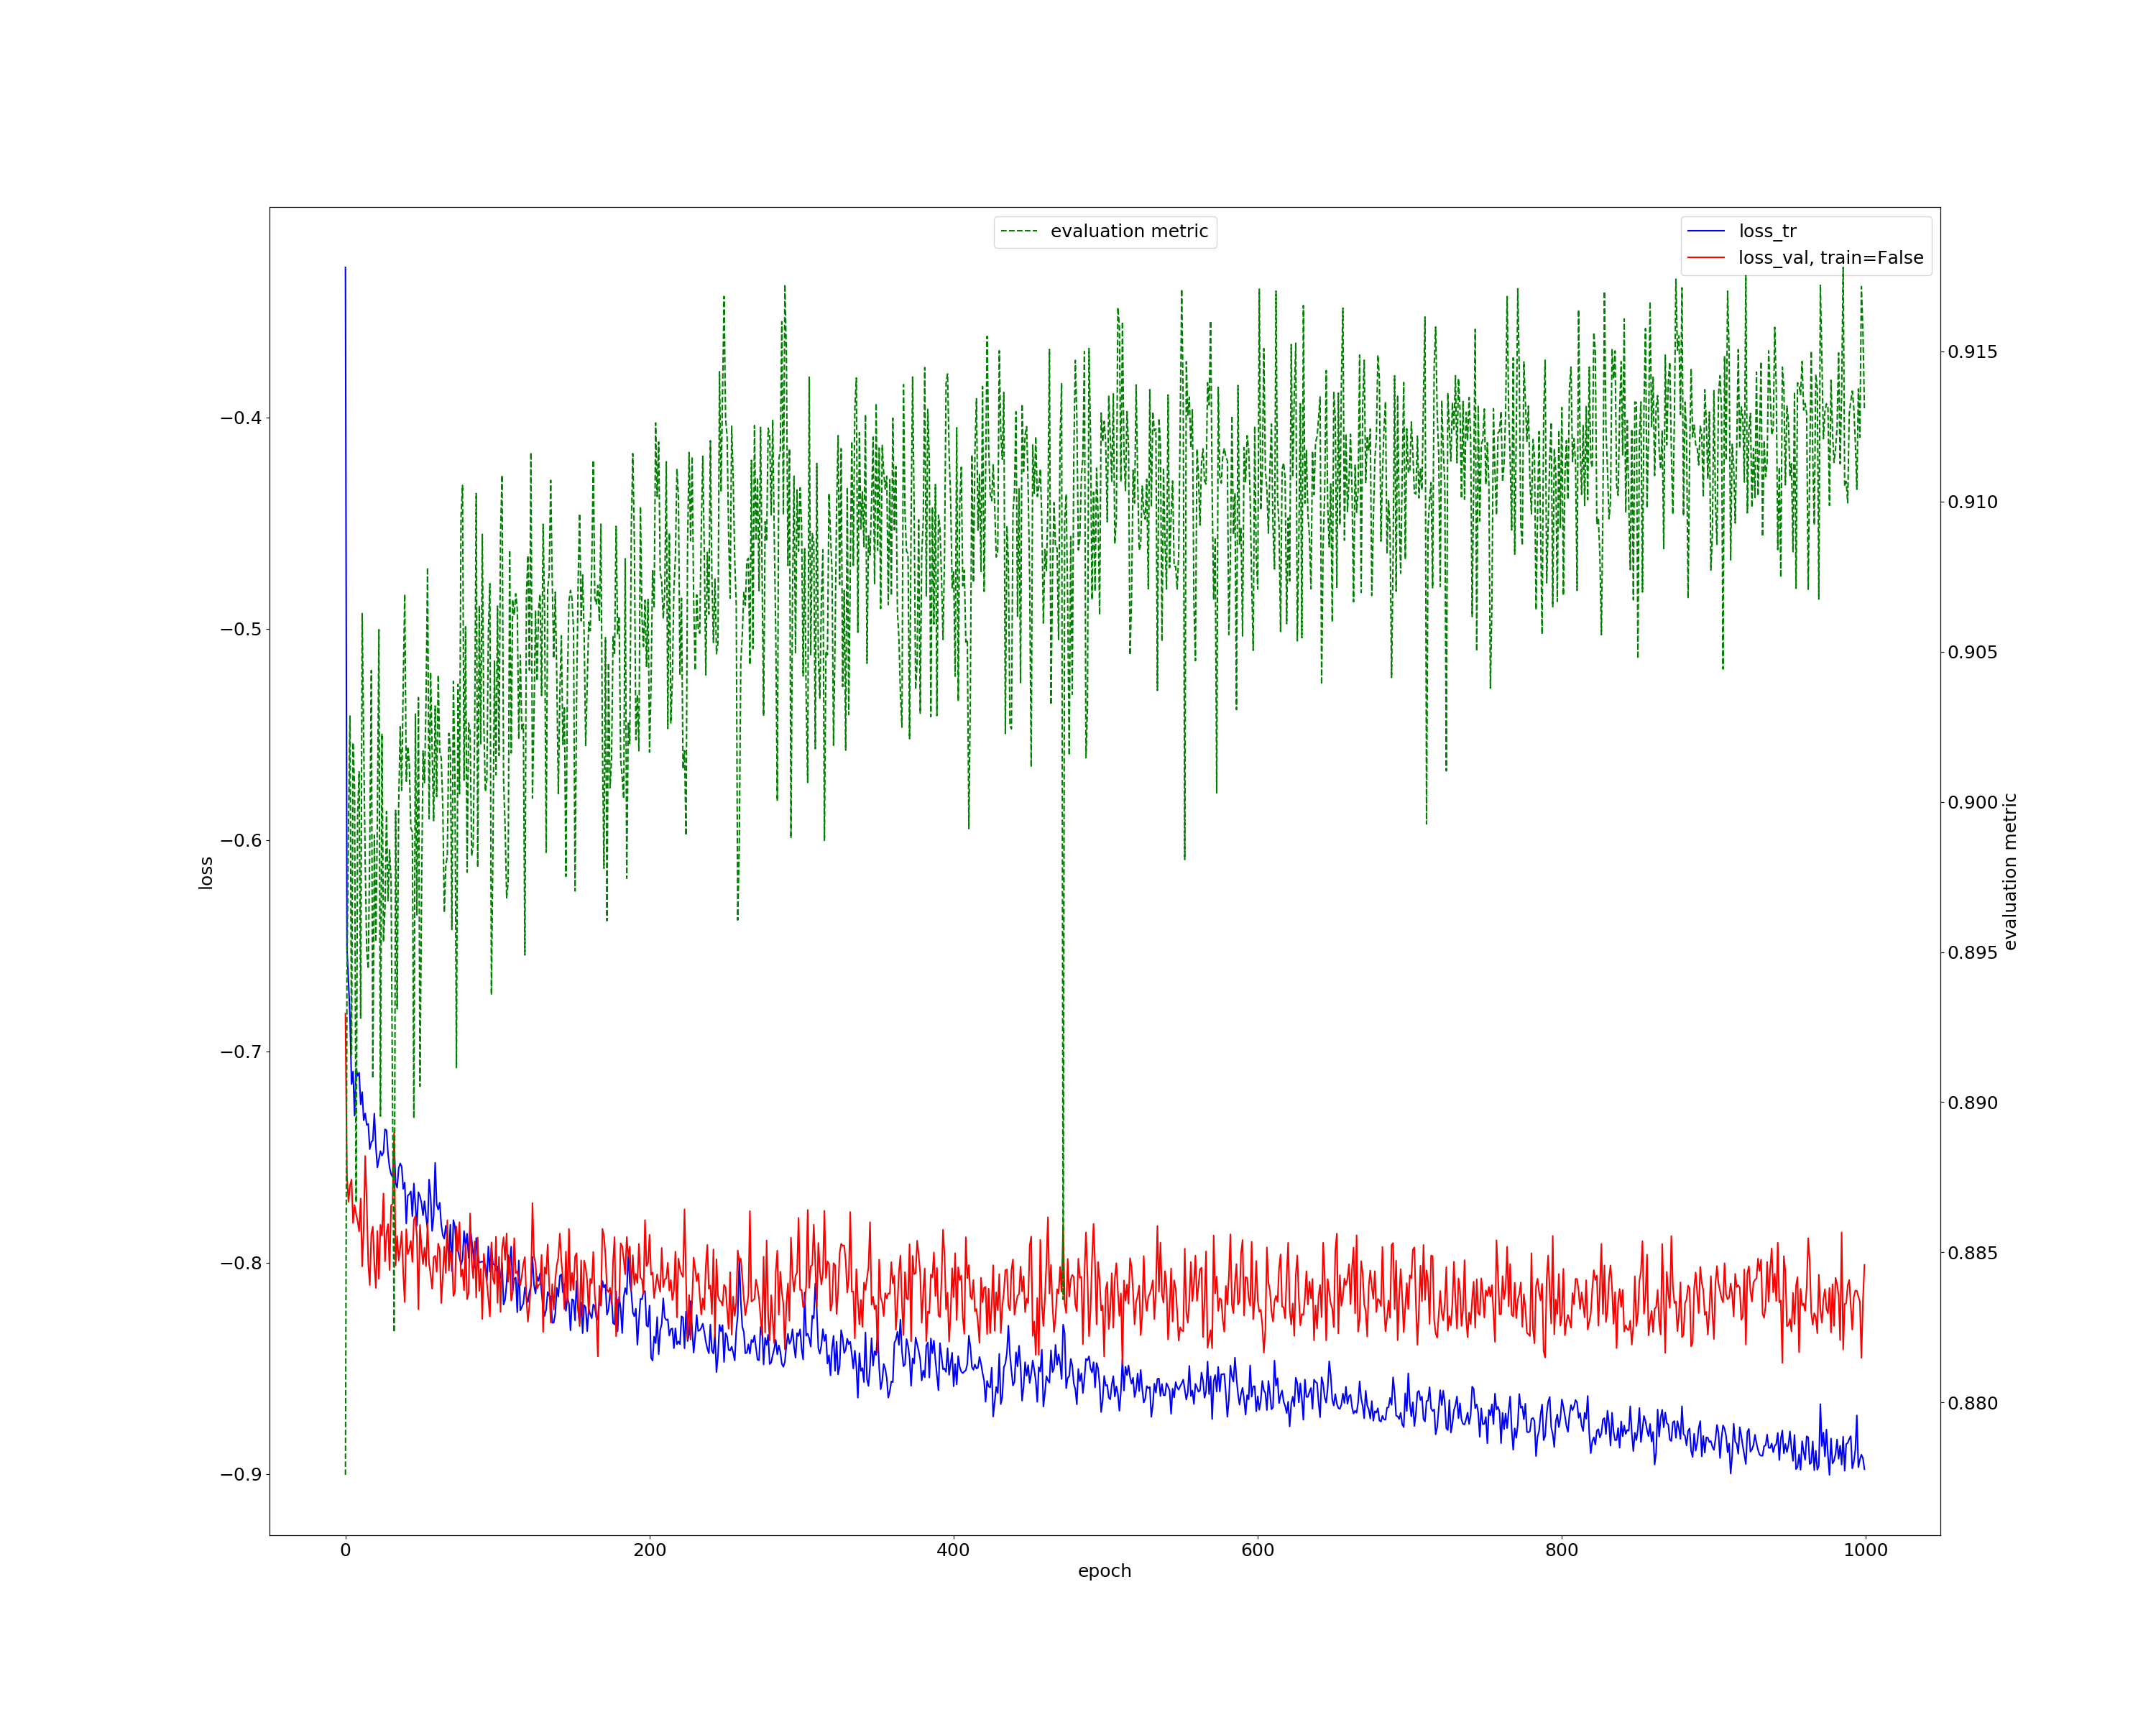}
& \includegraphics[ width=0.45\linewidth,height=0.27\linewidth,trim={1cm 0.5cm 0.25cm 1cm},clip,]{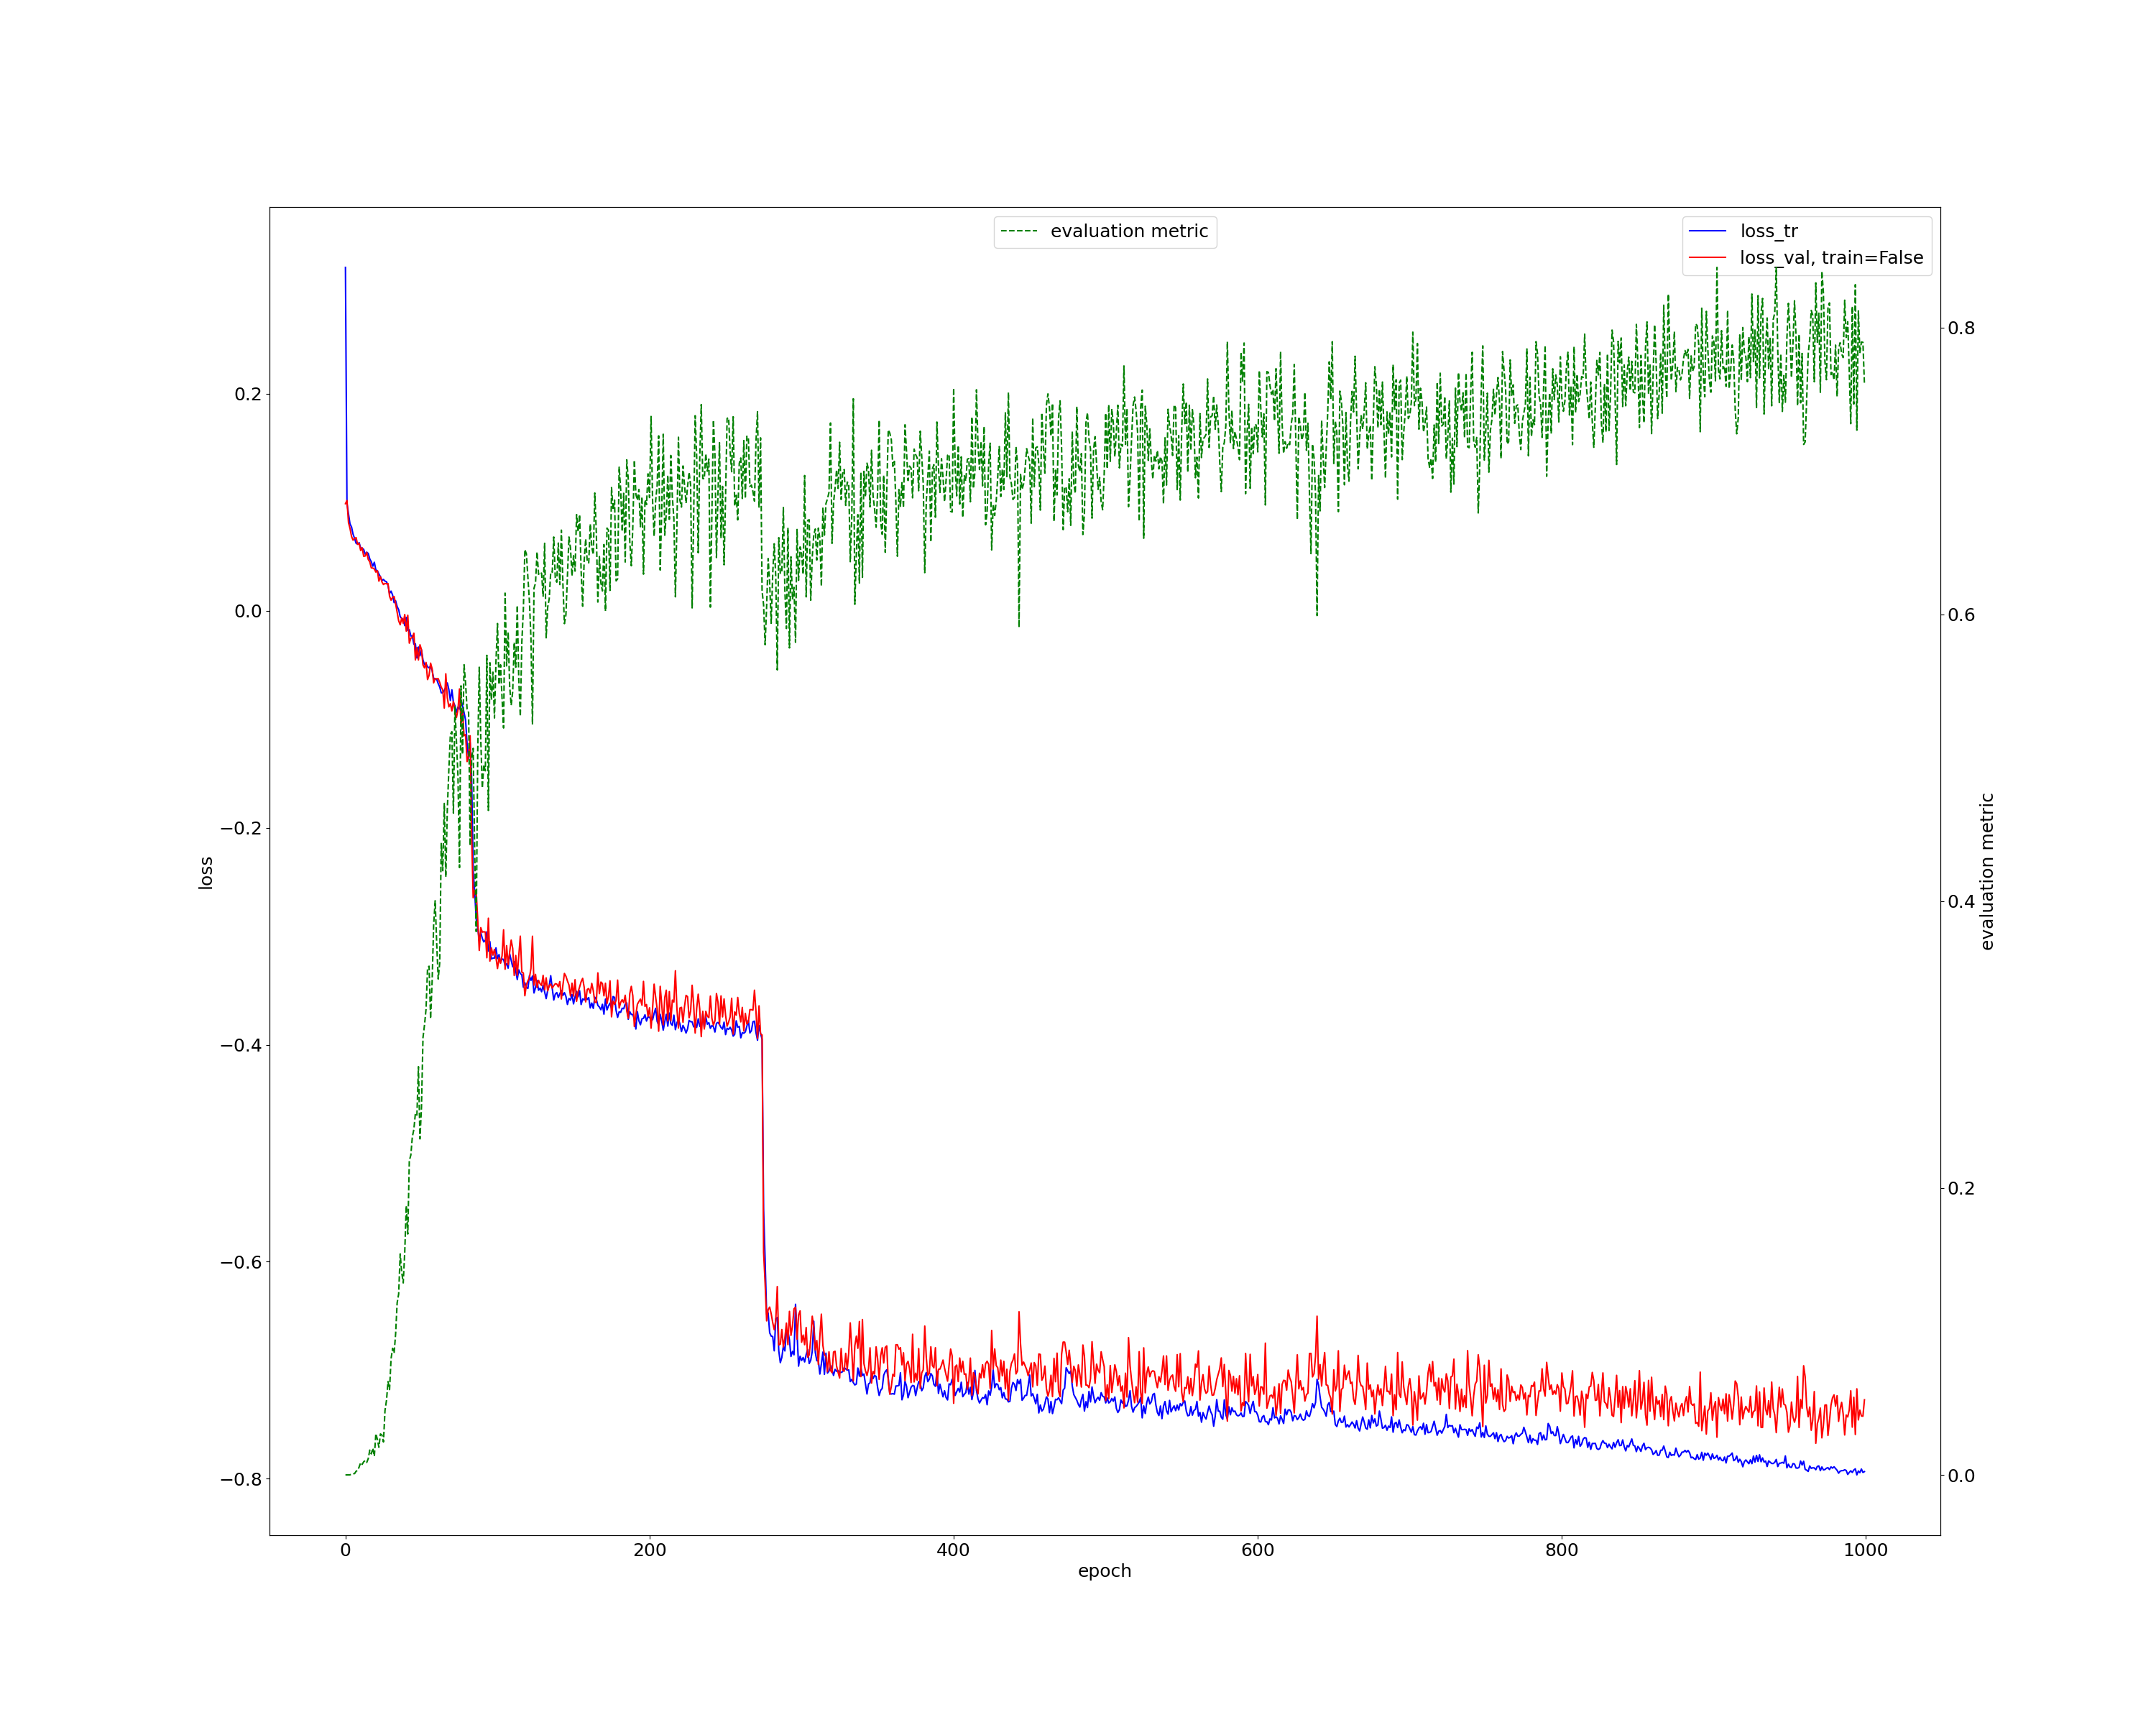}

\\

    \rotatebox{90}{$\;\;\;\;\;\;\;\;\;\;$ Split 4}
    & \includegraphics[ width=0.45\linewidth,height=0.27\linewidth,trim={1cm 0.5cm 0.25cm 1cm},clip,]{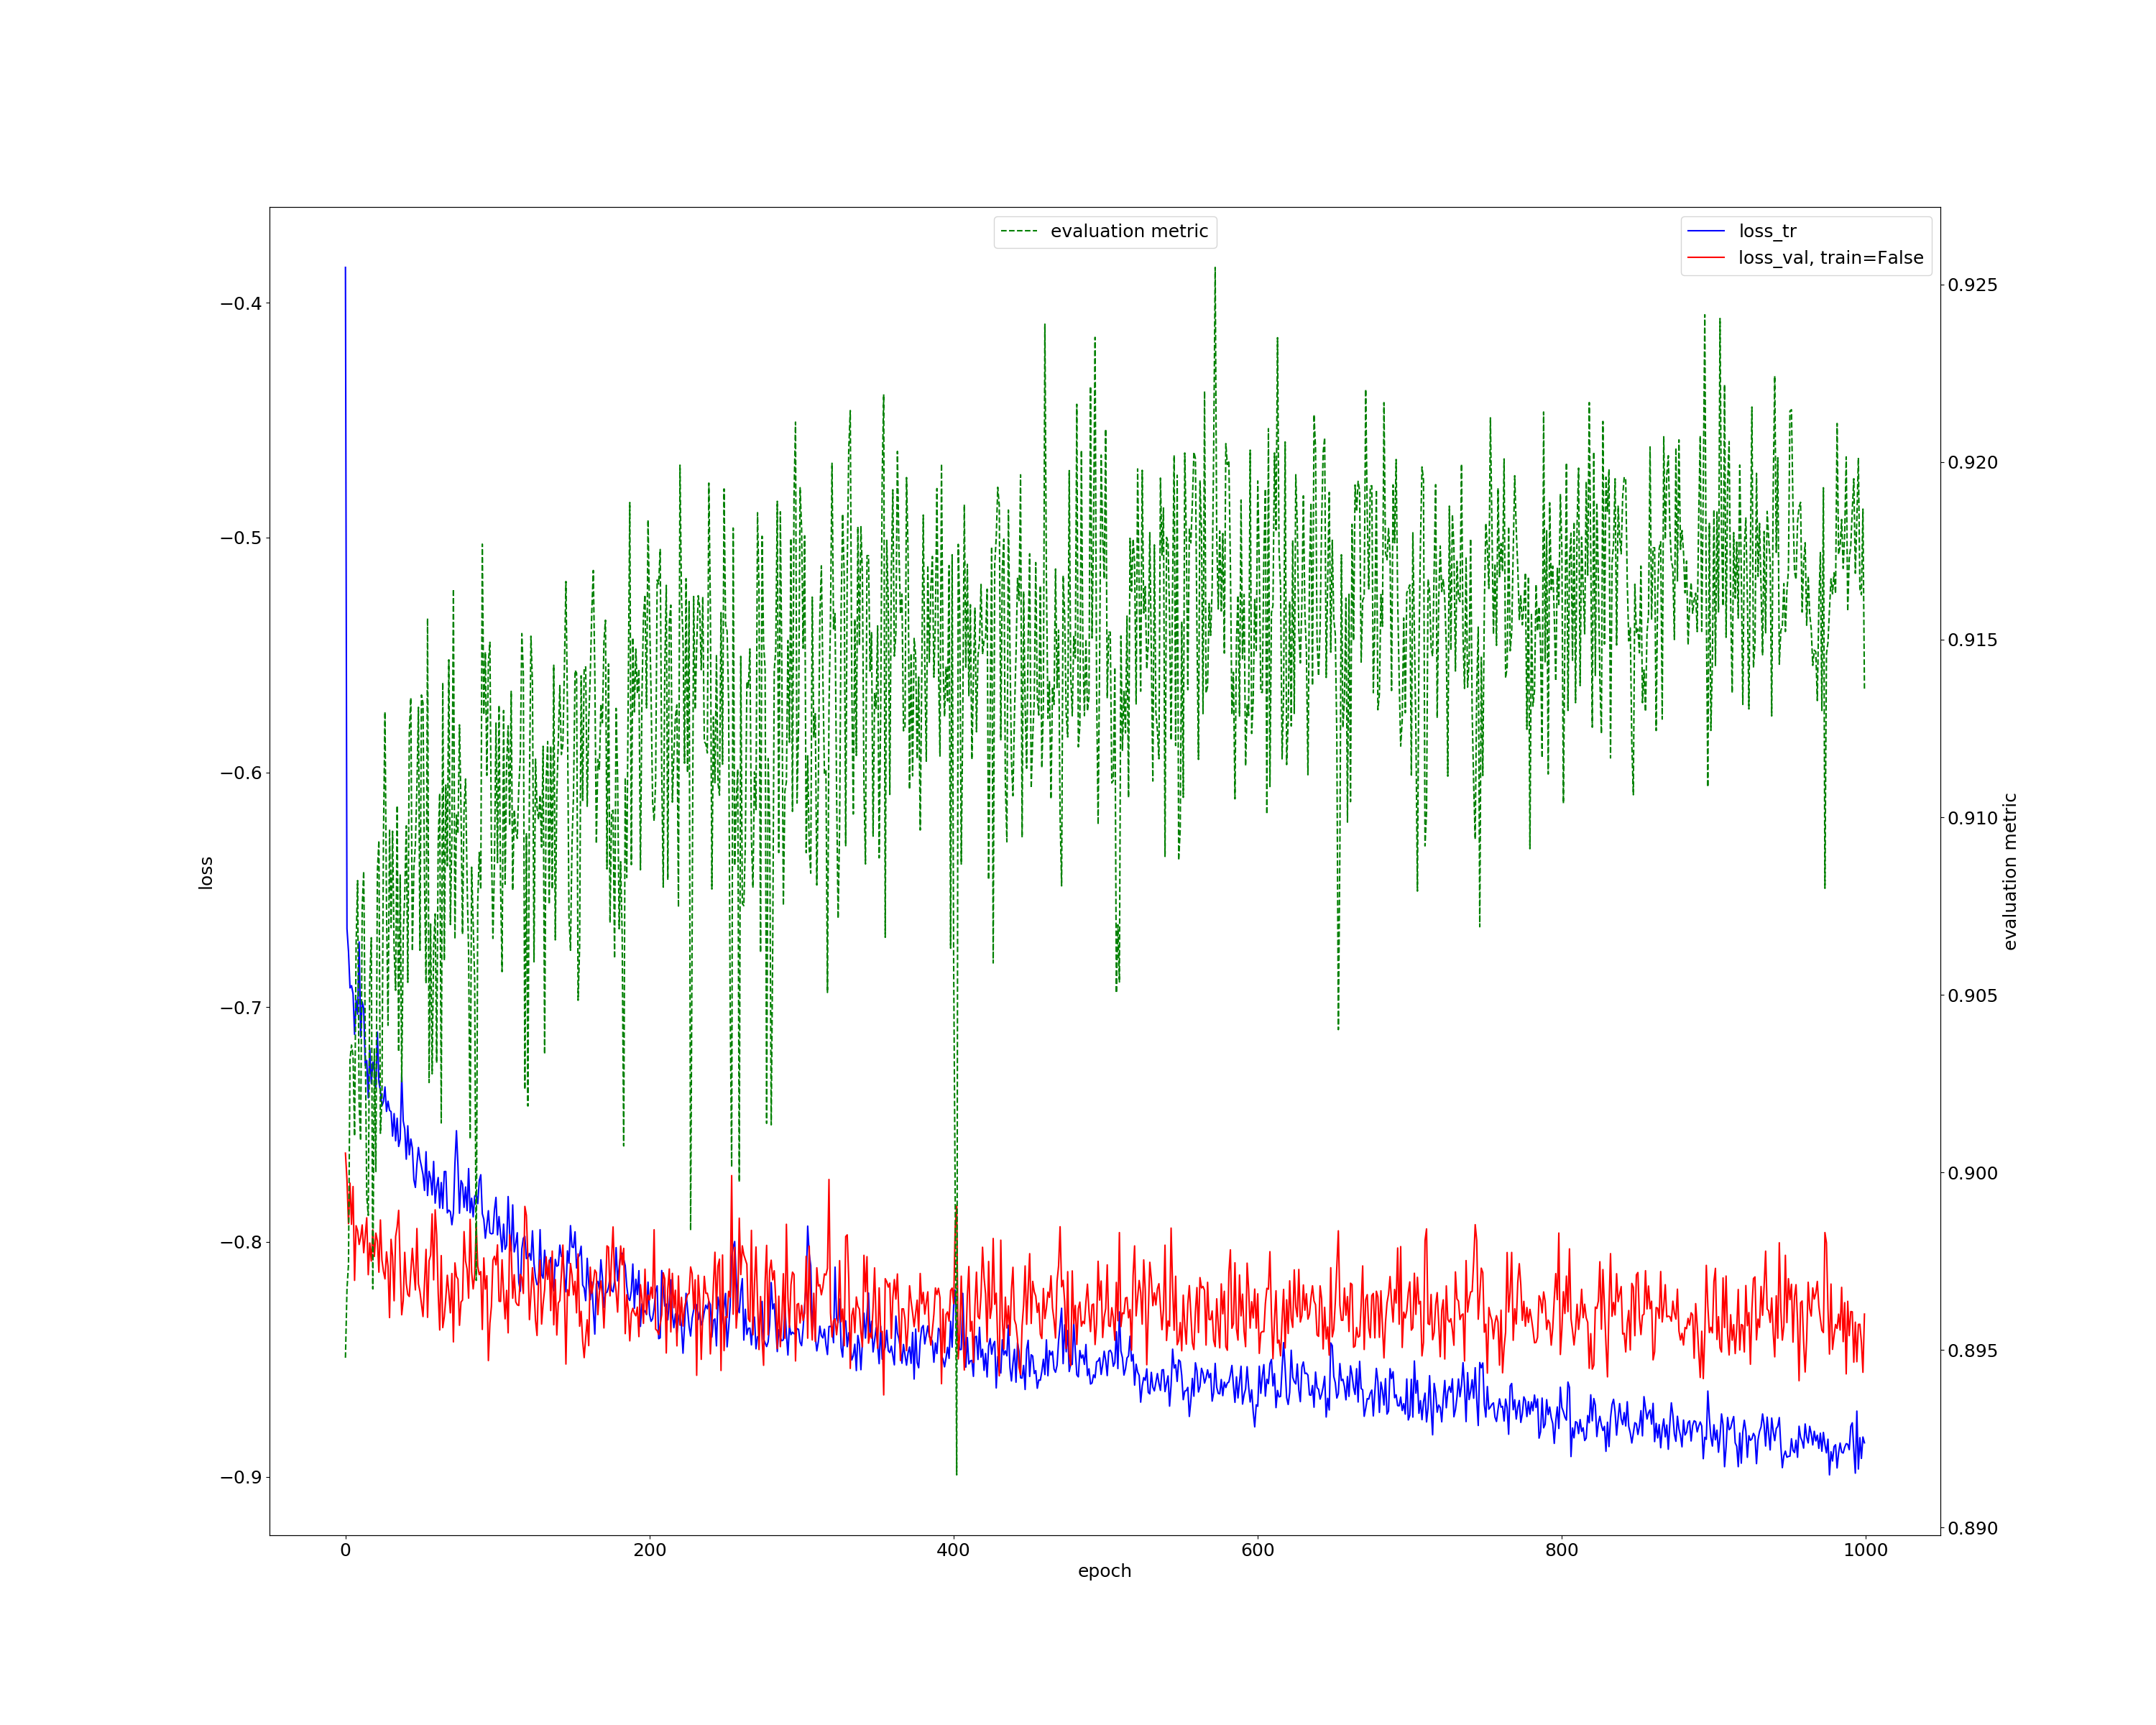}
& \includegraphics[width=0.45\linewidth,height=0.27\linewidth,trim={1cm 0.5cm 0.25cm 1cm},clip,]{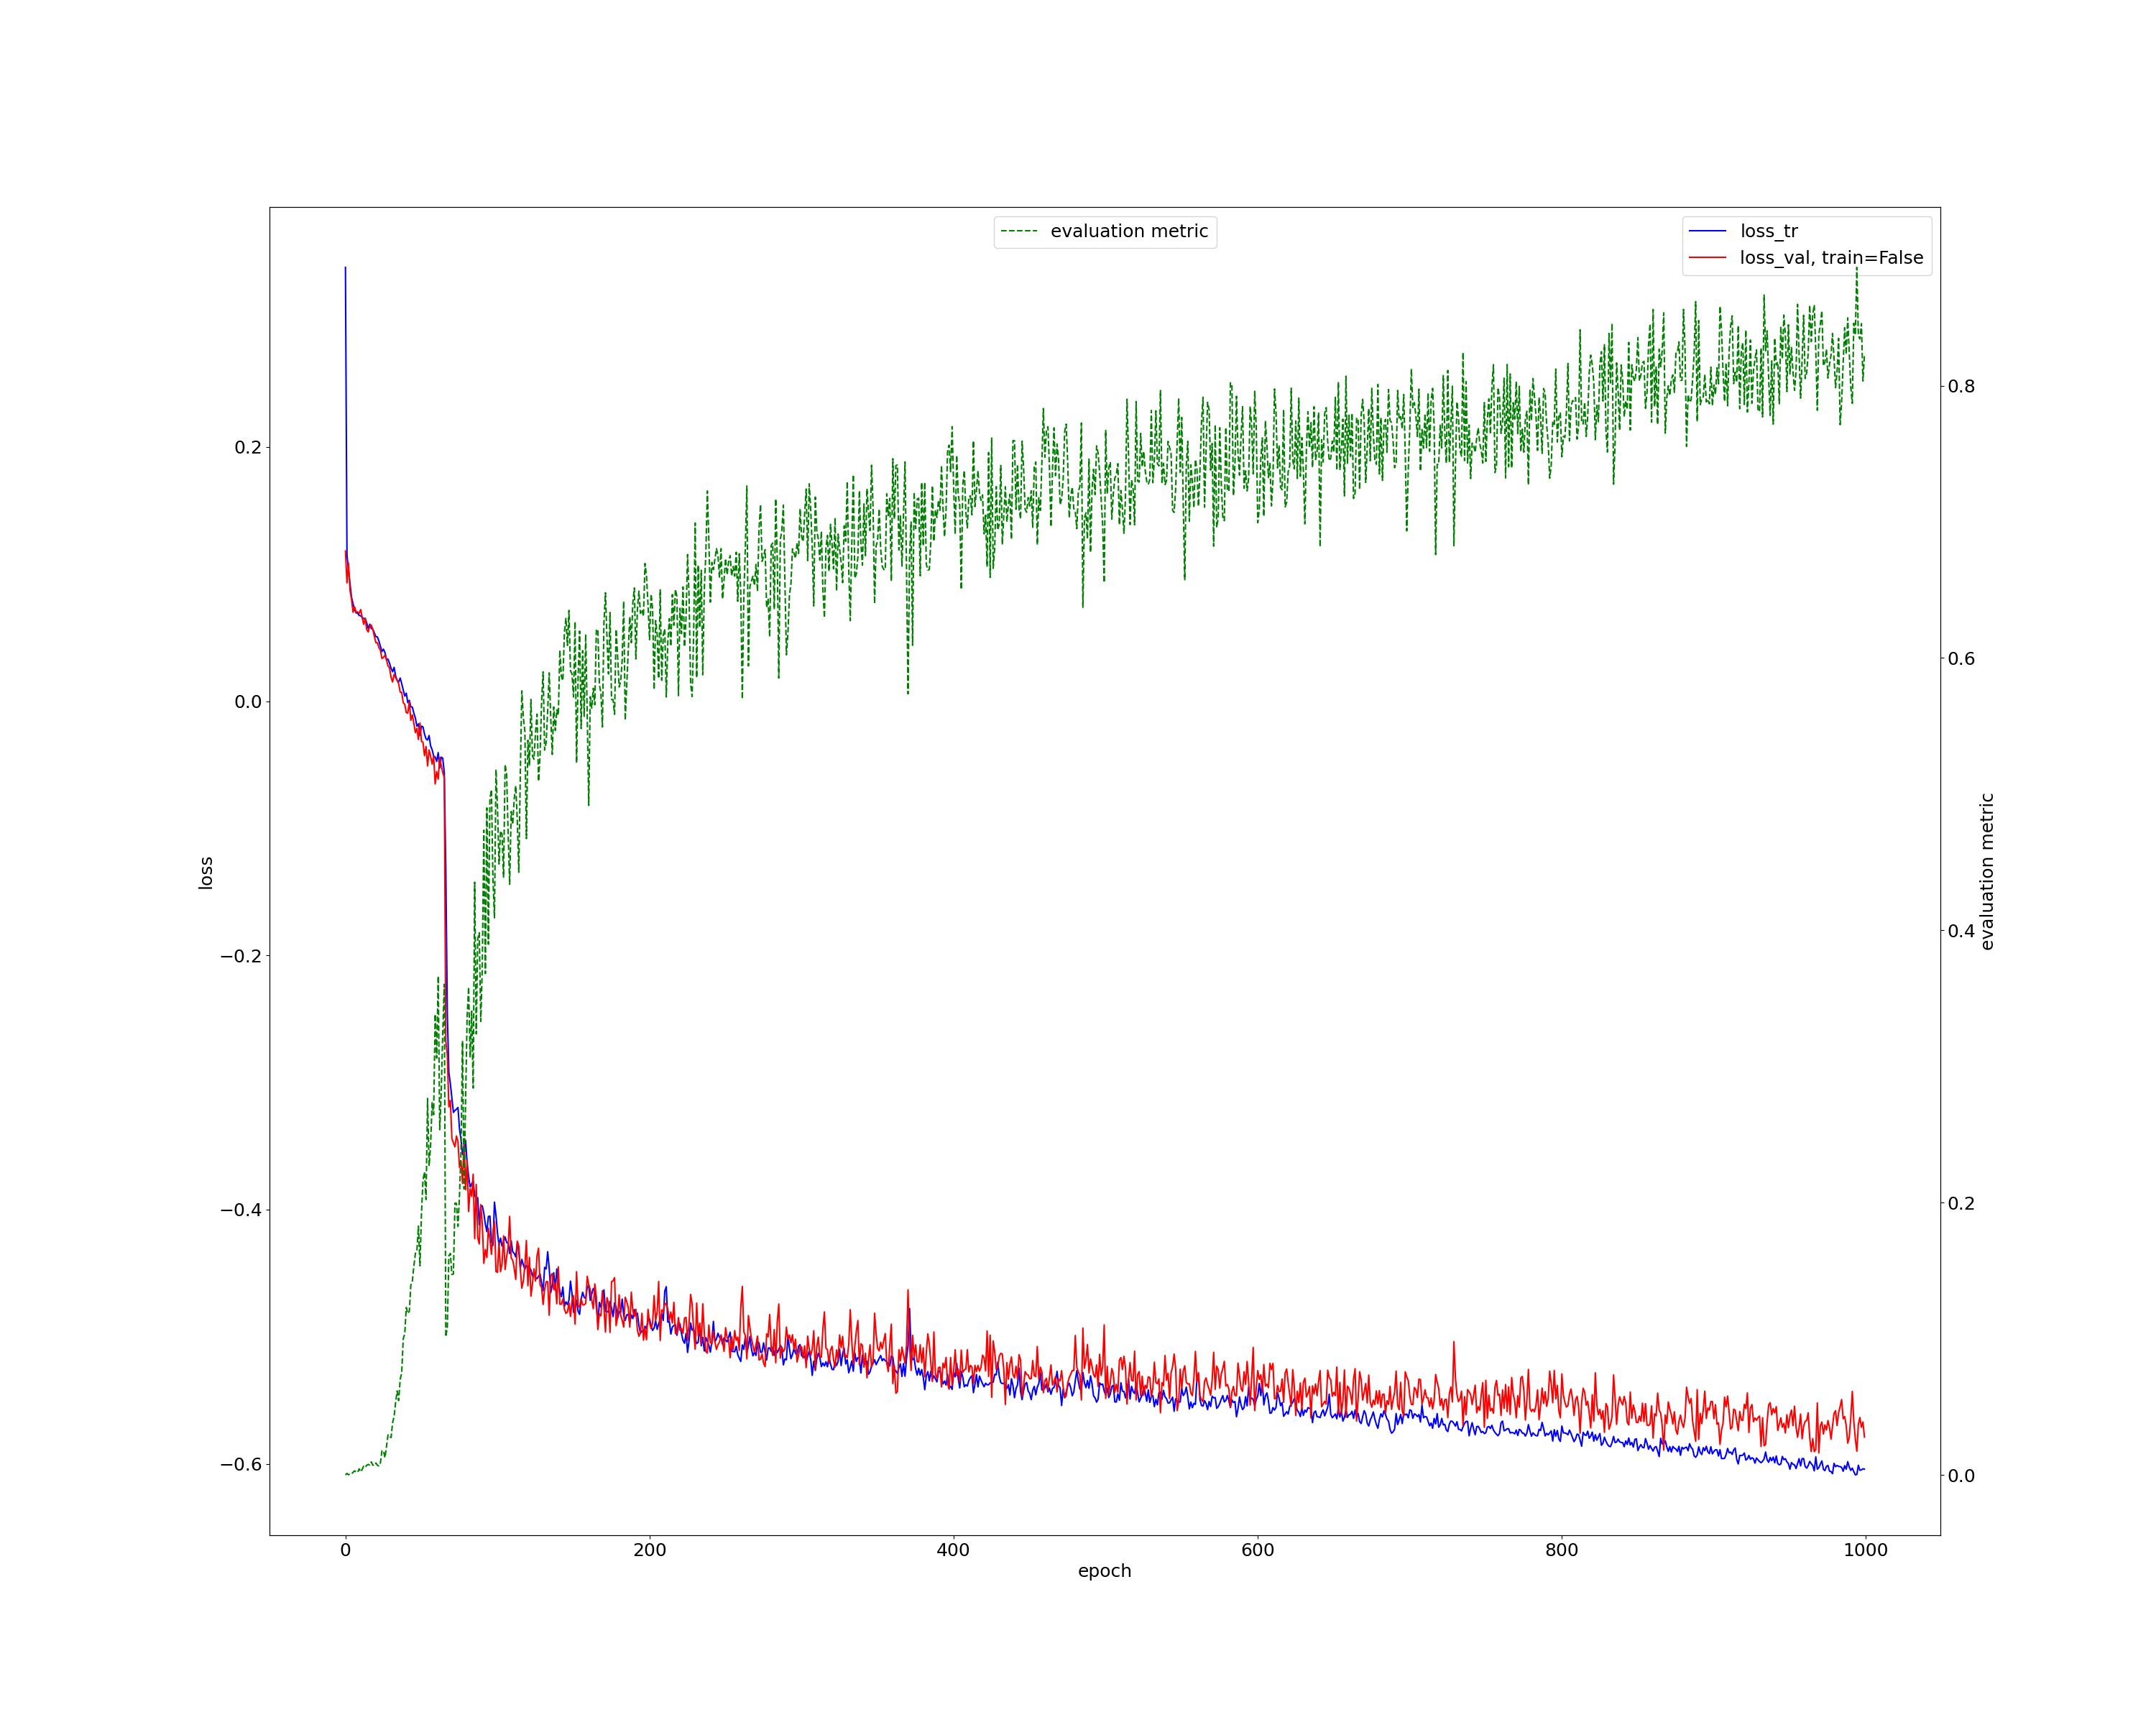}

\\

 \bottomrule
 
    \end{tabular}
    \caption{Visualization of training (Blue) and validation (Red) losses as well as validation performance (Green). For SegThor, the final validation performance ranges between 0.91 and 0.93 across all splits. For Verse, the final validation performance ranges between 0.82 and 0.84 across all splits. }
    \label{fig:training}
\end{figure*}
