# Supplementary material for: Detailed Annotations of Chest X-Rays via CT Projection for Report Understanding
Source: arXiv:2210.03416 source file (2022-10-07)
Supplement: Supplementary file 4 [file dataset.tex]

\setlength{\tabcolsep}{2pt}

\begin{figure}[h]
    \centering
        \begin{tabular}{cccccc}
        \toprule
         & Input & Lungs & Mediastinum & Bones & Sub-Diaphragm  \\
         \midrule
         \multirow{3}{*}{\rotatebox{90}{Frontal}} & 
         \includegraphics[width=0.18\linewidth,height=0.18\linewidth]{images/supplementary_dataset_examples/9_frontal.jpg}&
         \includegraphics[width=0.18\linewidth,height=0.18\linewidth]{images/supplementary_dataset_examples/9_lung_frontal.jpg}&
         \includegraphics[width=0.18\linewidth,height=0.18\linewidth]{images/supplementary_dataset_examples/9_mediastinum_frontal.jpg}&
         \includegraphics[width=0.18\linewidth,height=0.18\linewidth]{images/supplementary_dataset_examples/9_bones_frontal.jpg}&
         \includegraphics[width=0.18\linewidth,height=0.18\linewidth]{images/supplementary_dataset_examples/9_diaphragm_frontal.jpg}\\
         & 
         \includegraphics[width=0.18\linewidth,height=0.18\linewidth]{images/supplementary_dataset_examples/12_frontal.jpg}&
         \includegraphics[width=0.18\linewidth,height=0.18\linewidth]{images/supplementary_dataset_examples/12_lung_frontal.jpg}&
         \includegraphics[width=0.18\linewidth,height=0.18\linewidth]{images/supplementary_dataset_examples/12_mediastinum_frontal.jpg}&
         \includegraphics[width=0.18\linewidth,height=0.18\linewidth]{images/supplementary_dataset_examples/12_bones_frontal.jpg}&
         \includegraphics[width=0.18\linewidth,height=0.18\linewidth]{images/supplementary_dataset_examples/12_diaphragm_frontal.jpg}\\
         \midrule
         \multirow{3}{*}{\rotatebox{90}{Lateral}} & 
         \includegraphics[width=0.18\linewidth,height=0.18\linewidth]{images/supplementary_dataset_examples/9_lateral.jpg}&
         \includegraphics[width=0.18\linewidth,height=0.18\linewidth]{images/supplementary_dataset_examples/9_lung_lateral.jpg}&
         \includegraphics[width=0.18\linewidth,height=0.18\linewidth]{images/supplementary_dataset_examples/9_mediastinum_lateral.jpg}&
         \includegraphics[width=0.18\linewidth,height=0.18\linewidth]{images/supplementary_dataset_examples/9_bones_lateral.jpg}&
         \includegraphics[width=0.18\linewidth,height=0.18\linewidth]{images/supplementary_dataset_examples/9_diaphragm_lateral.jpg}\\
         & 
         \includegraphics[width=0.18\linewidth,height=0.18\linewidth]{images/supplementary_dataset_examples/12_lateral.jpg}&
         \includegraphics[width=0.18\linewidth,height=0.18\linewidth]{images/supplementary_dataset_examples/12_lung_lateral.jpg}&
         \includegraphics[width=0.18\linewidth,height=0.18\linewidth]{images/supplementary_dataset_examples/12_mediastinum_lateral.jpg}&
         \includegraphics[width=0.18\linewidth,height=0.18\linewidth]{images/supplementary_dataset_examples/12_bones_lateral.jpg}&
         \includegraphics[width=0.18\linewidth,height=0.18\linewidth]{images/supplementary_dataset_examples/12_diaphragm_lateral.jpg}\\
         \bottomrule
    \end{tabular}
    \caption{Different ground truth annotations of our PAX-ray dataset for frontal and lateral view}
    \label{fig:supplementary_dataset_examples}
\end{figure}
