# Supplementary material for: Detailed Annotations of Chest X-Rays via CT Projection for Report Understanding
Source: arXiv:2210.03416 source file (2022-10-07)
Supplement: Supplementary file 5 [file labels.tex]

% \begin{figure}%{r}{0.5\textwidth}
% % \centering
%   \begin{tabular}{c}

%     \includegraphics[width=0.48\textwidth]{images/supplementary/labels/3_lobes_frontal.jpg}
%     \\
%     text
%     \\
%     \includegraphics[width=0.48\textwidth]{images/supplementary/labels/3_mediastinum_lateral.jpg}
%     \\
%     text
%     \\
%     \includegraphics[width=0.48\textwidth]{images/supplementary/labels/3_heart_frontal.jpg}
%     \\
%     text
%     \\
%     \includegraphics[width=0.48\textwidth]{images/supplementary/labels/3_heart_lateral.jpg}
%     \\
%     text
%     \\
%     \includegraphics[width=0.48\textwidth]{images/supplementary/labels/3_vessels_frontal.jpg}
%     \\
%     text
%     \\
%     \includegraphics[width=0.48\textwidth]{images/supplementary/labels/3_cervical_frontal.jpg}
%     \\
%     text
%     \\
%     \includegraphics[width=0.48\textwidth]{images/supplementary/labels/3_cervical_lateral.jpg}
%     \\
%     text
%     \\
%     \includegraphics[width=0.48\textwidth]{images/supplementary/labels/3_thoracic_frontal.jpg}
%     \\
%     text
%     \\
%     \includegraphics[width=0.48\textwidth]{images/supplementary/labels/3_thoracic_lateral.jpg}
%     \\
%     text
%     \\
%     \includegraphics[width=0.48\textwidth]{images/supplementary/labels/3_lumbar_frontal.jpg}
%     \\
%     text
%     \\
%     \includegraphics[width=0.48\textwidth]{images/supplementary/labels/3_lumbar_lateral.jpg}
%     \\
%     text
%     \\
%     \includegraphics[width=0.48\textwidth]{images/supplementary/labels/3_ribs_frontal.jpg}
%     \\
%     text
%     \\
%     \includegraphics[width=0.48\textwidth]{images/supplementary/labels/3_rib_lateral.jpg}
%       \end{tabular}

%   \caption{Birds}
% \end{figure}
