# Supplementary material for: Detailed Annotations of Chest X-Rays via CT Projection for Report Understanding
Source: arXiv:2210.03416 source file (2022-10-07)
Supplement: Supplementary file 6 [file preds_and_gts.tex]

\setlength{\tabcolsep}{2pt}

\begin{figure*}[t]
    \centering
        \begin{tabular}{cccccc}
        \toprule
         & Input & Lungs & Mediastinum & Bones & Sub-Diaphragm  \\
         \midrule
         \multirow{3}{*}{\rotatebox{90}{Frontal}} & 
         \includegraphics[width=0.17\linewidth,height=0.17\linewidth]{images/supplementary_label_examples/15_frontal.png}&
         \includegraphics[width=0.17\linewidth,height=0.17\linewidth]{images/supplementary_label_examples/15_frontal_lung.png}&
         \includegraphics[width=0.17\linewidth,height=0.17\linewidth]{images/supplementary_label_examples/15_frontal_mediastinum.png}&
         \includegraphics[width=0.17\linewidth,height=0.17\linewidth]{images/supplementary_label_examples/15_frontal_bones.png}&
         \includegraphics[width=0.17\linewidth,height=0.17\linewidth]{images/supplementary_label_examples/15_frontal_diaphragm.png}\\
         & 
         \includegraphics[width=0.17\linewidth,height=0.17\linewidth]{images/supplementary_label_examples/14_frontal.png}&
         \includegraphics[width=0.17\linewidth,height=0.17\linewidth]{images/supplementary_label_examples/14_frontal_lung.png}&
         \includegraphics[width=0.17\linewidth,height=0.17\linewidth]{images/supplementary_label_examples/14_frontal_mediastinum.png}&
         \includegraphics[width=0.17\linewidth,height=0.17\linewidth]{images/supplementary_label_examples/14_frontal_bones.png}&
         \includegraphics[width=0.17\linewidth,height=0.17\linewidth]{images/supplementary_label_examples/14_frontal_diaphragm.png}\\
         \midrule
         \multirow{3}{*}{\rotatebox{90}{Lateral}} & 
         \includegraphics[width=0.17\linewidth,height=0.17\linewidth]{images/supplementary_label_examples/15_lateral.png}&
         \includegraphics[width=0.17\linewidth,height=0.17\linewidth]{images/supplementary_label_examples/15_lateral_lung.png}&
         \includegraphics[width=0.17\linewidth,height=0.17\linewidth]{images/supplementary_label_examples/15_lateral_mediastinum.png}&
         \includegraphics[width=0.17\linewidth,height=0.17\linewidth]{images/supplementary_label_examples/15_lateral_bones.png}&
         \includegraphics[width=0.17\linewidth,height=0.17\linewidth]{images/supplementary_label_examples/15_lateral_diaphragm.png}\\

         & 
         \includegraphics[width=0.17\linewidth,height=0.17\linewidth]{images/supplementary_label_examples/14_lateral.png}&
         \includegraphics[width=0.17\linewidth,height=0.17\linewidth]{images/supplementary_label_examples/14_lateral_lung.png}&
         \includegraphics[width=0.17\linewidth,height=0.17\linewidth]{images/supplementary_label_examples/14_lateral_mediastinum.png}&
         \includegraphics[width=0.17\linewidth,height=0.17\linewidth]{images/supplementary_label_examples/14_lateral_bones.png}&
         \includegraphics[width=0.17\linewidth,height=0.17\linewidth]{images/supplementary_label_examples/14_lateral_diaphragm.png}\\
         \bottomrule
    \end{tabular}
    \caption{Qualitative results of a UNet with ResNet50 backbone trained on our PAX-ray dataset for multiple patients in OpenI.}
    \label{fig:supplementary_label_examples}
\end{figure*}
