# Supplementary material for: Detailed Annotations of Chest X-Rays via CT Projection for Report Understanding
Source: arXiv:2210.03416 source file (2022-10-07)
Supplement: Supplementary file 7 [file setup.tex]

\begin{figure}[h!]
    \centering
    \includegraphics[width=\linewidth]{images/Study_setup.png}
    \caption{Illustration of one question of the user study investigating the label quality of individual ribs.}
    \label{fig:study}
\end{figure}
