# Supplementary material for: Detailed Annotations of Chest X-Rays via CT Projection for Report Understanding
Source: arXiv:2210.03416 source file (2022-10-07)
Supplement: Supplementary file 8 [file syn_v_real.tex]

\setlength{\tabcolsep}{2pt}
\setlength{\abovecaptionskip}{6pt}
\setlength{\belowcaptionskip}{10pt}

\begin{figure}[h!]
    \centering
    \begin{tabular}{c ccc || ccc}
    \toprule
    & \multicolumn{3}{c}{OpenI (X-Ray)} & \multicolumn{3}{c}{PAXRay (Projected)} \\
    \midrule
    \multirow{3}{*}{\rotatebox{90}{Frontal}} & \includegraphics[width=0.15\linewidth,height=0.15\linewidth]{images/supplementary/real/CXR27_IM-1168-2002.png}& \includegraphics[width=0.15\linewidth,height=0.15\linewidth]{images/supplementary/real/CXR28_IM-1231-1001.png}& \includegraphics[width=0.15\linewidth,height=0.15\linewidth]{images/supplementary/real/CXR29_IM-1302-1001.png}& 
    \includegraphics[width=0.15\linewidth,height=0.15\linewidth]{images/supplementary/synthethic/RibFrac21frontal.png}& \includegraphics[width=0.15\linewidth,height=0.15\linewidth]{images/supplementary/synthethic/RibFrac22frontal.png}& \includegraphics[width=0.15\linewidth,height=0.15\linewidth]{images/supplementary/synthethic/RibFrac23frontal.png} \\
    & \includegraphics[width=0.15\linewidth,height=0.15\linewidth]{images/supplementary/real/CXR30_IM-1385-1001.png}& \includegraphics[width=0.15\linewidth,height=0.15\linewidth]{images/supplementary/real/CXR31_IM-1450-1001.png}& \includegraphics[width=0.15\linewidth,height=0.15\linewidth]{images/supplementary/real/CXR32_IM-1511-1001.png}& 
    \includegraphics[width=0.15\linewidth,height=0.15\linewidth]{images/supplementary/synthethic/RibFrac24frontal.png}& \includegraphics[width=0.15\linewidth,height=0.15\linewidth]{images/supplementary/synthethic/RibFrac25frontal.png}& \includegraphics[width=0.15\linewidth,height=0.15\linewidth]{images/supplementary/synthethic/RibFrac26frontal.png}\\
    & \includegraphics[width=0.15\linewidth,height=0.15\linewidth]{images/supplementary/real/CXR33_IM-1576-13013.png}& \includegraphics[width=0.15\linewidth,height=0.15\linewidth]{images/supplementary/real/CXR34_IM-1644-1001.png}& \includegraphics[width=0.15\linewidth,height=0.15\linewidth]{images/supplementary/real/CXR2_IM-0652-1001.png}& 
    \includegraphics[width=0.15\linewidth,height=0.15\linewidth]{images/supplementary/synthethic/RibFrac27frontal.png}& \includegraphics[width=0.15\linewidth,height=0.15\linewidth]{images/supplementary/synthethic/RibFrac28frontal.png}& \includegraphics[width=0.15\linewidth,height=0.15\linewidth]{images/supplementary/synthethic/RibFrac29frontal.png}\\\midrule\midrule
    \multirow{3}{*}{\rotatebox{90}{Lateral}}& \includegraphics[width=0.15\linewidth,height=0.15\linewidth]{images/supplementary/real/CXR27_IM-1168-3003.png}& \includegraphics[width=0.15\linewidth,height=0.15\linewidth]{images/supplementary/real/CXR29_IM-1302-2001.png}& \includegraphics[width=0.15\linewidth,height=0.15\linewidth]{images/supplementary/real/CXR28_IM-1231-2001.png}& 
    \includegraphics[width=0.15\linewidth,height=0.15\linewidth]{images/supplementary/synthethic/RibFrac21lateral.png}& \includegraphics[width=0.15\linewidth,height=0.15\linewidth]{images/supplementary/synthethic/RibFrac22lateral.png}& \includegraphics[width=0.15\linewidth,height=0.15\linewidth]{images/supplementary/synthethic/RibFrac23lateral.png} \\
    & \includegraphics[width=0.15\linewidth,height=0.15\linewidth]{images/supplementary/real/CXR30_IM-1385-2001.png}& \includegraphics[width=0.15\linewidth,height=0.15\linewidth]{images/supplementary/real/CXR31_IM-1450-3003.png}& \includegraphics[width=0.15\linewidth,height=0.15\linewidth]{images/supplementary/real/CXR32_IM-1511-4001.png}& 
    \includegraphics[width=0.15\linewidth,height=0.15\linewidth]{images/supplementary/synthethic/RibFrac24lateral.png}& \includegraphics[width=0.15\linewidth,height=0.15\linewidth]{images/supplementary/synthethic/RibFrac25lateral.png}& \includegraphics[width=0.15\linewidth,height=0.15\linewidth]{images/supplementary/synthethic/RibFrac26lateral.png}\\
    & \includegraphics[width=0.15\linewidth,height=0.15\linewidth]{images/supplementary/real/CXR33_IM-1576-12012.png}& \includegraphics[width=0.15\linewidth,height=0.15\linewidth]{images/supplementary/real/CXR34_IM-1644-2001.png}& \includegraphics[width=0.15\linewidth,height=0.15\linewidth]{images/supplementary/real/CXR2_IM-0652-2001.png}& 
    \includegraphics[width=0.15\linewidth,height=0.15\linewidth]{images/supplementary/synthethic/RibFrac27lateral.png}& \includegraphics[width=0.15\linewidth,height=0.15\linewidth]{images/supplementary/synthethic/RibFrac28lateral.png}& \includegraphics[width=0.15\linewidth,height=0.15\linewidth]{images/supplementary/synthethic/RibFrac29lateral.png}\\
    \bottomrule
    \end{tabular}
    \caption{Comparison of different real and projected samples for the frontal and lateral view}
    \label{fig:syn_real}
\end{figure}
