# Supplementary material for: Detailed Annotations of Chest X-Rays via CT Projection for Report Understanding
Source: arXiv:2210.03416 source file (2022-10-07)
Supplement: Supplementary file 9 [file userstudy.tex]

\begin{table*}[h!]
% \tiny
        \caption{Inter-annotator agreement in the form of Fleiss' $\kappa$ and the mean and standard deviation of the annotator-pairwise Spearman correlation coefficient of the user study for label evaluation}
    \centering
    \begin{tabular}{cccccc}
    \toprule
        \multicolumn{6}{c}{Frontal}\\
        \hline
        &Lobes & Vessels & Sub-Diaphragm & Ribs & Spine\\
        Fleiss $\kappa$ &-0.076 & -0.099 & -0.195 & -0.172 & -0.188\\
        Spearman & $0.10 \pm 0.27$ & $0.03 \pm 039$ & $0.26 \pm 0.23$ & $-0.21 \pm 0.22 $& $0.25\pm0.29$
        \\
        
        \hline
        &Mediastinal Regions & Heart & Airways& Esophagus & Aorta  \\
        Fleiss $\kappa$ &-0.045 & -0.13 & 0.027 & -0.001 & 0.05
        \\Spearman & $0.36 \pm 0.23$ & $0.73 \pm 0.19$ & $0.07 \pm 0.44$ & $0.45\pm0.15$ & $0.62\pm0.09$ 
        \\
        \midrule
        \multicolumn{6}{c}{Lateral}\\
        \hline
        &Lungs & Vessels & Sub-Diaphragm & Ribs & Spine\\
        Fleiss $\kappa$ &-0.114 & -0.017 & -0.187 & -0.115 & -0.072\\Spearman & $0.14 \pm 0.22$& $0.08 \pm 0.28$ & $0.09 \pm 0.37$ & $0.55 \pm 0.13 $& $0.55 \pm 0.09 $\\
        
        \hline
        &Mediastinal Regions & Heart & Airways& Esophagus & Aorta  \\
        Fleiss $\kappa$ &0.013 & -0.12 & 0.033 & -0.103 & -0.074\\
        Spearman & $0.27\pm 0.27 $& $0.35  \pm 0.15 $& $0.09 \pm 0.17$ & $0.43 \pm 0.26$ & $-0.07 \pm 0.39 $\\
        \bottomrule
    \end{tabular}

    \label{tab:agreement}
\end{table*}
